# Supplementary material for: Electricity Price Forecasting using Sale and Purchase Curves: The X-Model
Source: arXiv:1509.00372 ancillary file (2016-08-17)
Supplement: Supplementary file 1 [file appendix_time_series.pdf]

# Appendix 3: Electricity Price Forecasting using Sale and Purchase Curves: The X-Model

Florian Ziel (ziel@europa-uni.de), Rick Steinert (steinert@europa-uni.de)
Europa-Universität Viadrina, Große Scharrnstraße 59, 15230 Frankfurt (Oder), Germany

July 25, 2016

## Appendix

Time series plots for the X-Model of the full time range:

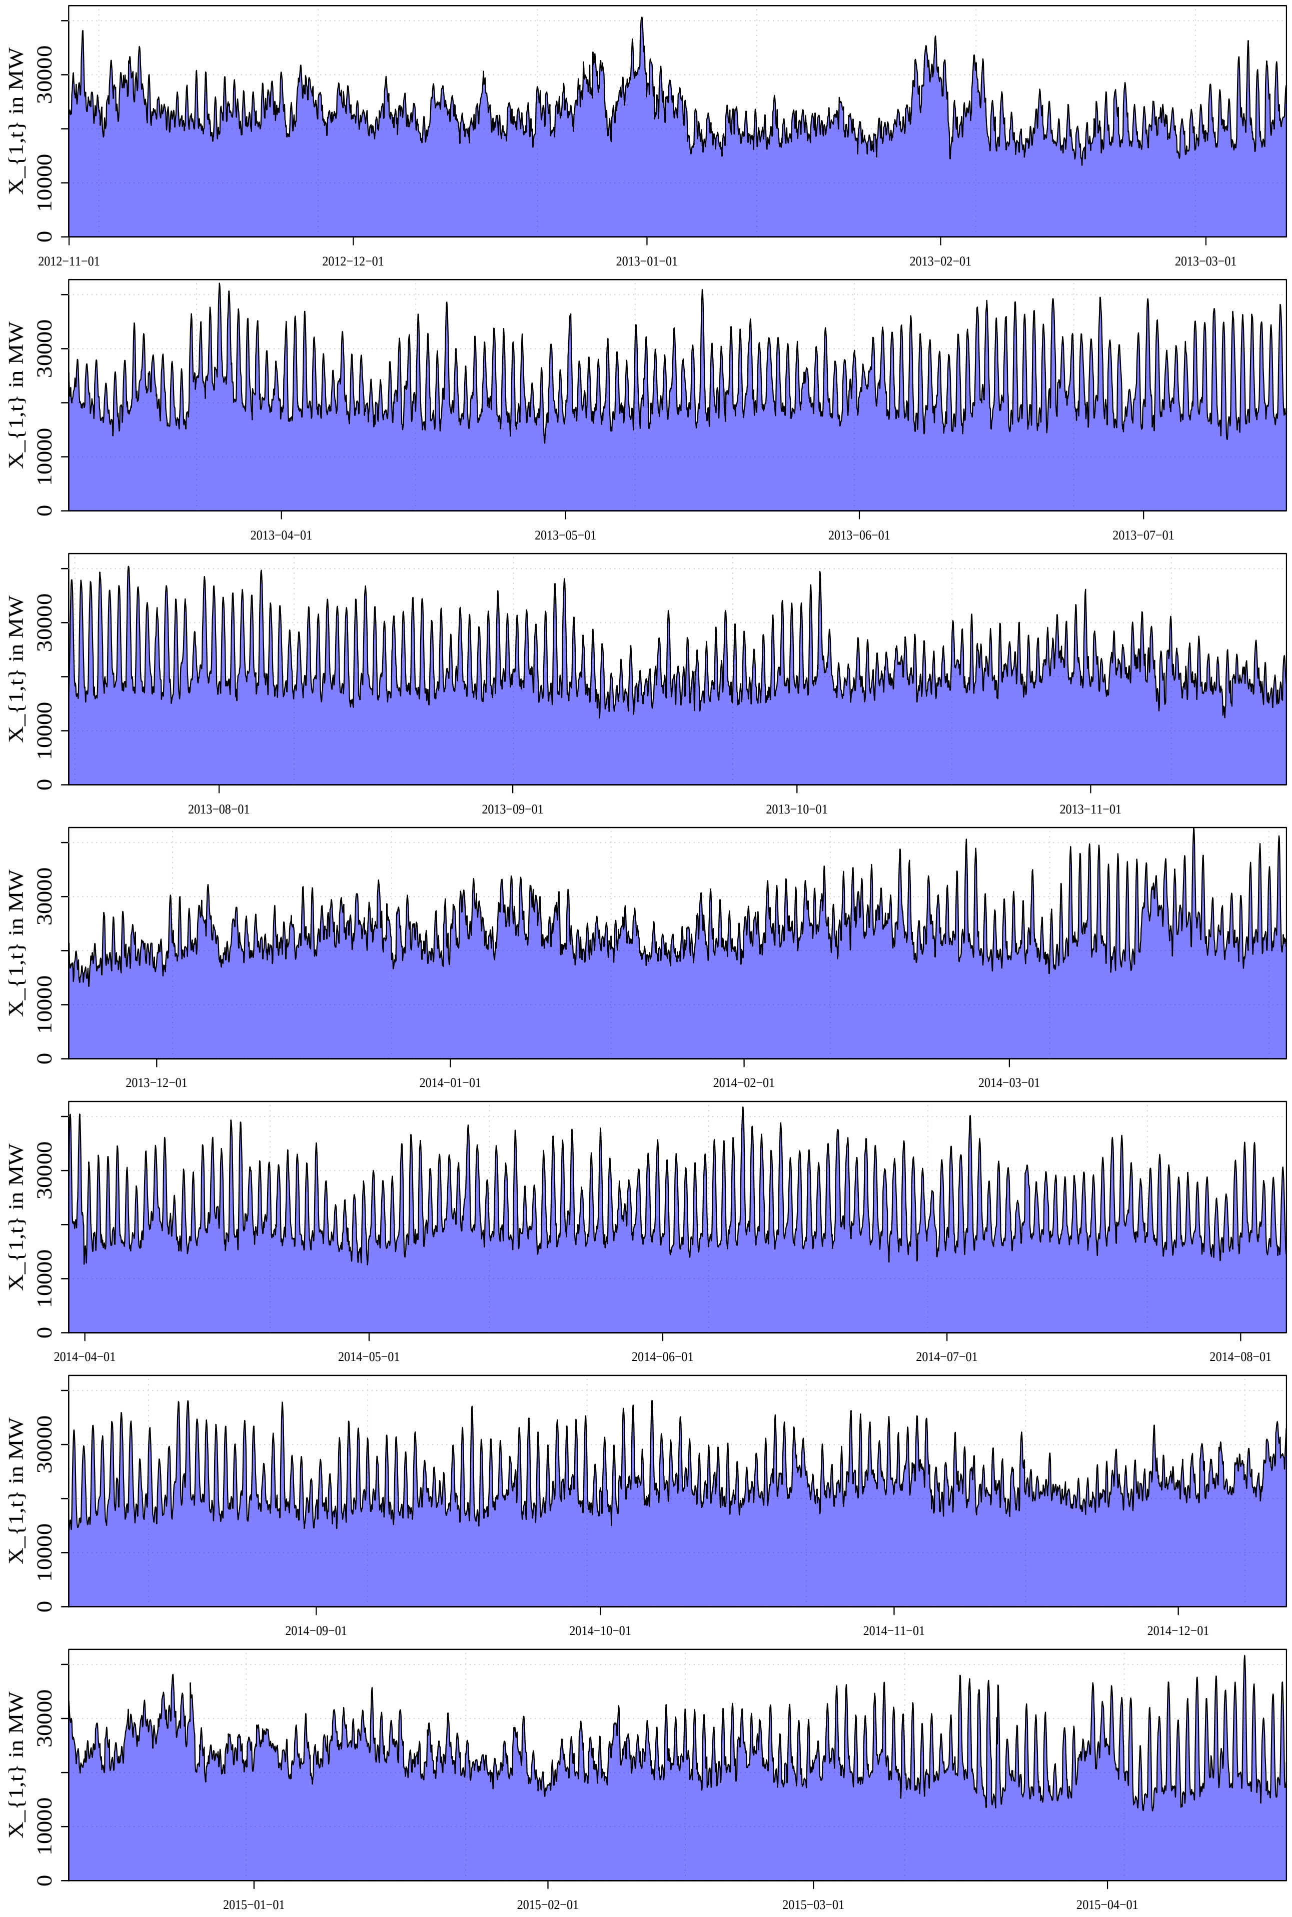


Figure 1: Time series plot of $X_{1,t} = X_{S,t}^{(-500)}$ with supply/sale bids on exactly $-500$

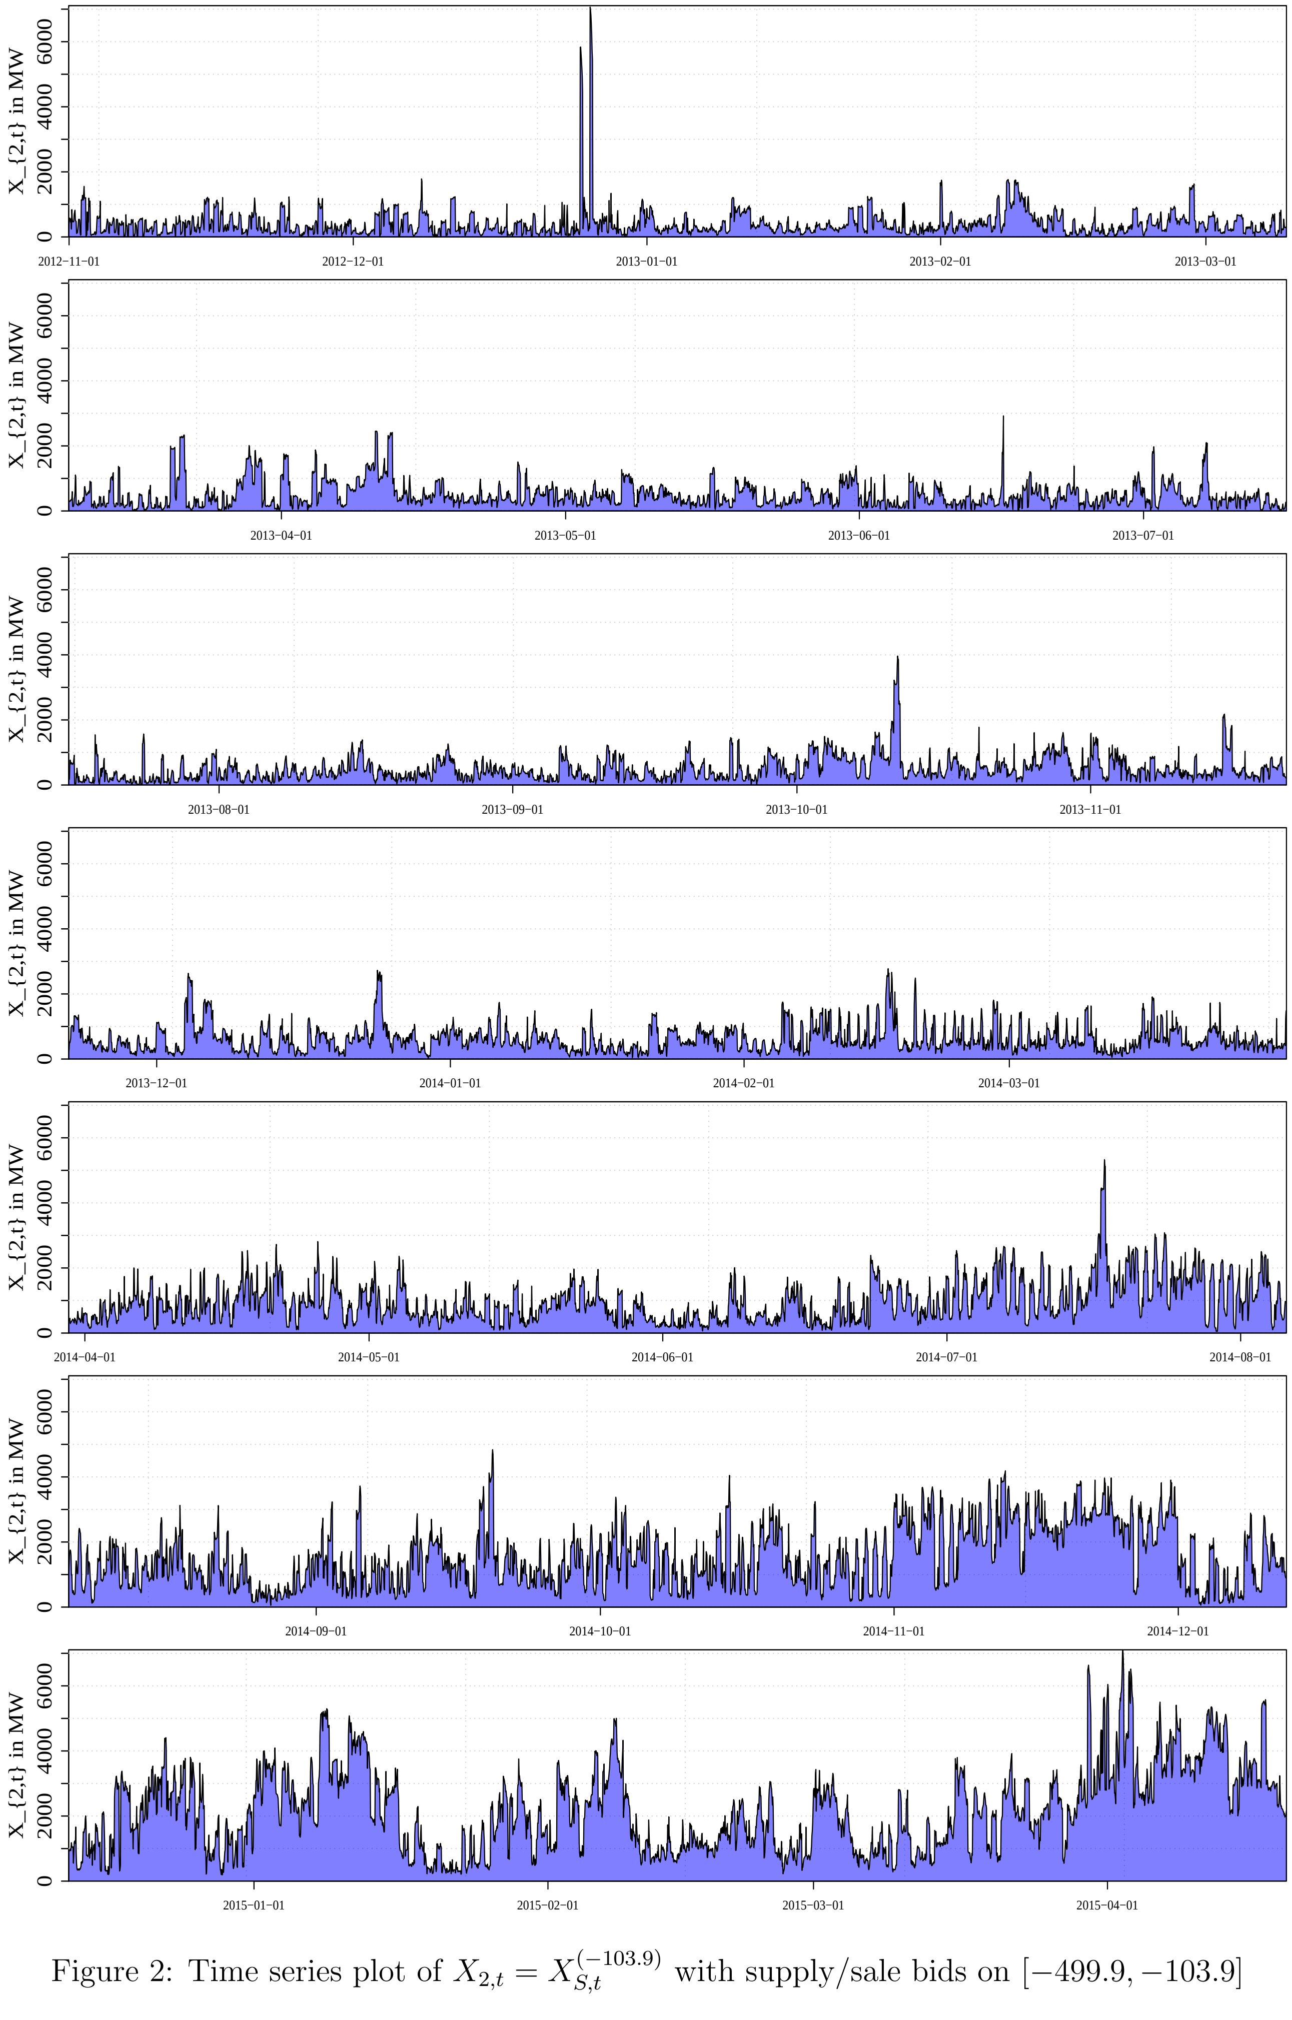


Figure 2: Time series plot of $X_{2,t} = X_{S,t}^{(-103.9)}$ with supply/sale bids on $[-499.9, -103.9]$

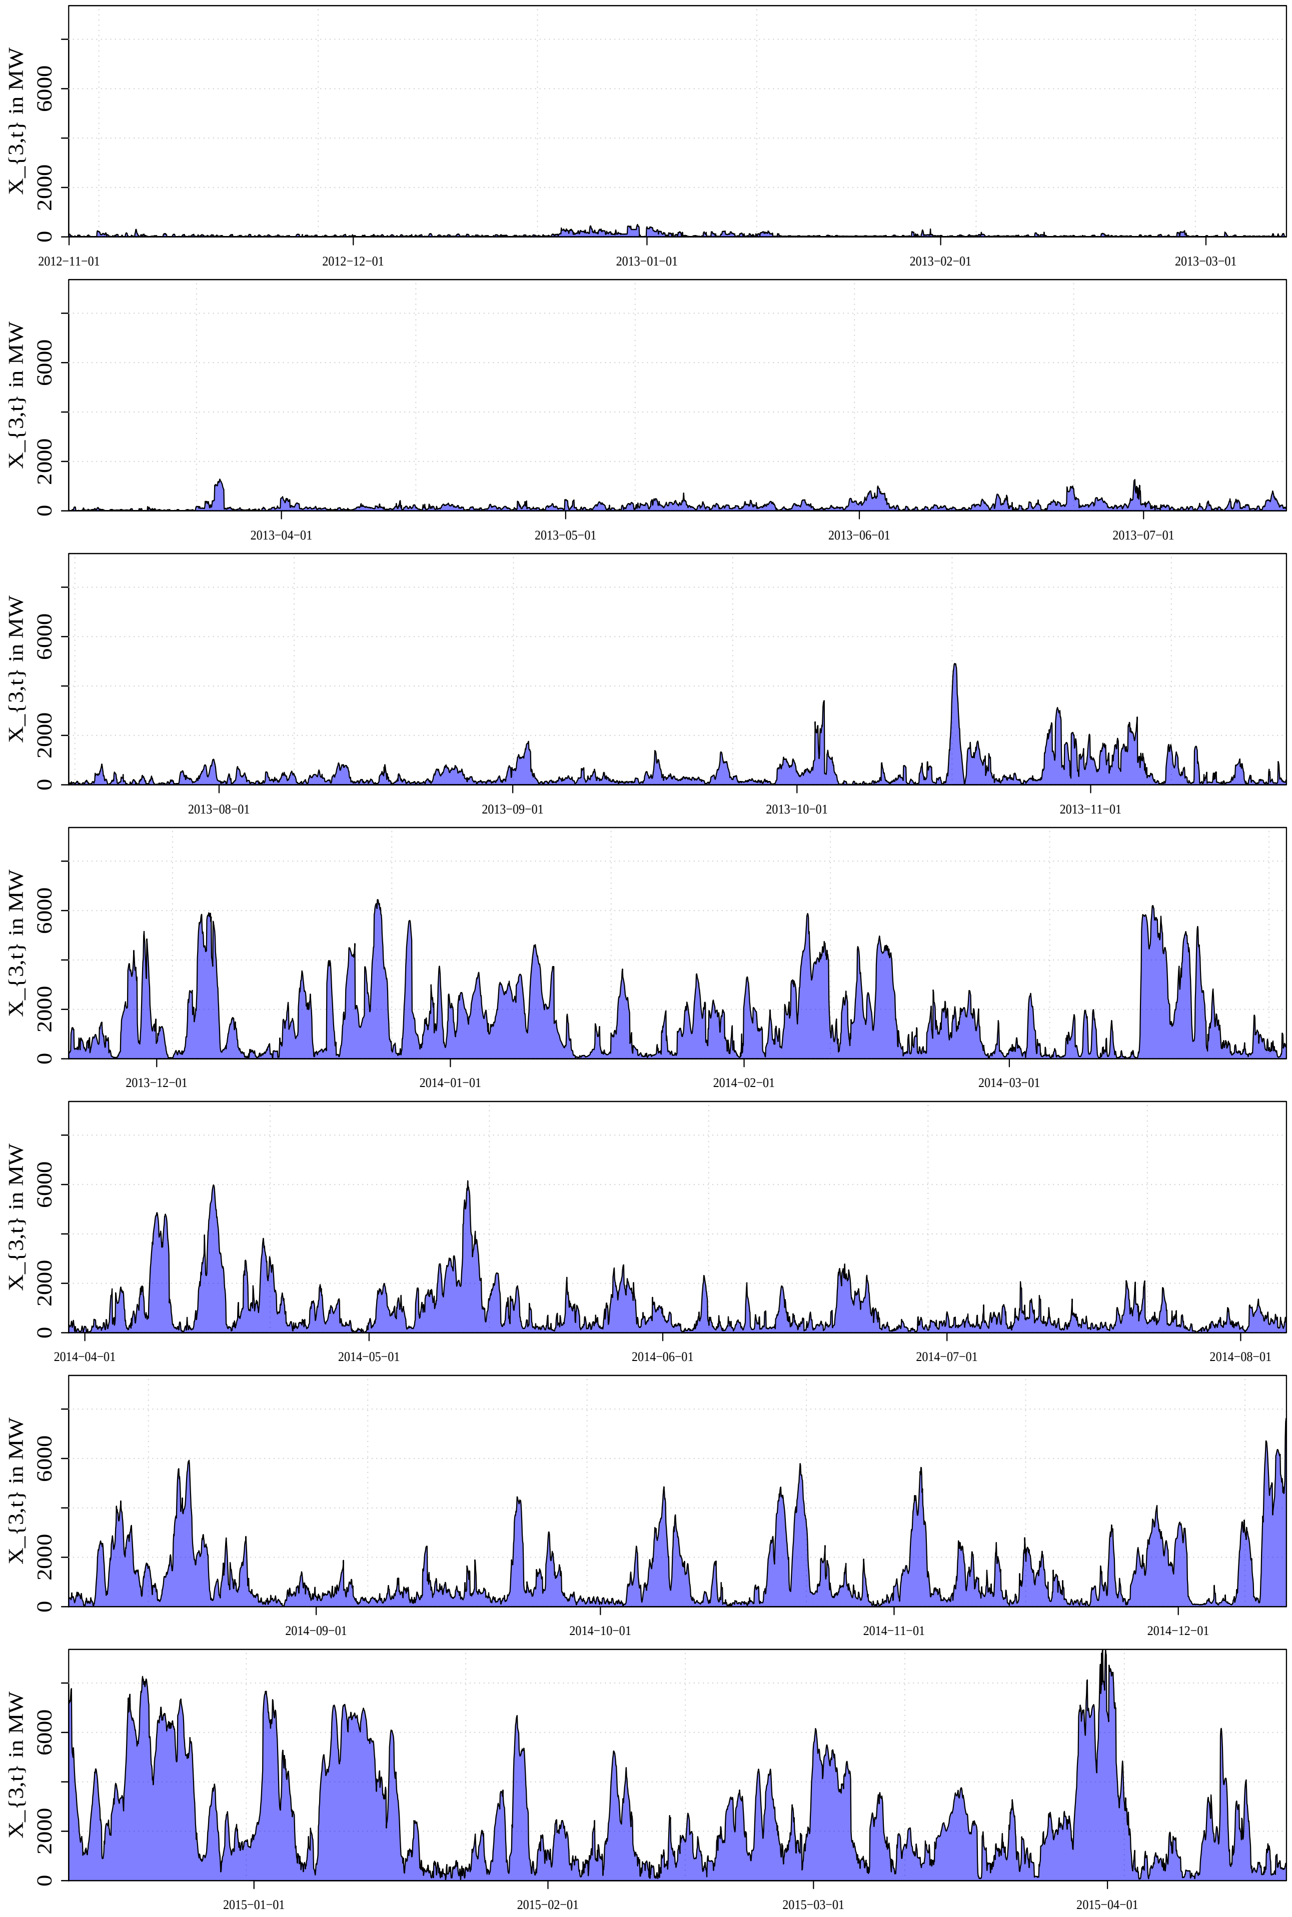


Figure 3: Time series plot of $X_{3,t} = X_{S,t}^{(-55.1)}$ with supply/sale bids on $[-103.8, -55.1]$

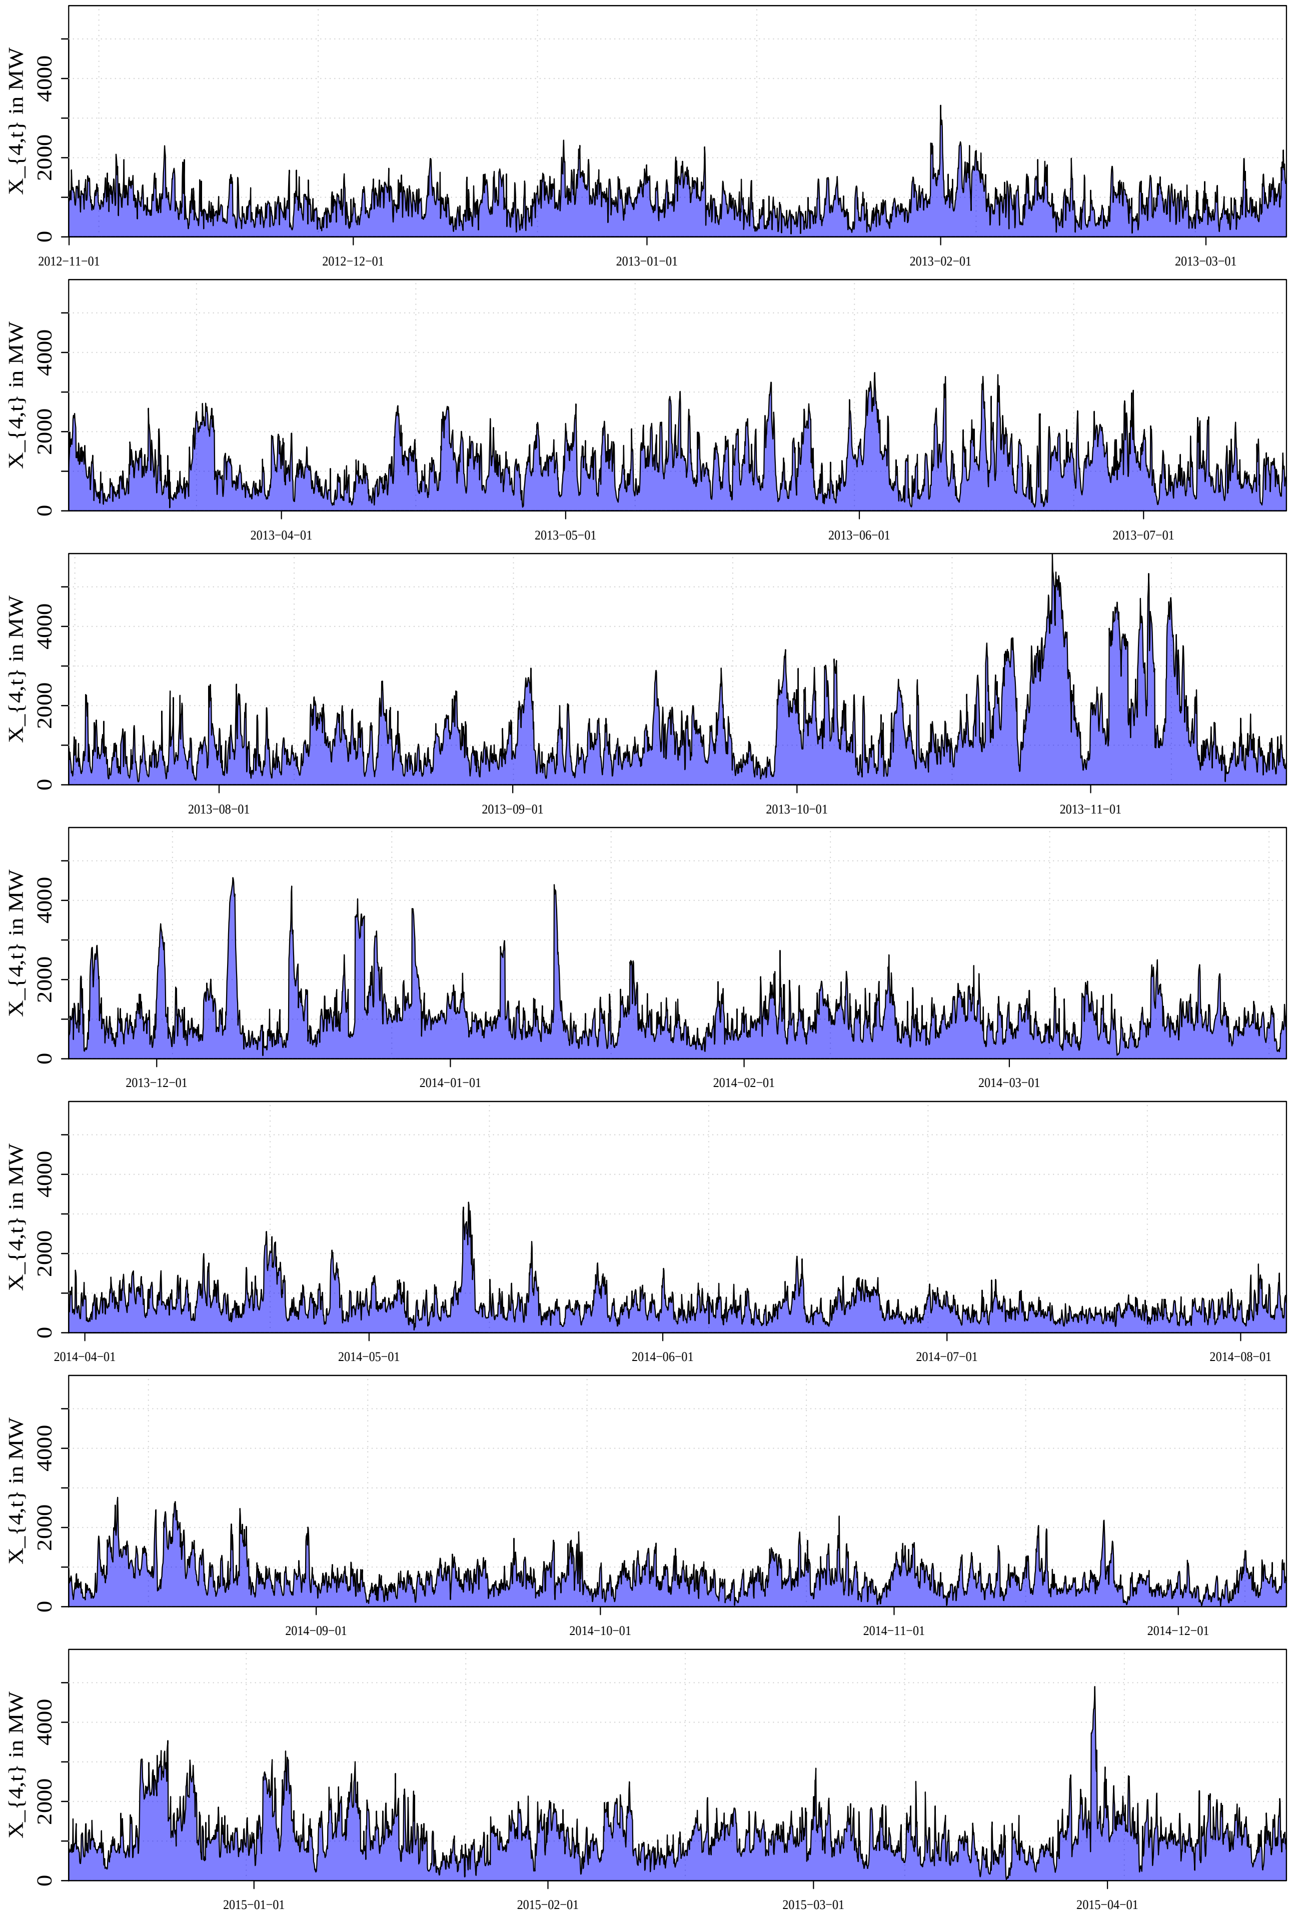


Figure 4: Time series plot of $X_{4,t} = X_{S,t}^{(1.3)}$ with supply/sale bids on $[-55.0, 1.3]$

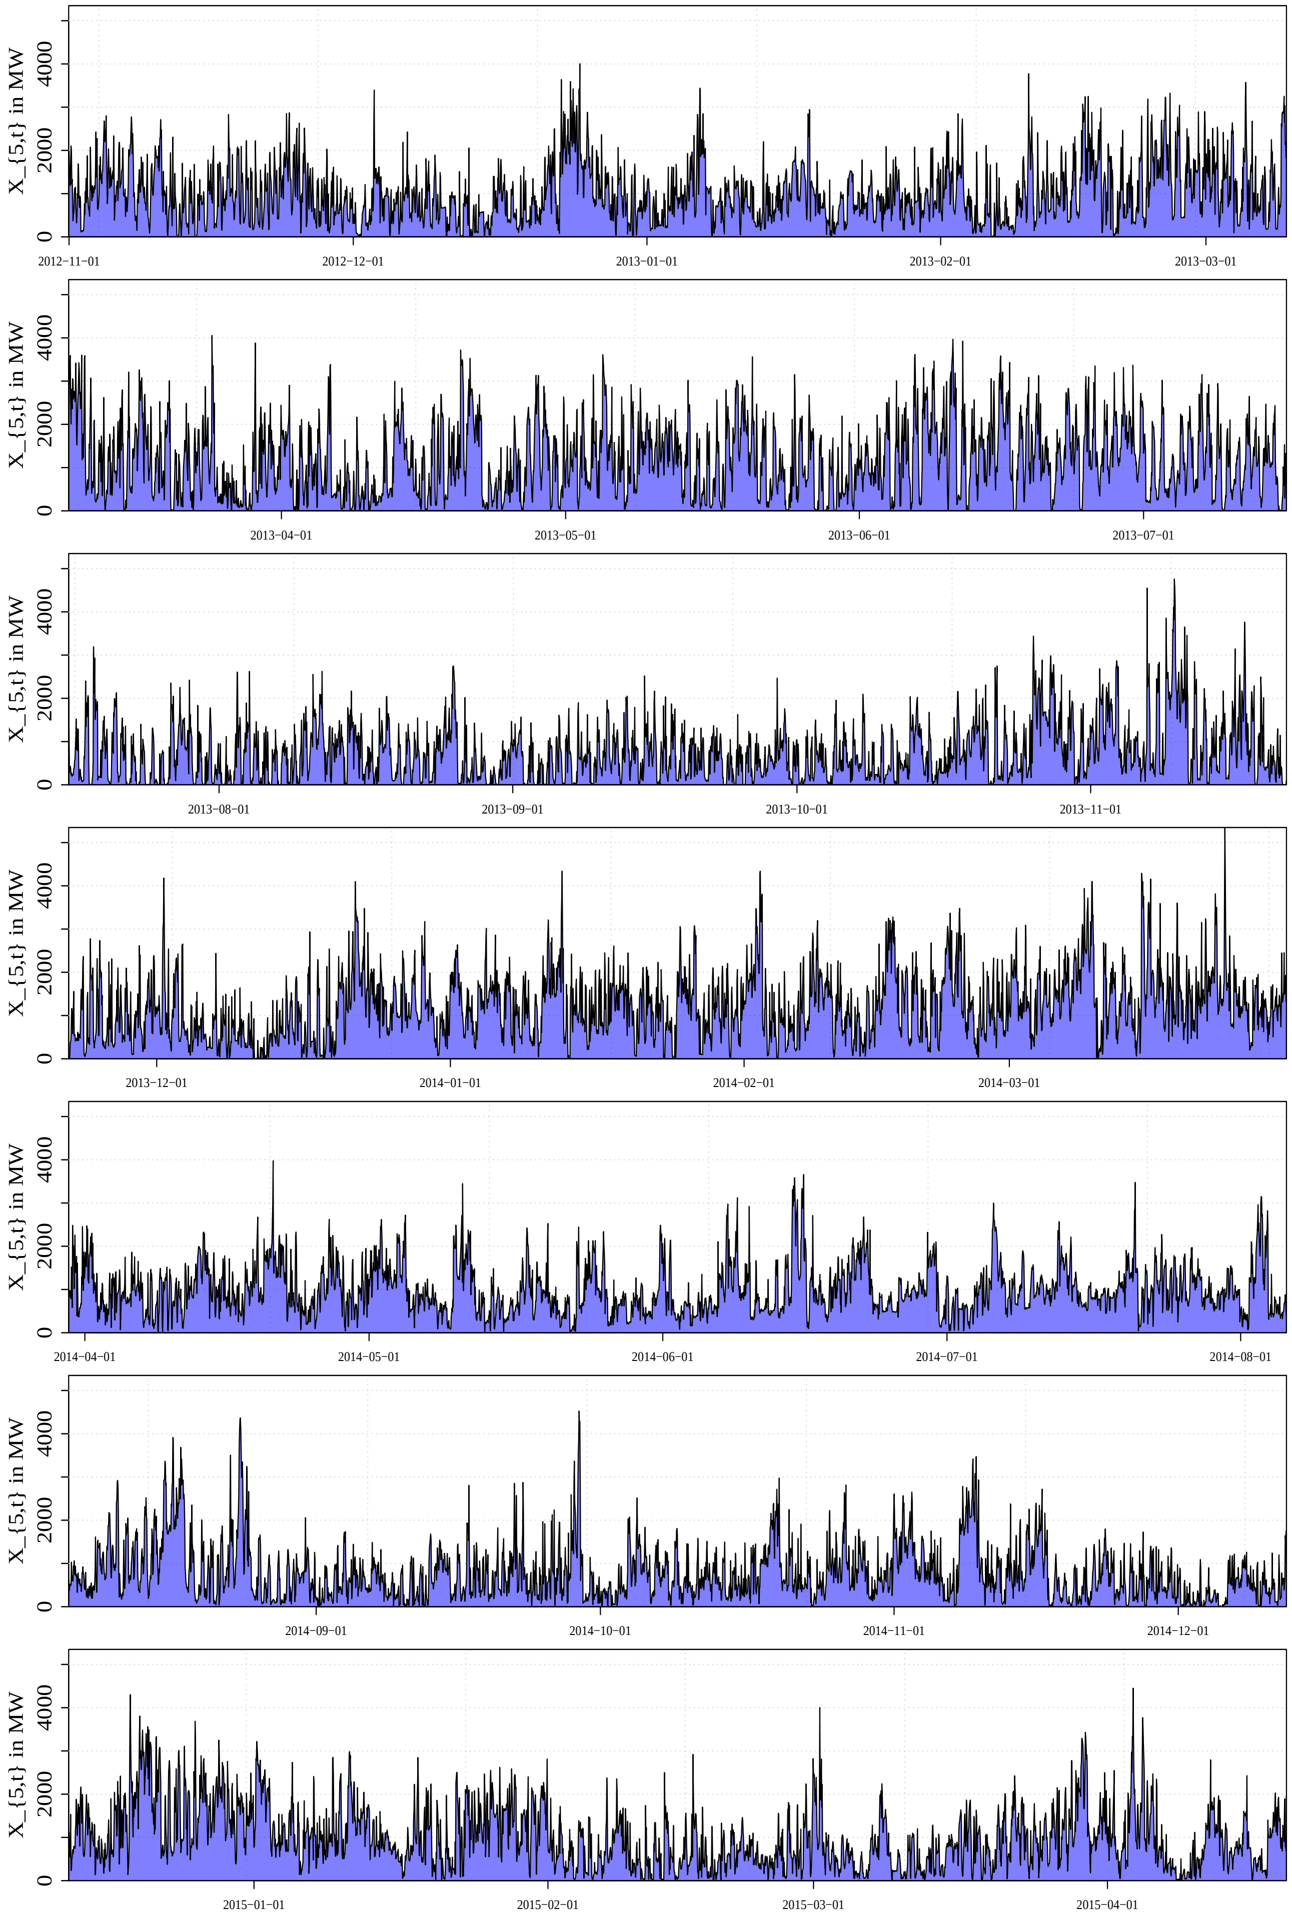


Figure 5: Time series plot of $X_{5,t} = X_{S,t}^{(19.5)}$ with supply/sale bids on $[1.4, 19.5]$

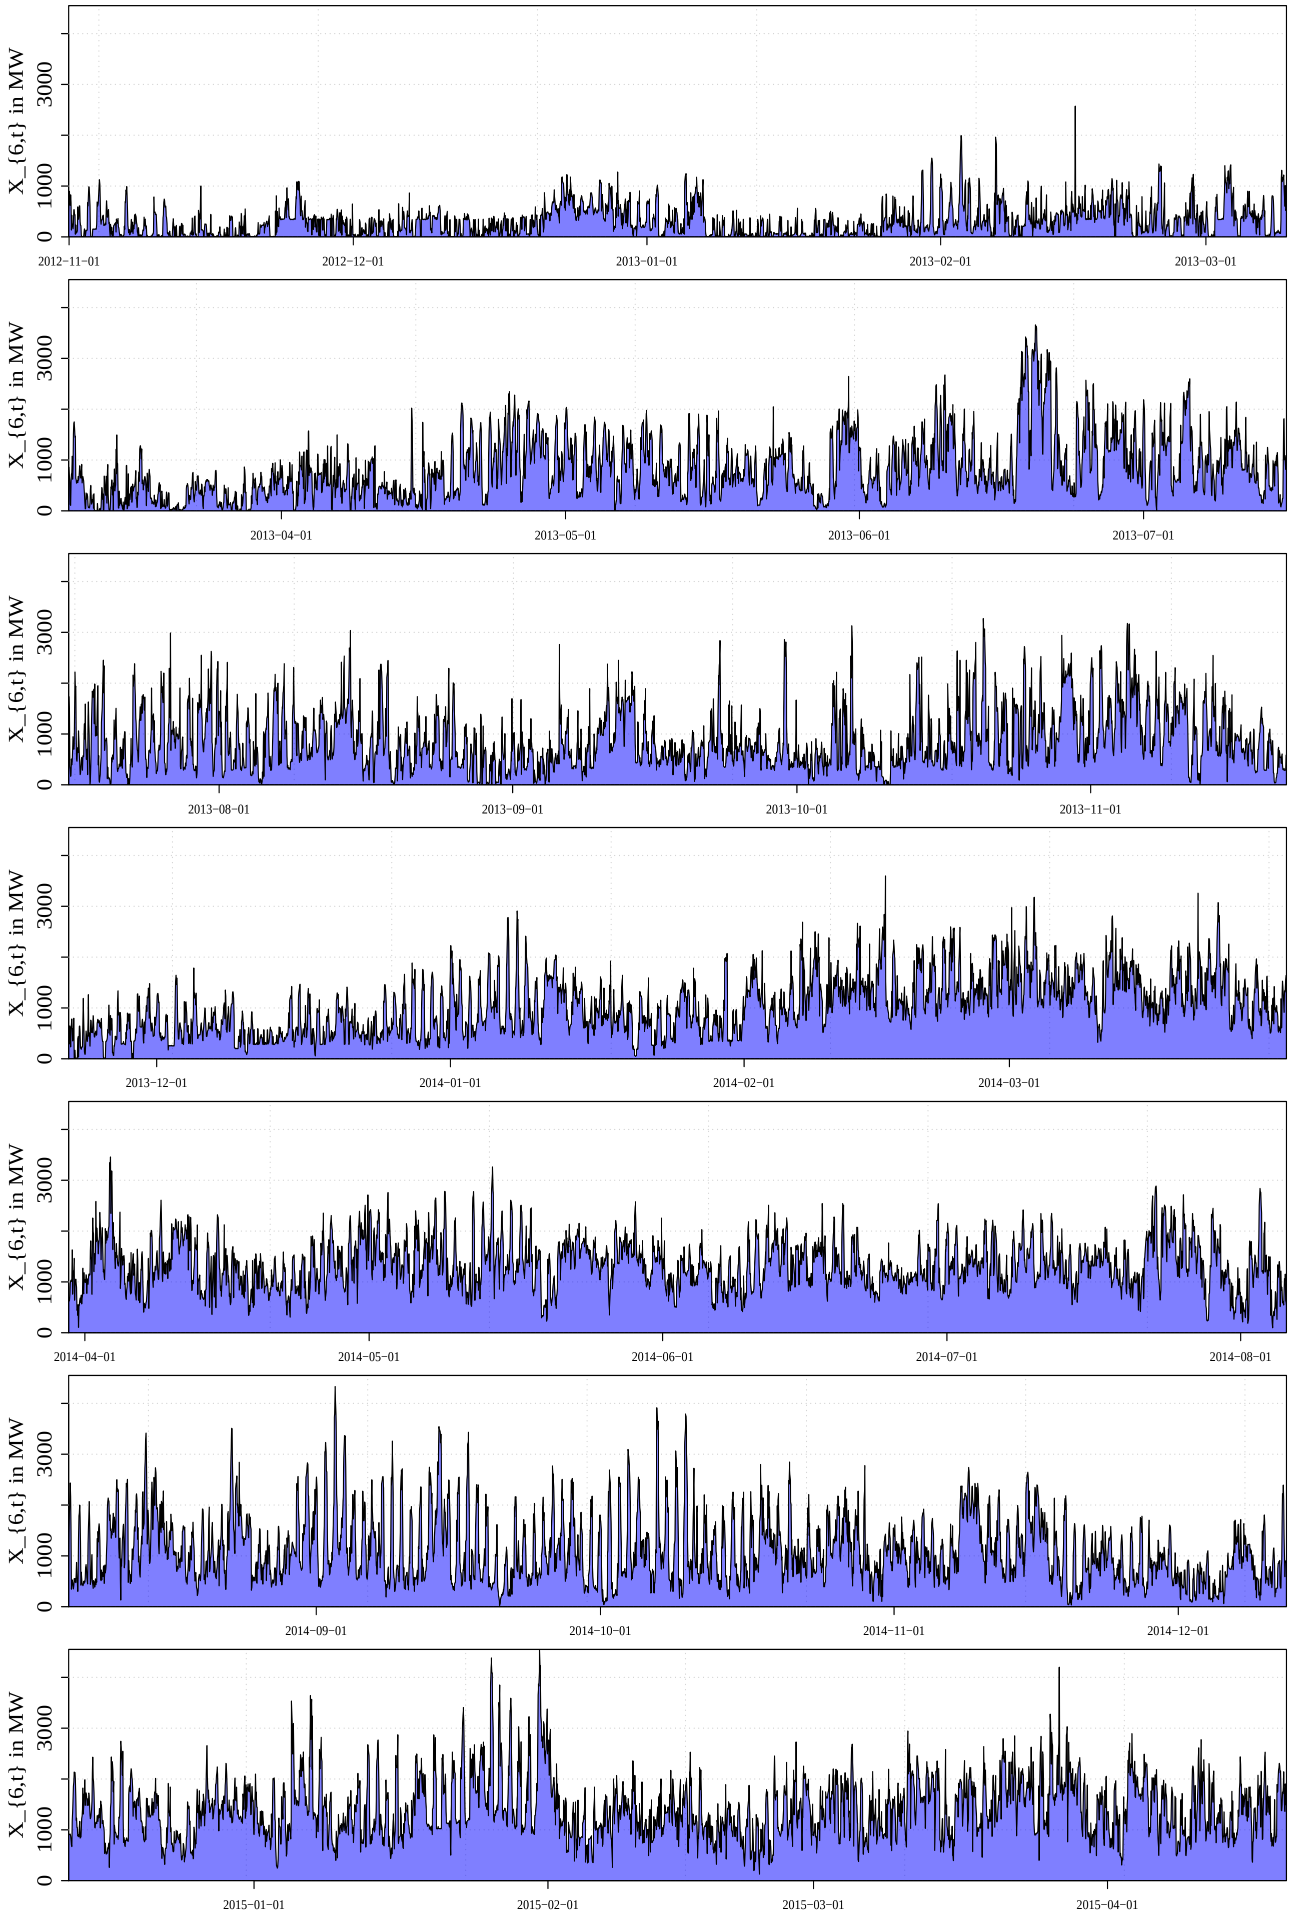


Figure 6: Time series plot of $X_{6,t} = X_{S,t}^{(27.5)}$ with supply/sale bids on $[19.6, 27.5]$

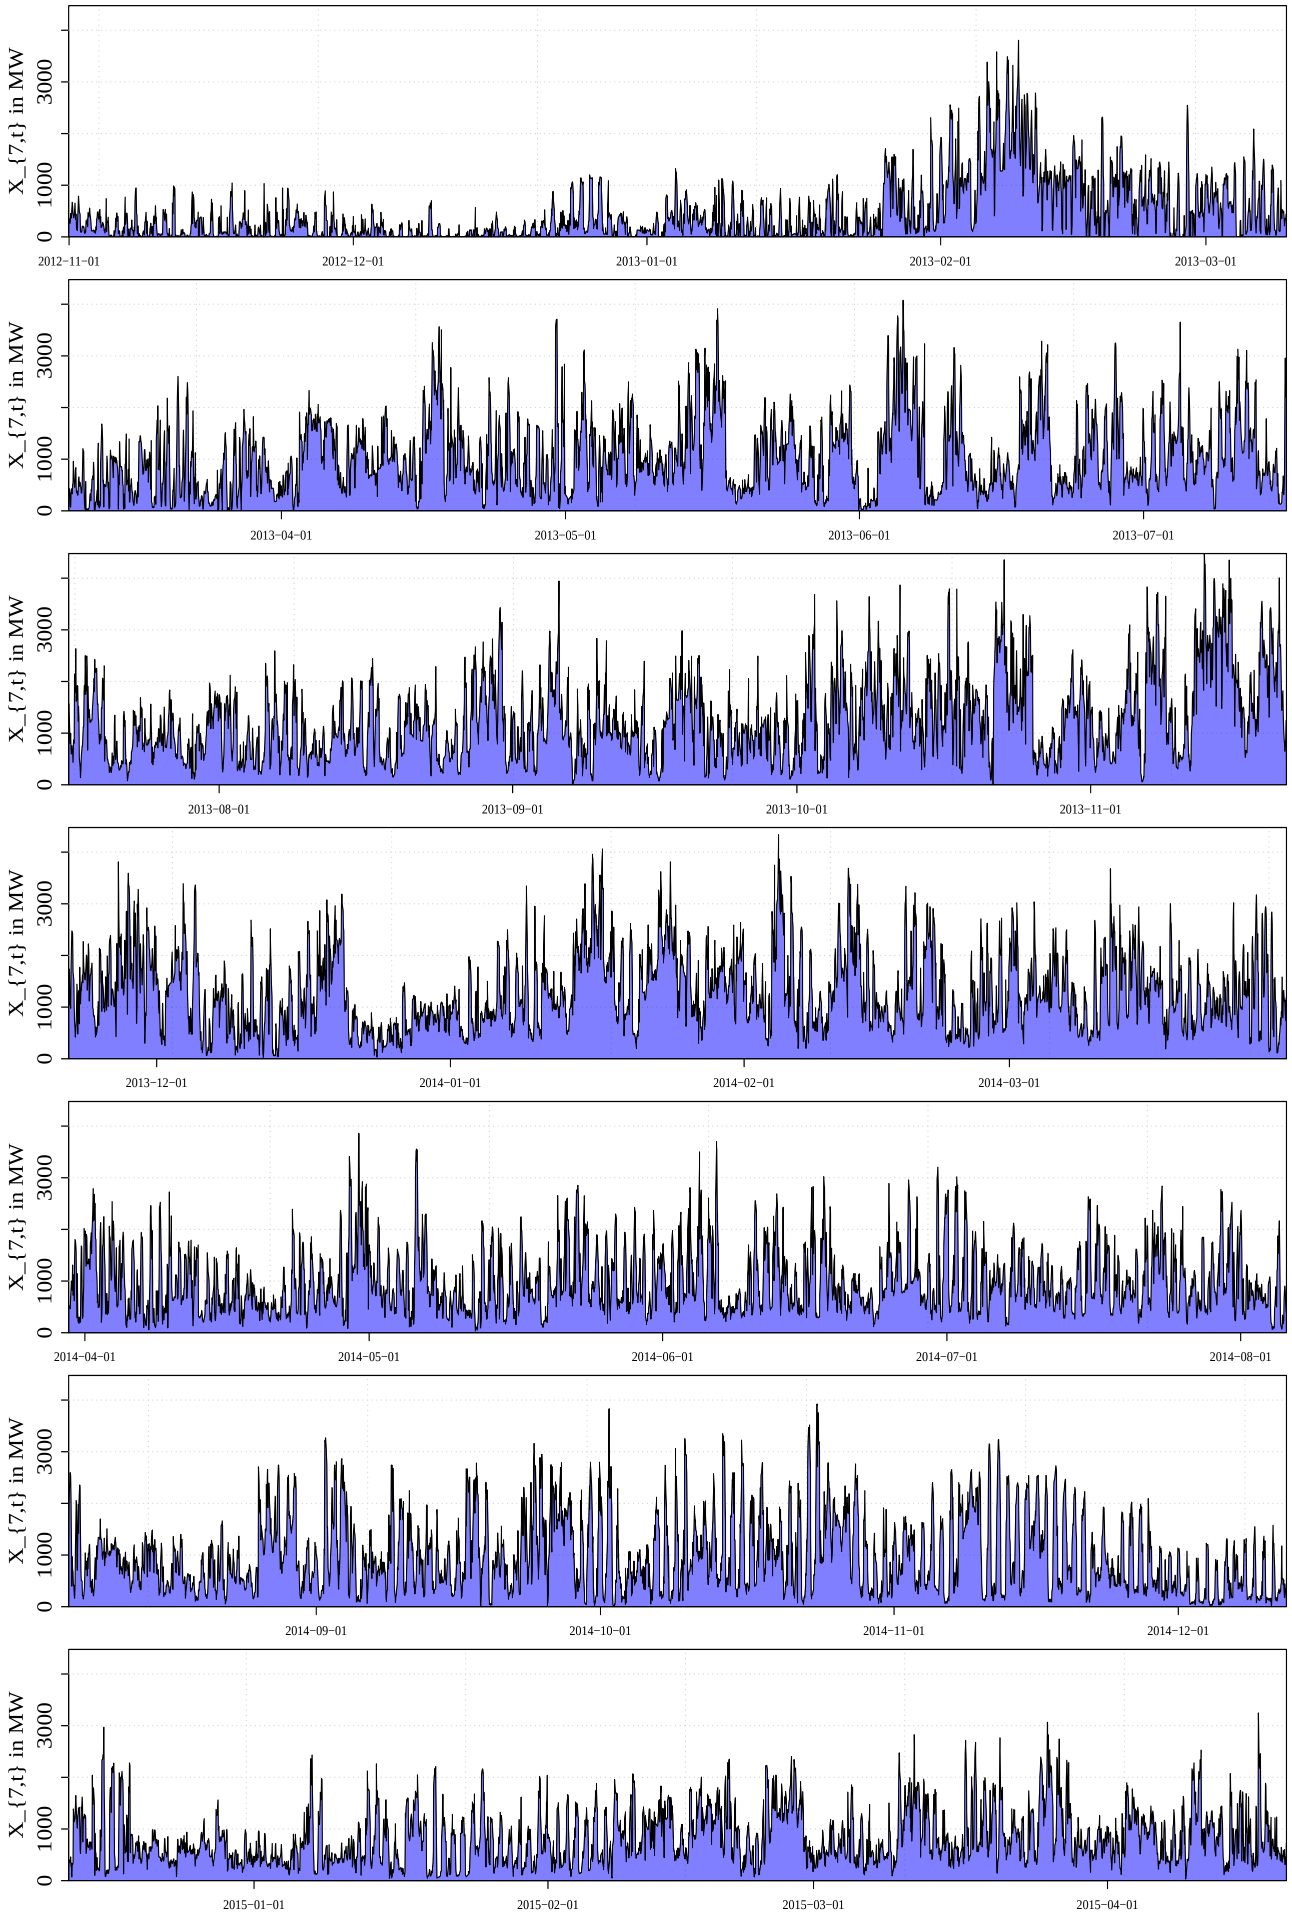


Figure 7: Time series plot of $X_{7,t} = X_{S,t}^{(31.3)}$ with supply/sale bids on $[27.6, 31.3]$

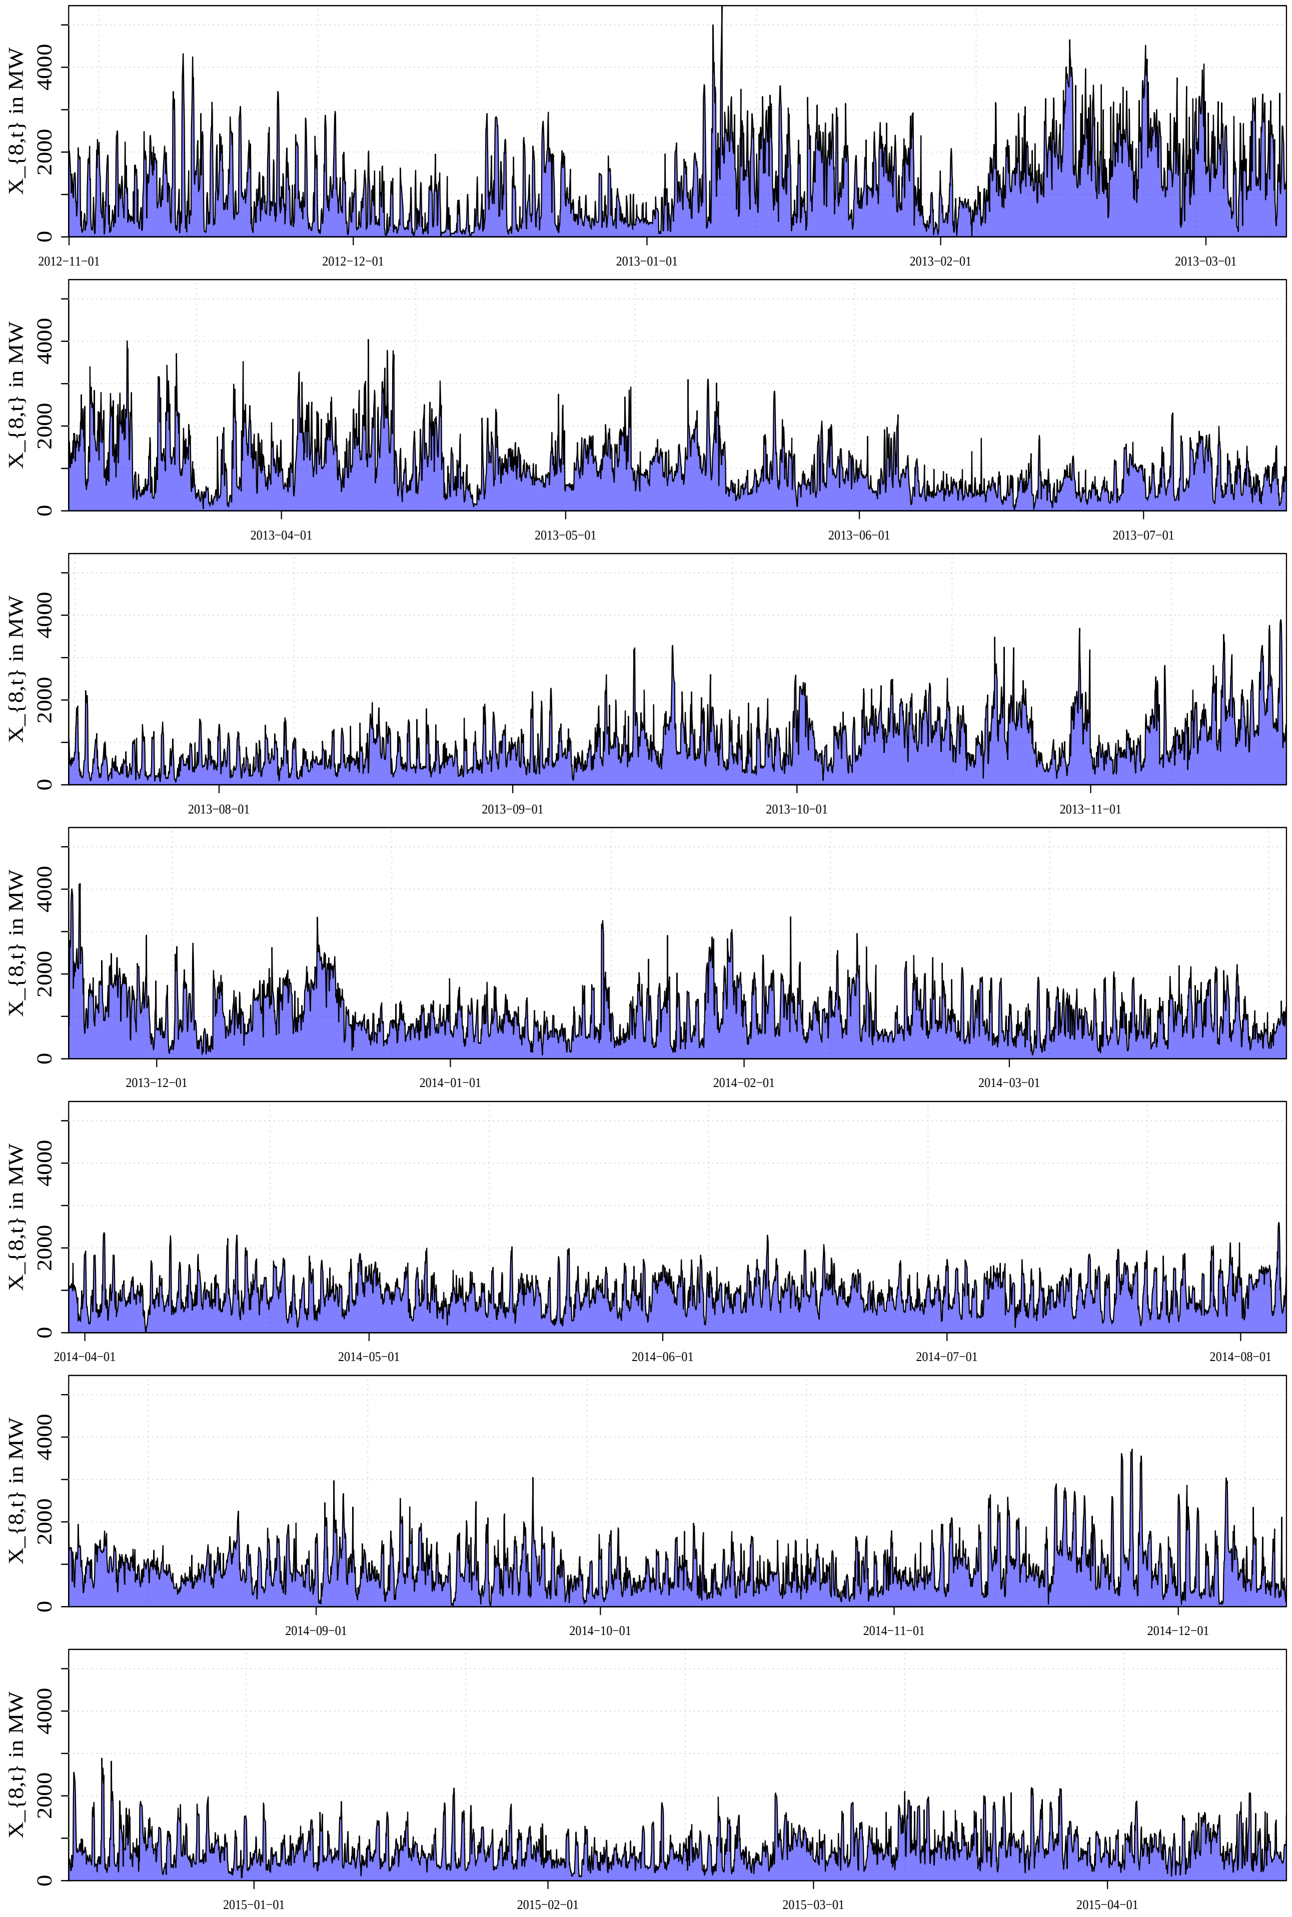


Figure 8: Time series plot of $X_{8,t} = X_{S,t}^{(36.2)}$ with supply/sale bids on $[31.4, 36.2]$

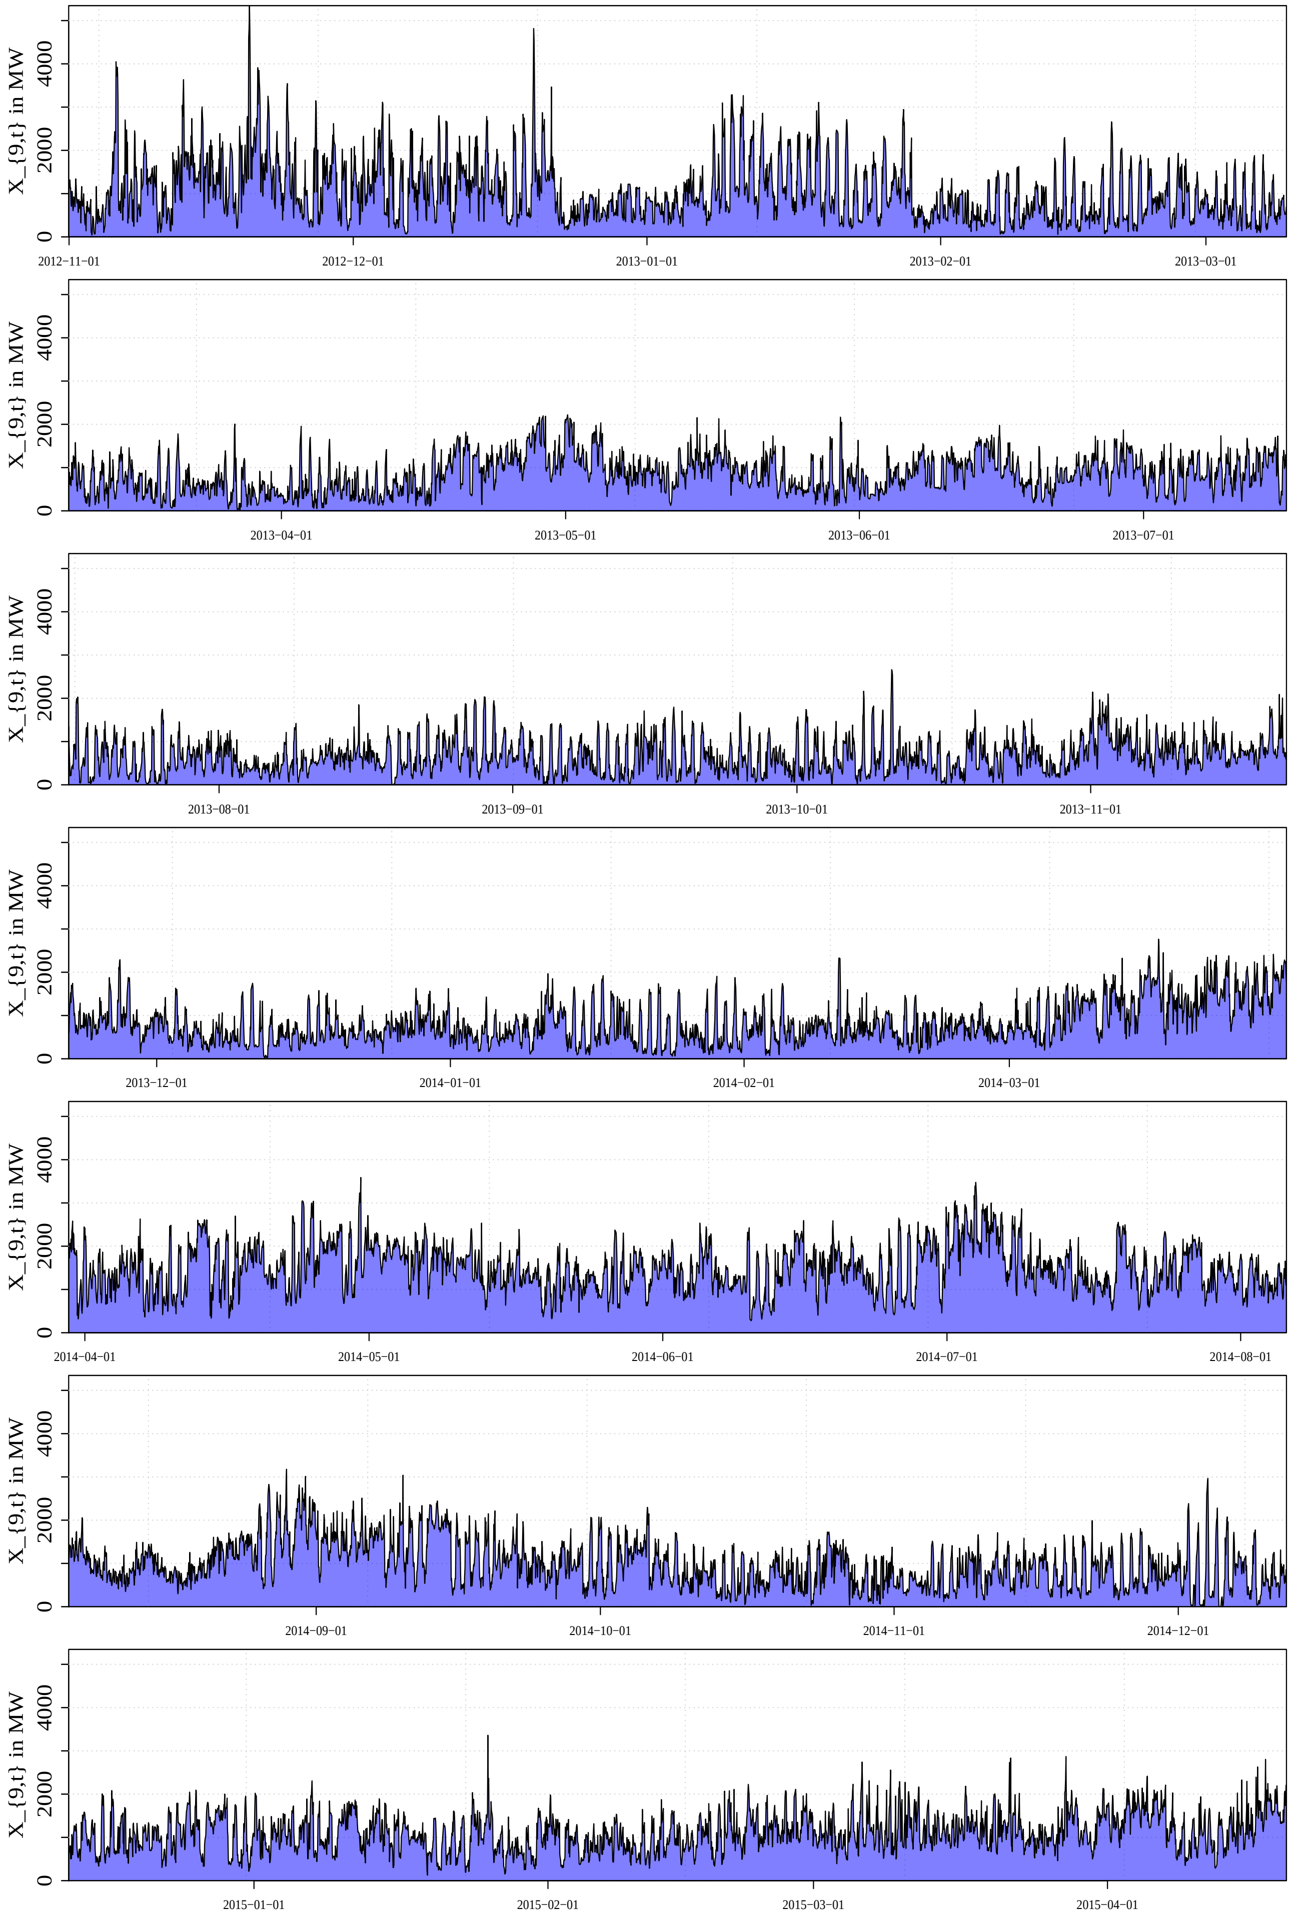


Figure 9: Time series plot of $X_{9,t} = X_{S,t}^{(42.4)}$ with supply/sale bids on $[36.3, 42.4]$

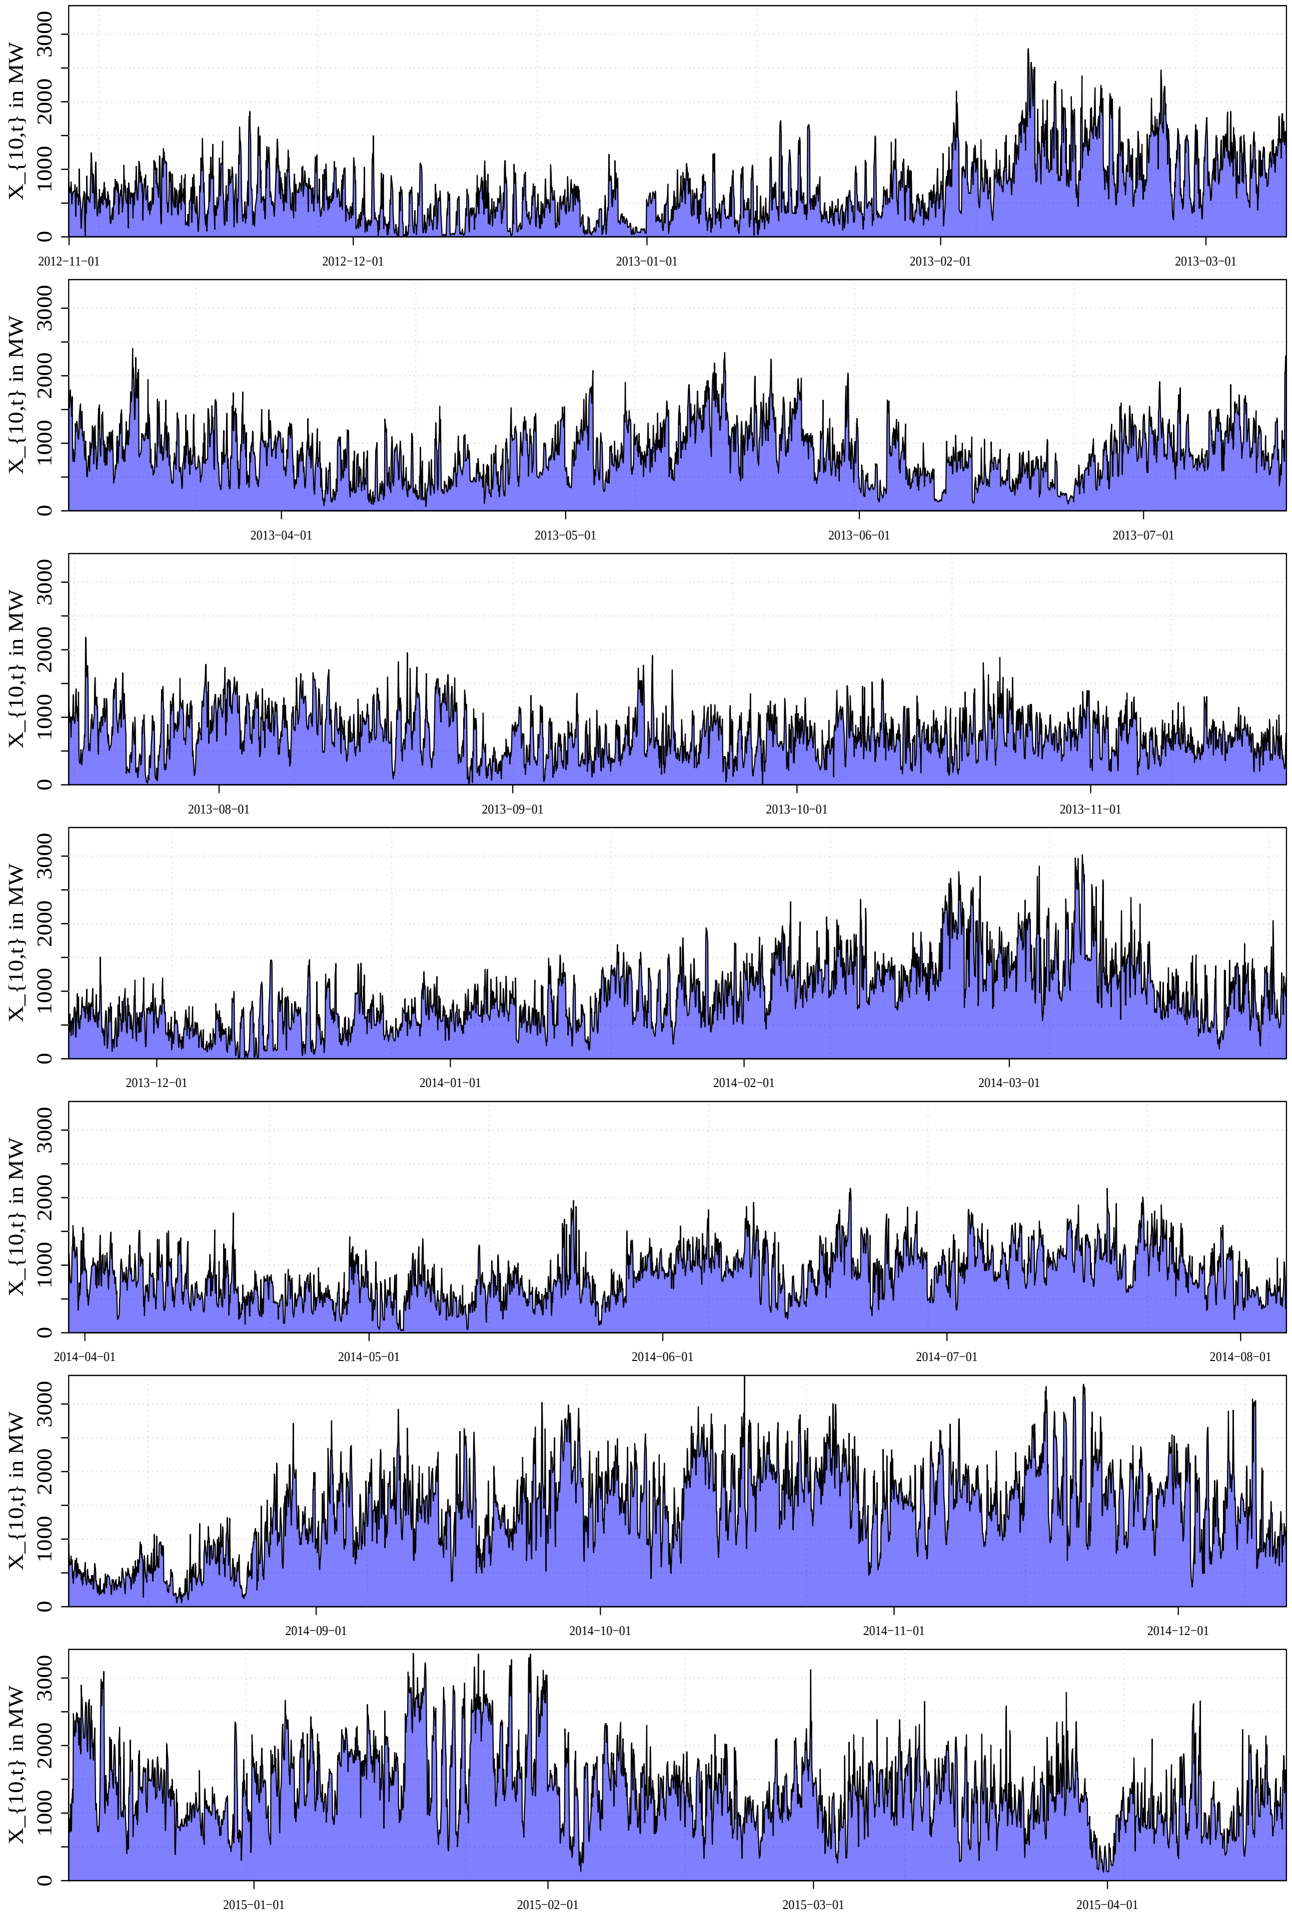


Figure 10: Time series plot of $X_{10,t} = X_{S,t}^{(49.2)}$ with supply/sale bids on $[42.5, 49.2]$

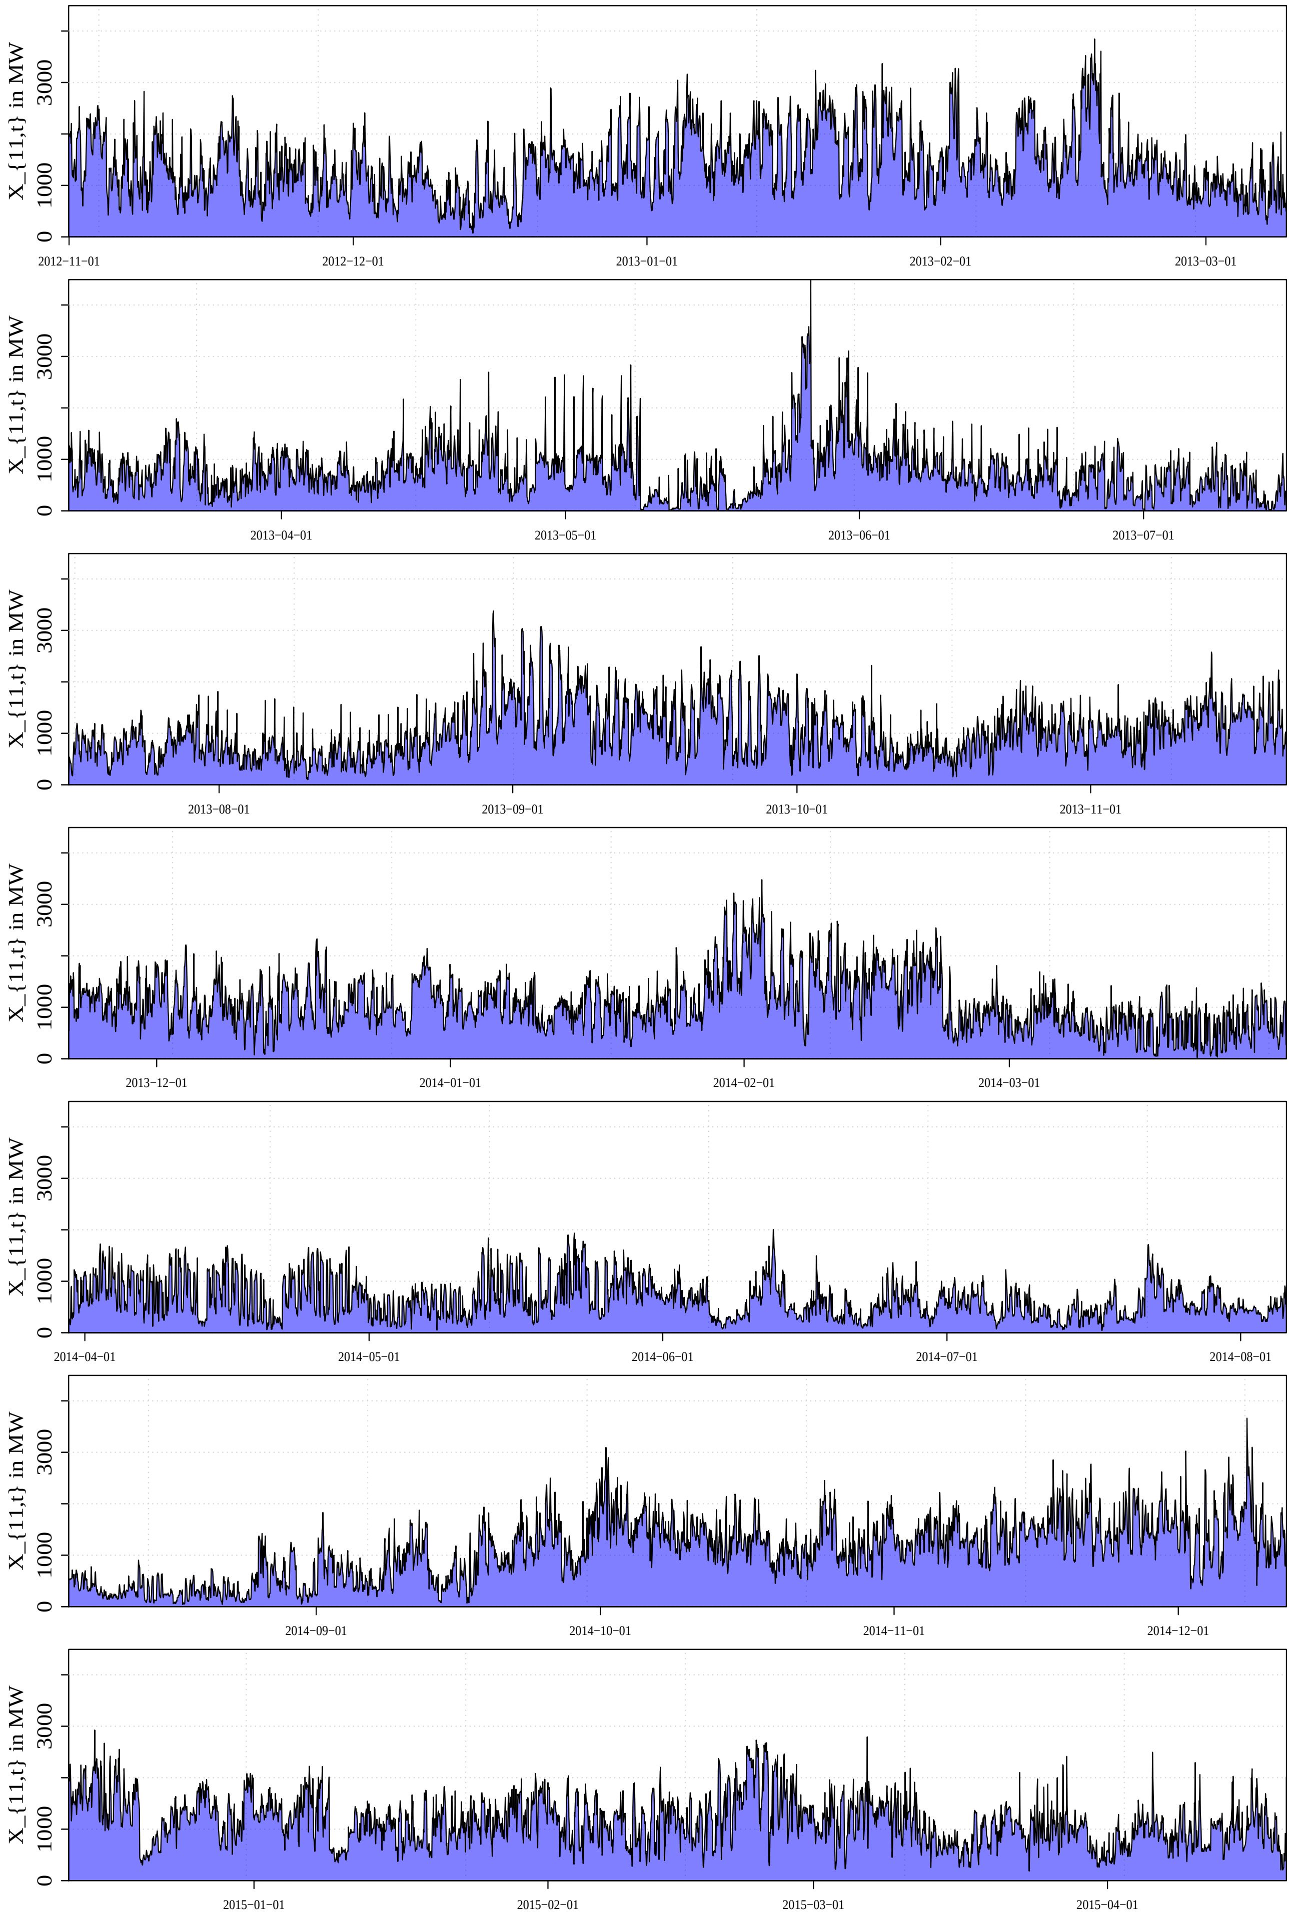


Figure 11: Time series plot of $X_{11,t} = X_{S,t}^{(58.0)}$ with supply/sale bids on $[49.3, 58.0]$

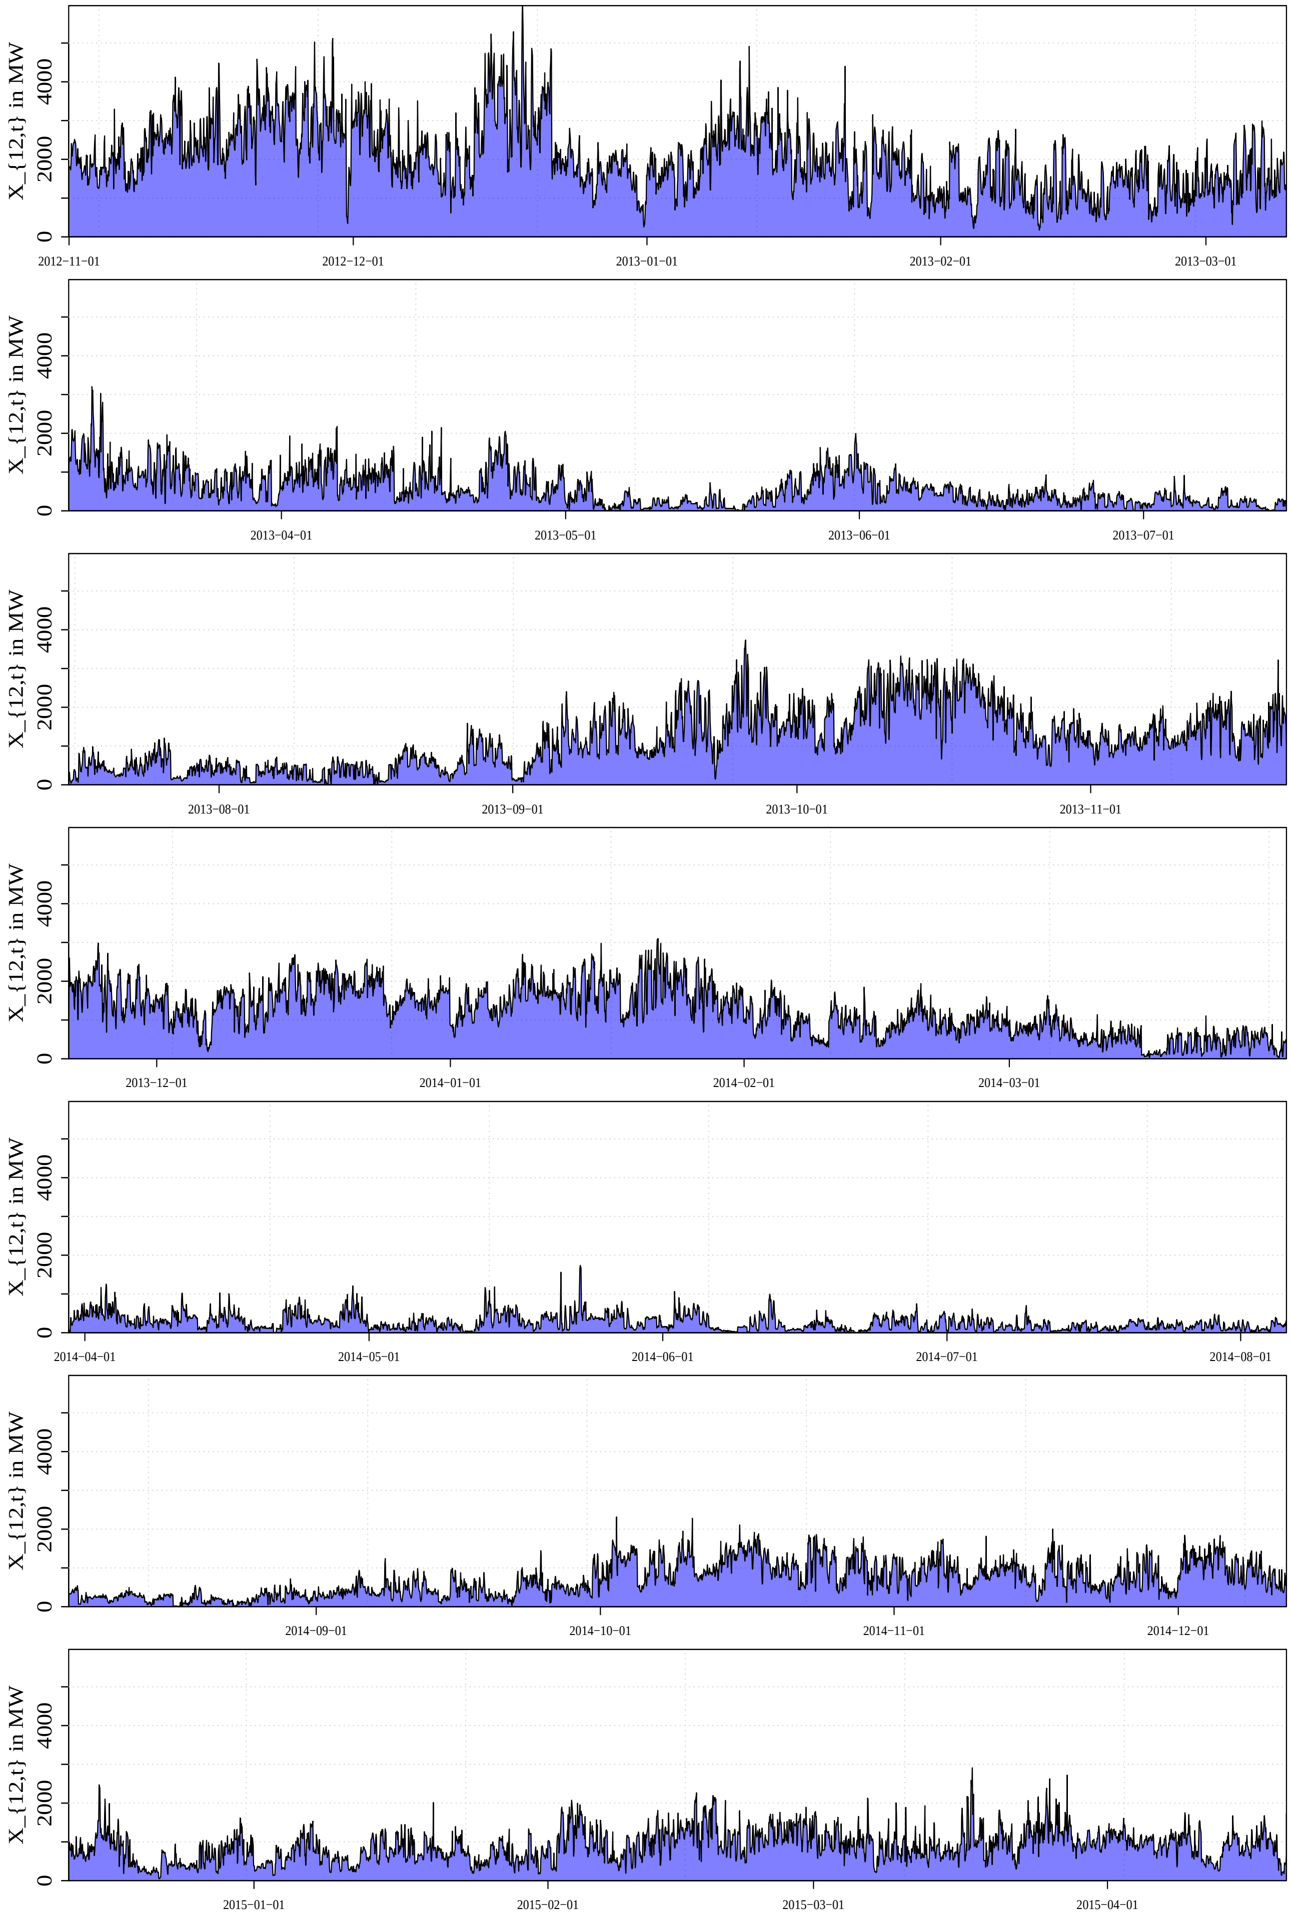


Figure 12: Time series plot of $X_{12,t} = X_{S,t}^{(72.2)}$ with supply/sale bids on $[58.1, 72.2]$

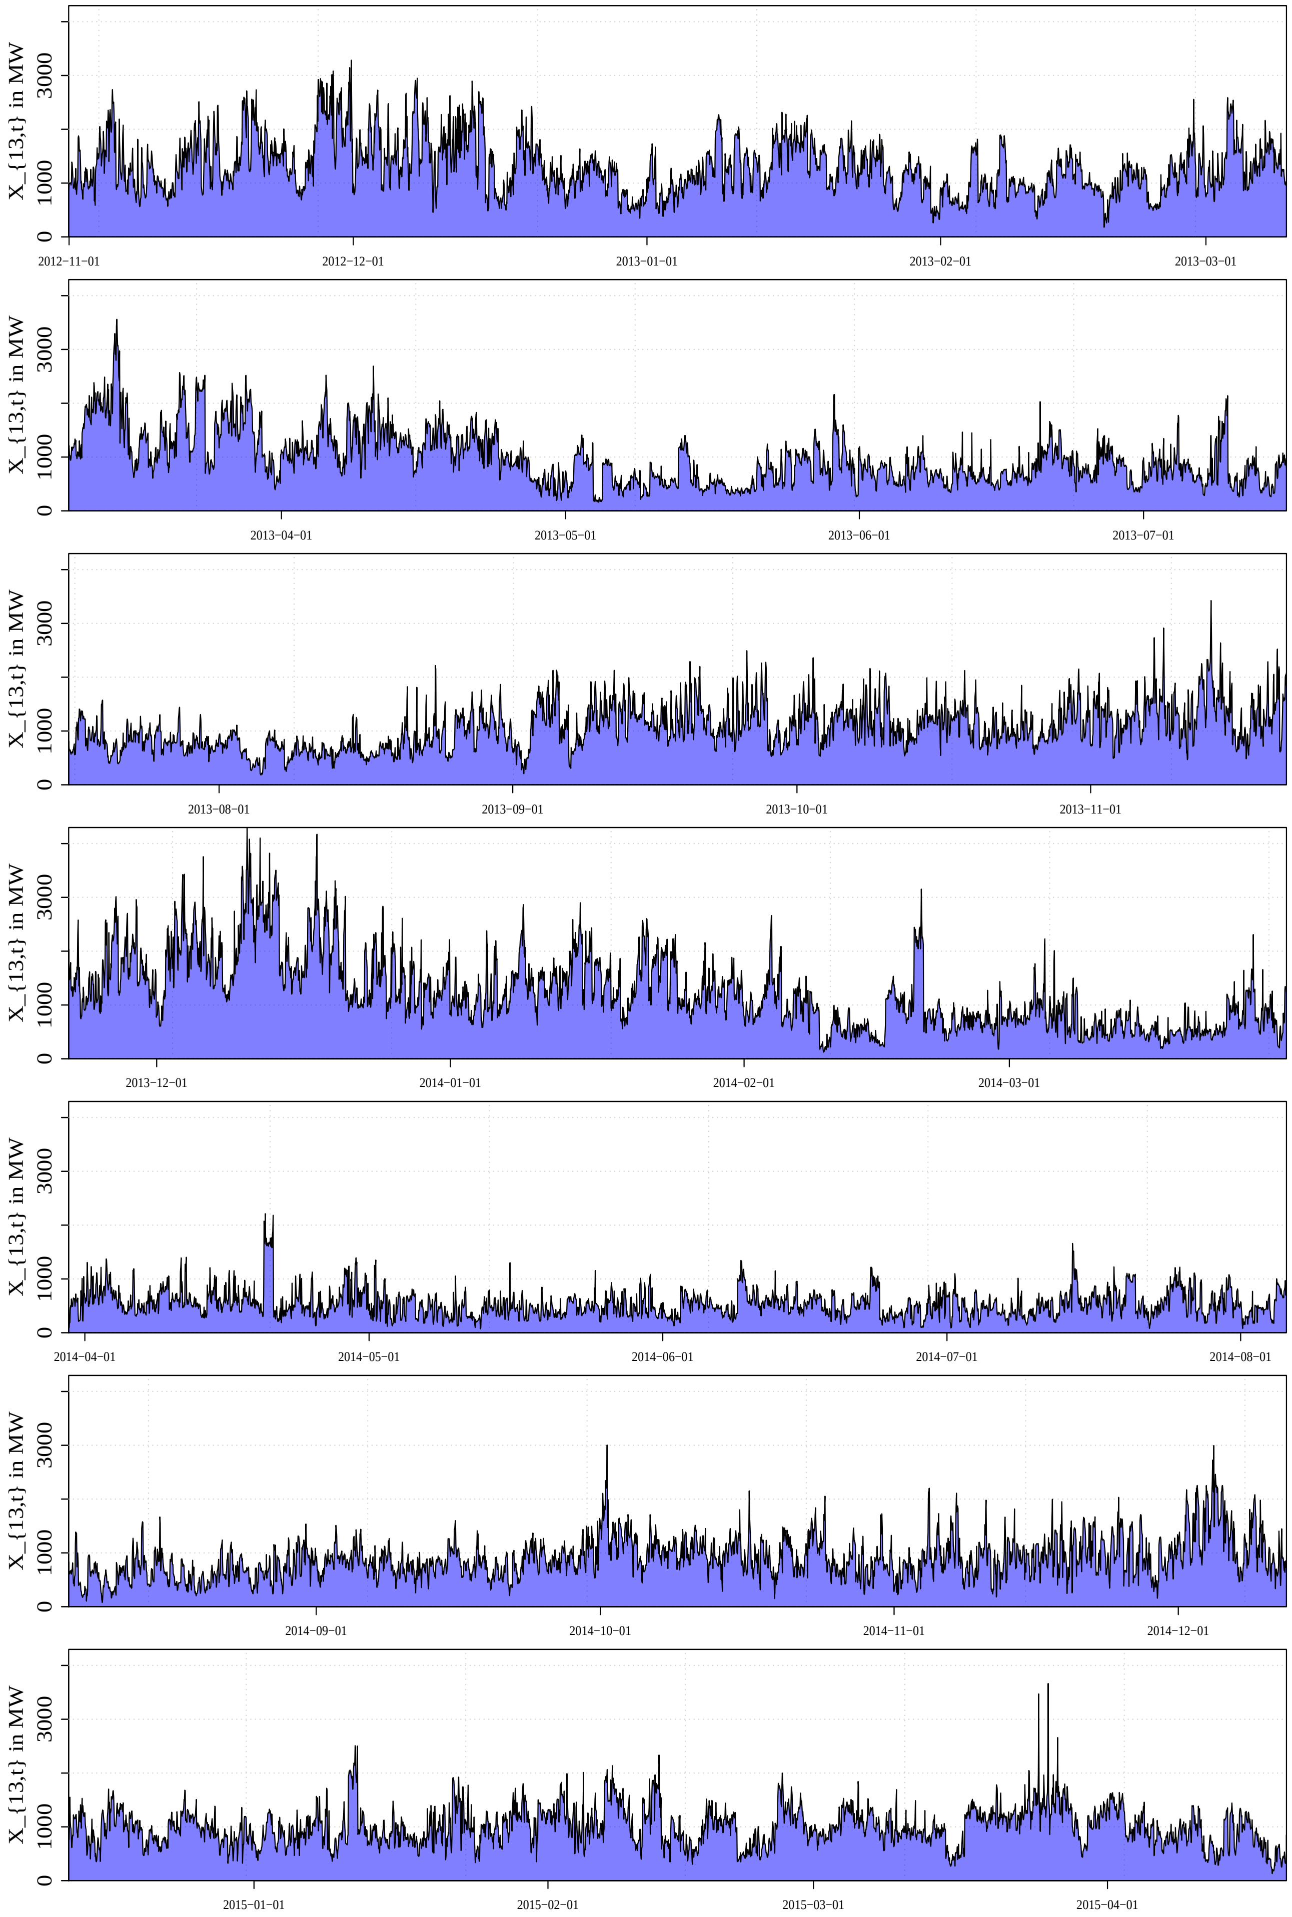


Figure 13: Time series plot of $X_{13,t} = X_{S,t}^{(225.0)}$ with supply/sale bids on $[72.3, 225.0]$

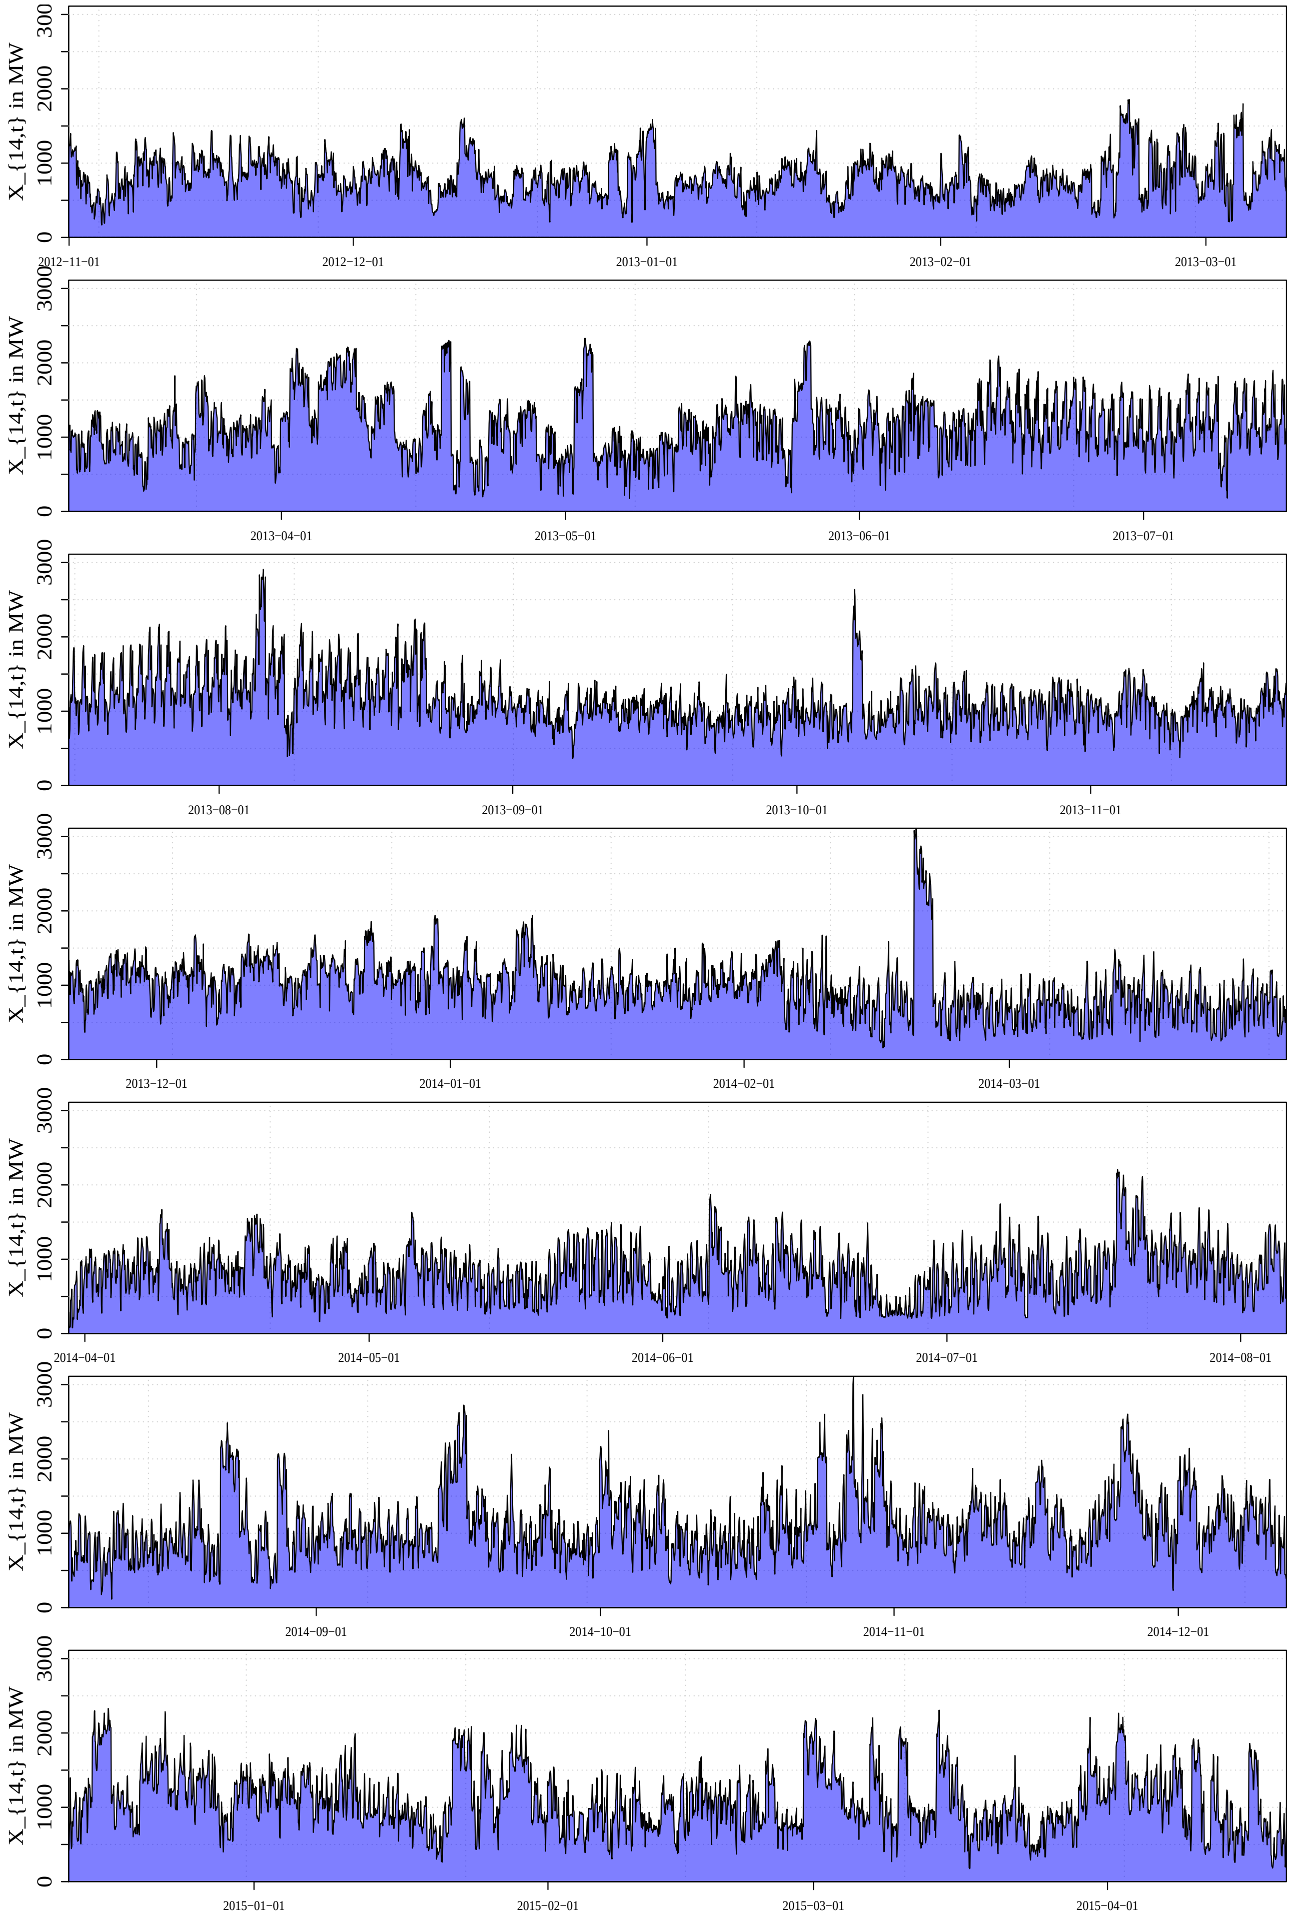


Figure 14: Time series plot of $X_{14,t} = X_{S,t}^{(950.0)}$ with supply/sale bids on $[225.1, 950.0]$

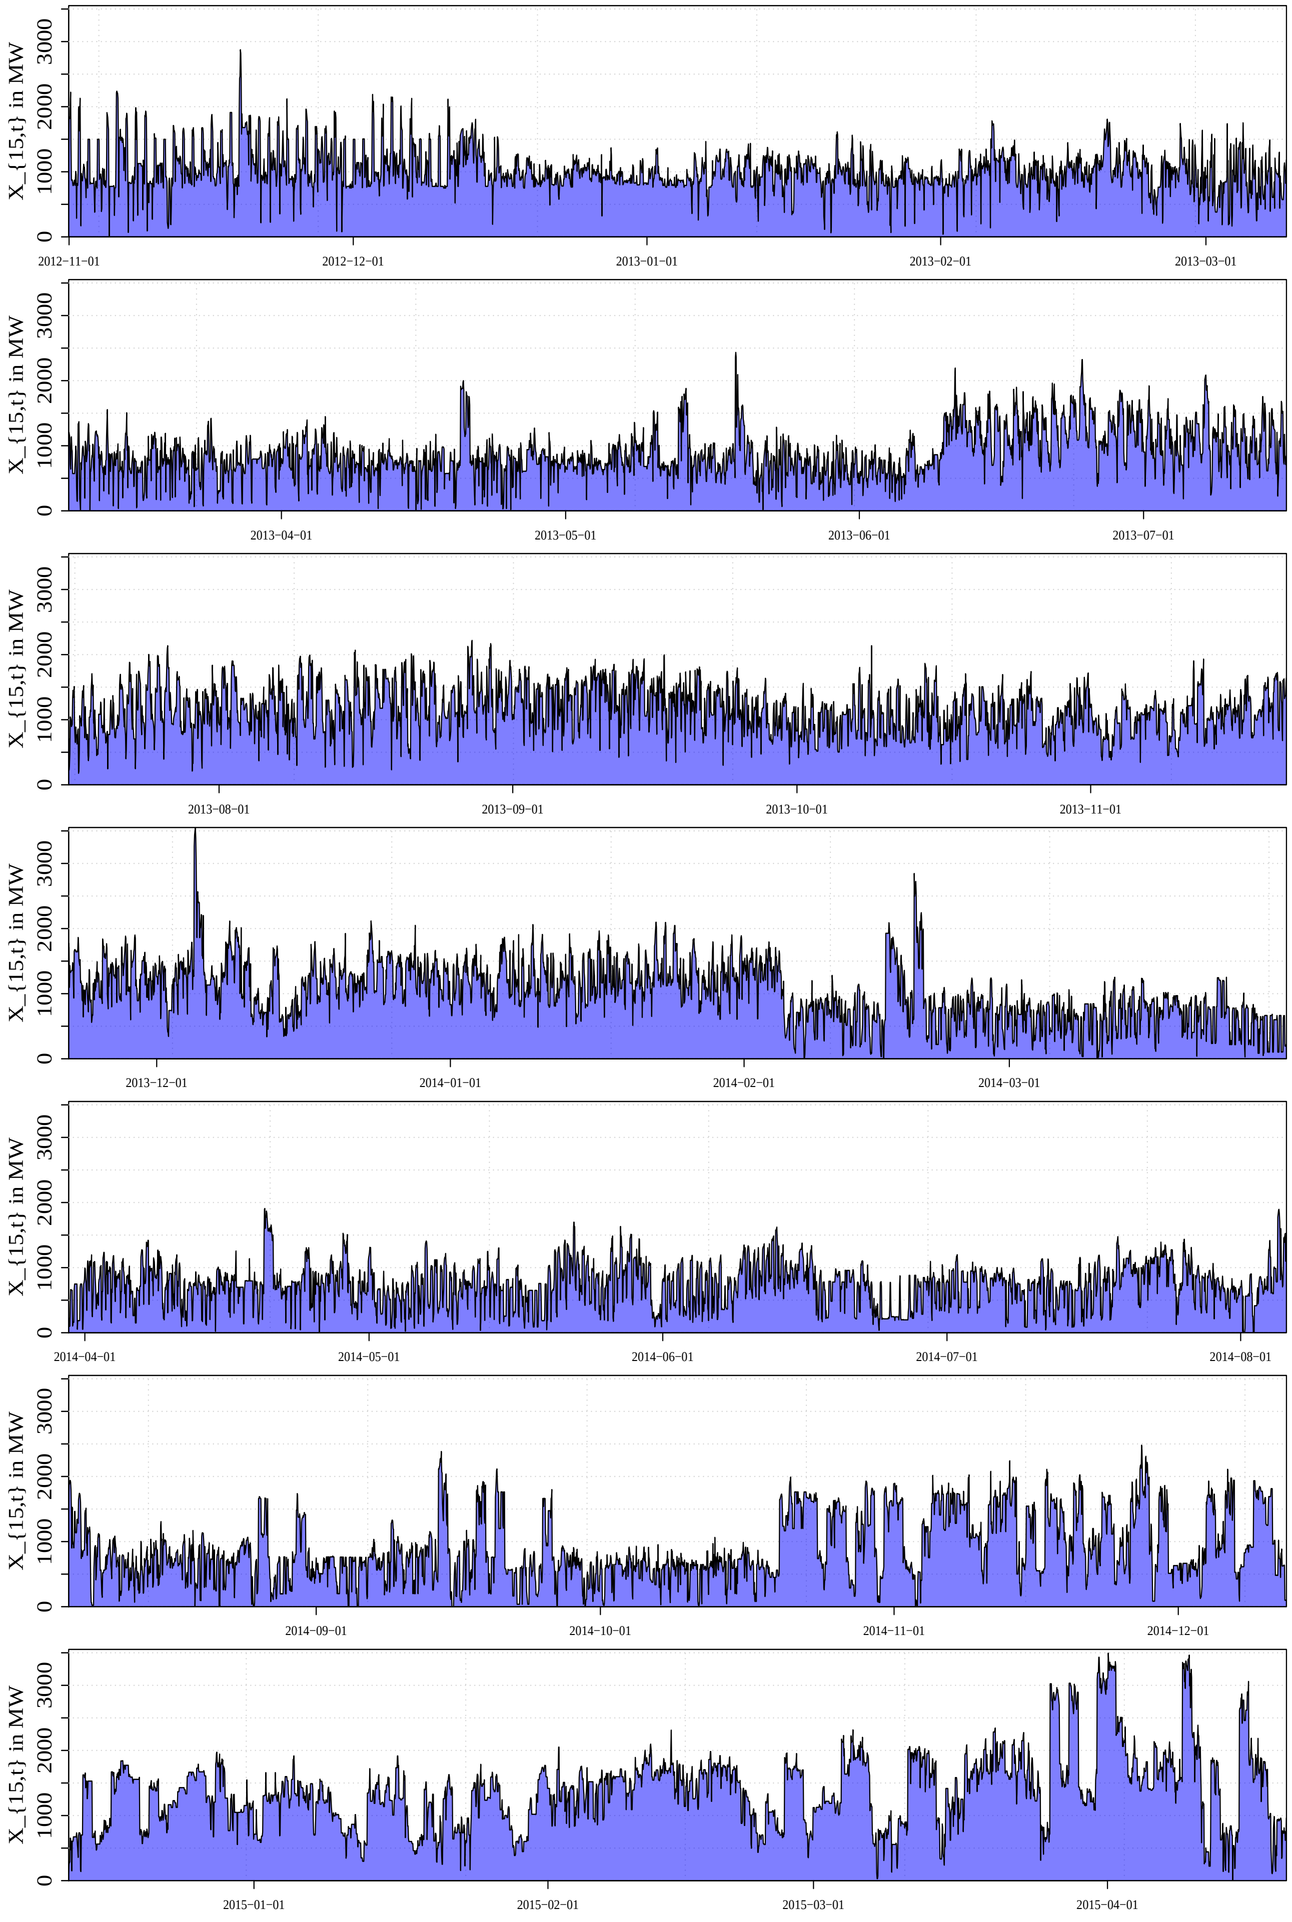


Figure 15: Time series plot of $X_{15,t} = X_{S,t}^{(2883.0)}$ with supply/sale bids on $[950.1, 2883.0]$

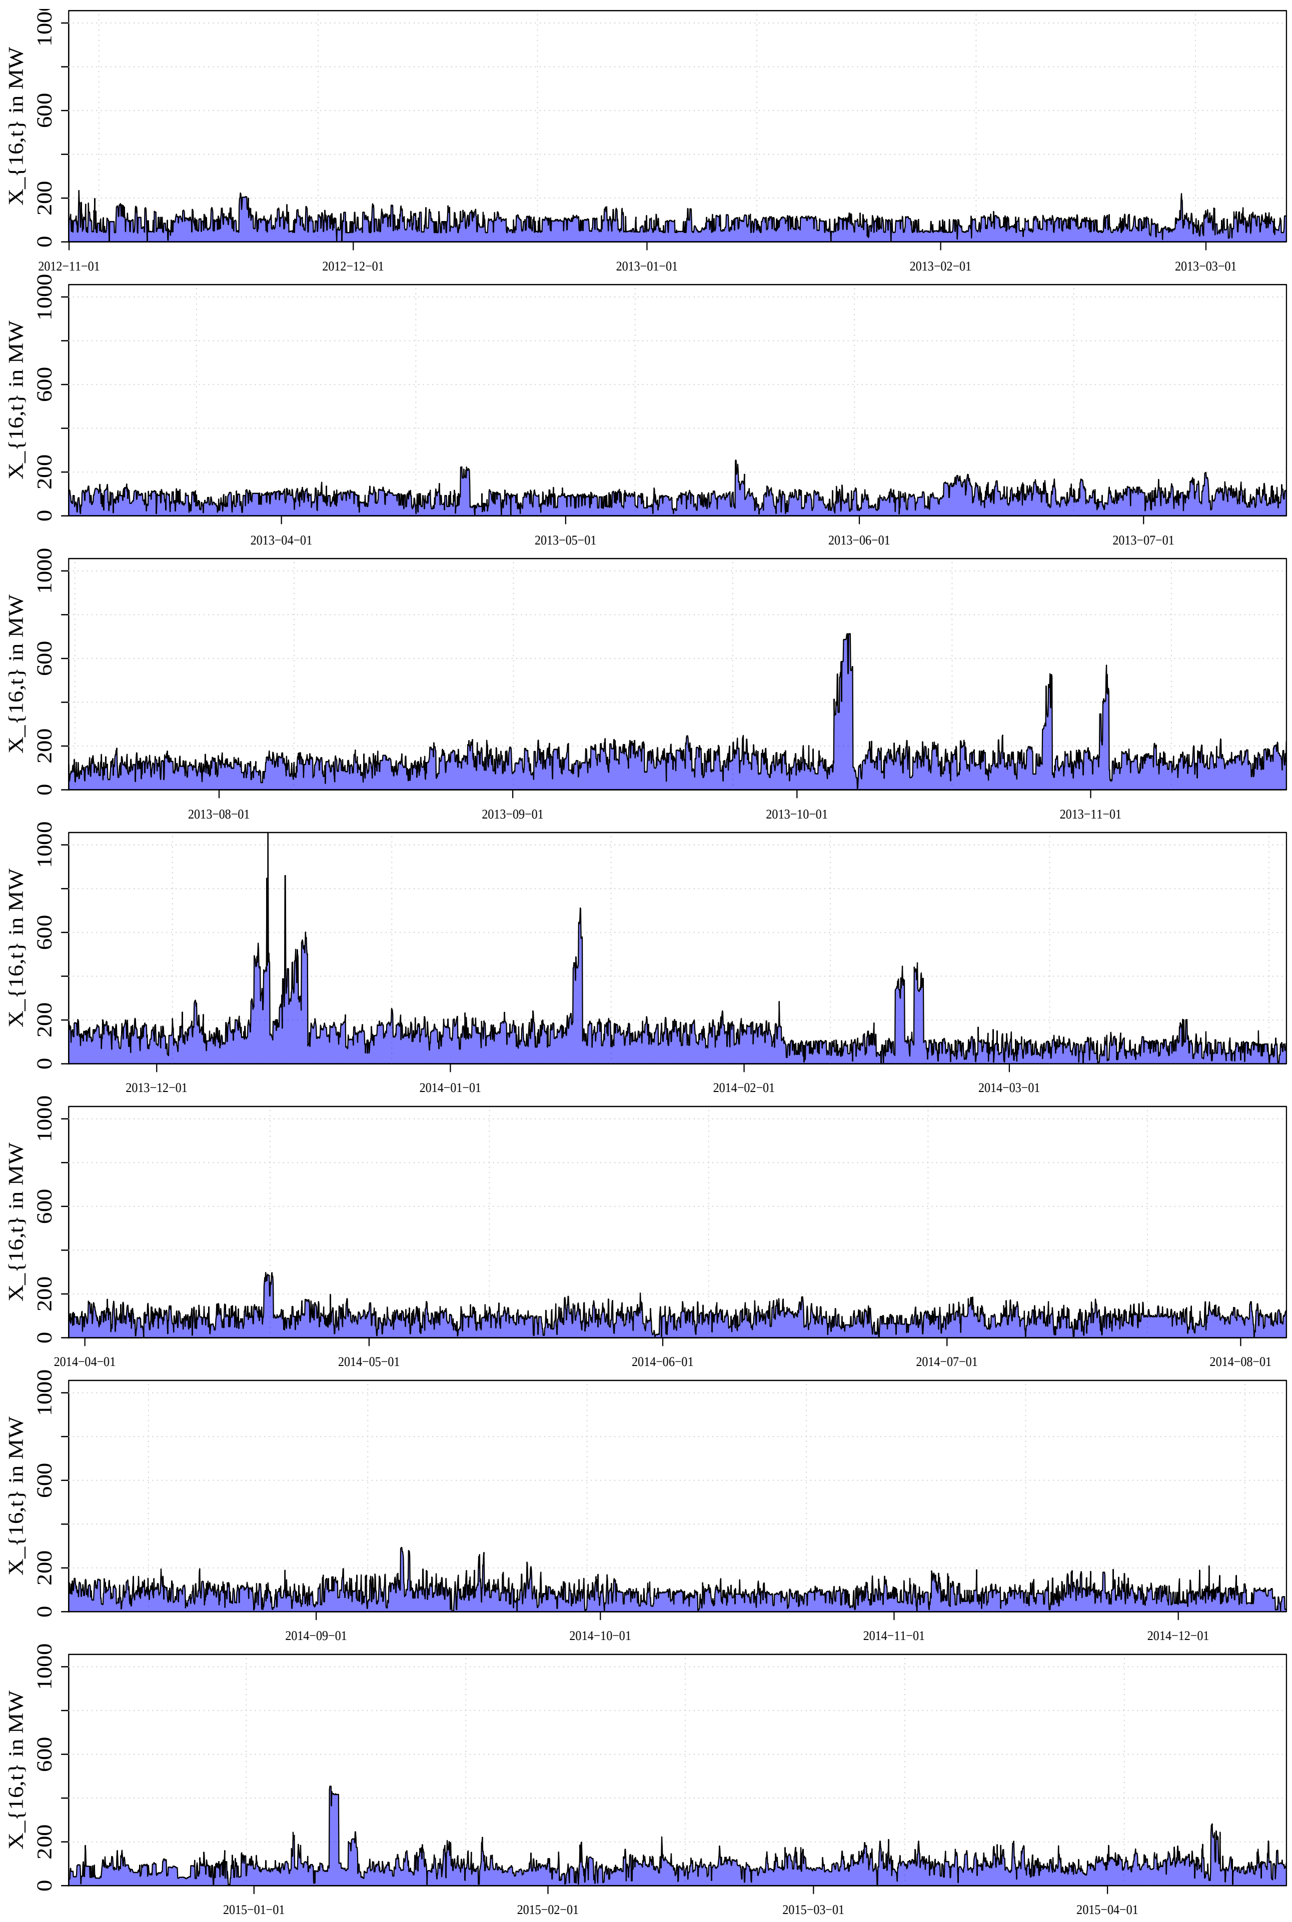


Figure 16: Time series plot of $X_{16,t} = X_{S,t}^{(3000)}$ with supply/sale bids on $[2883.1, 3000]$

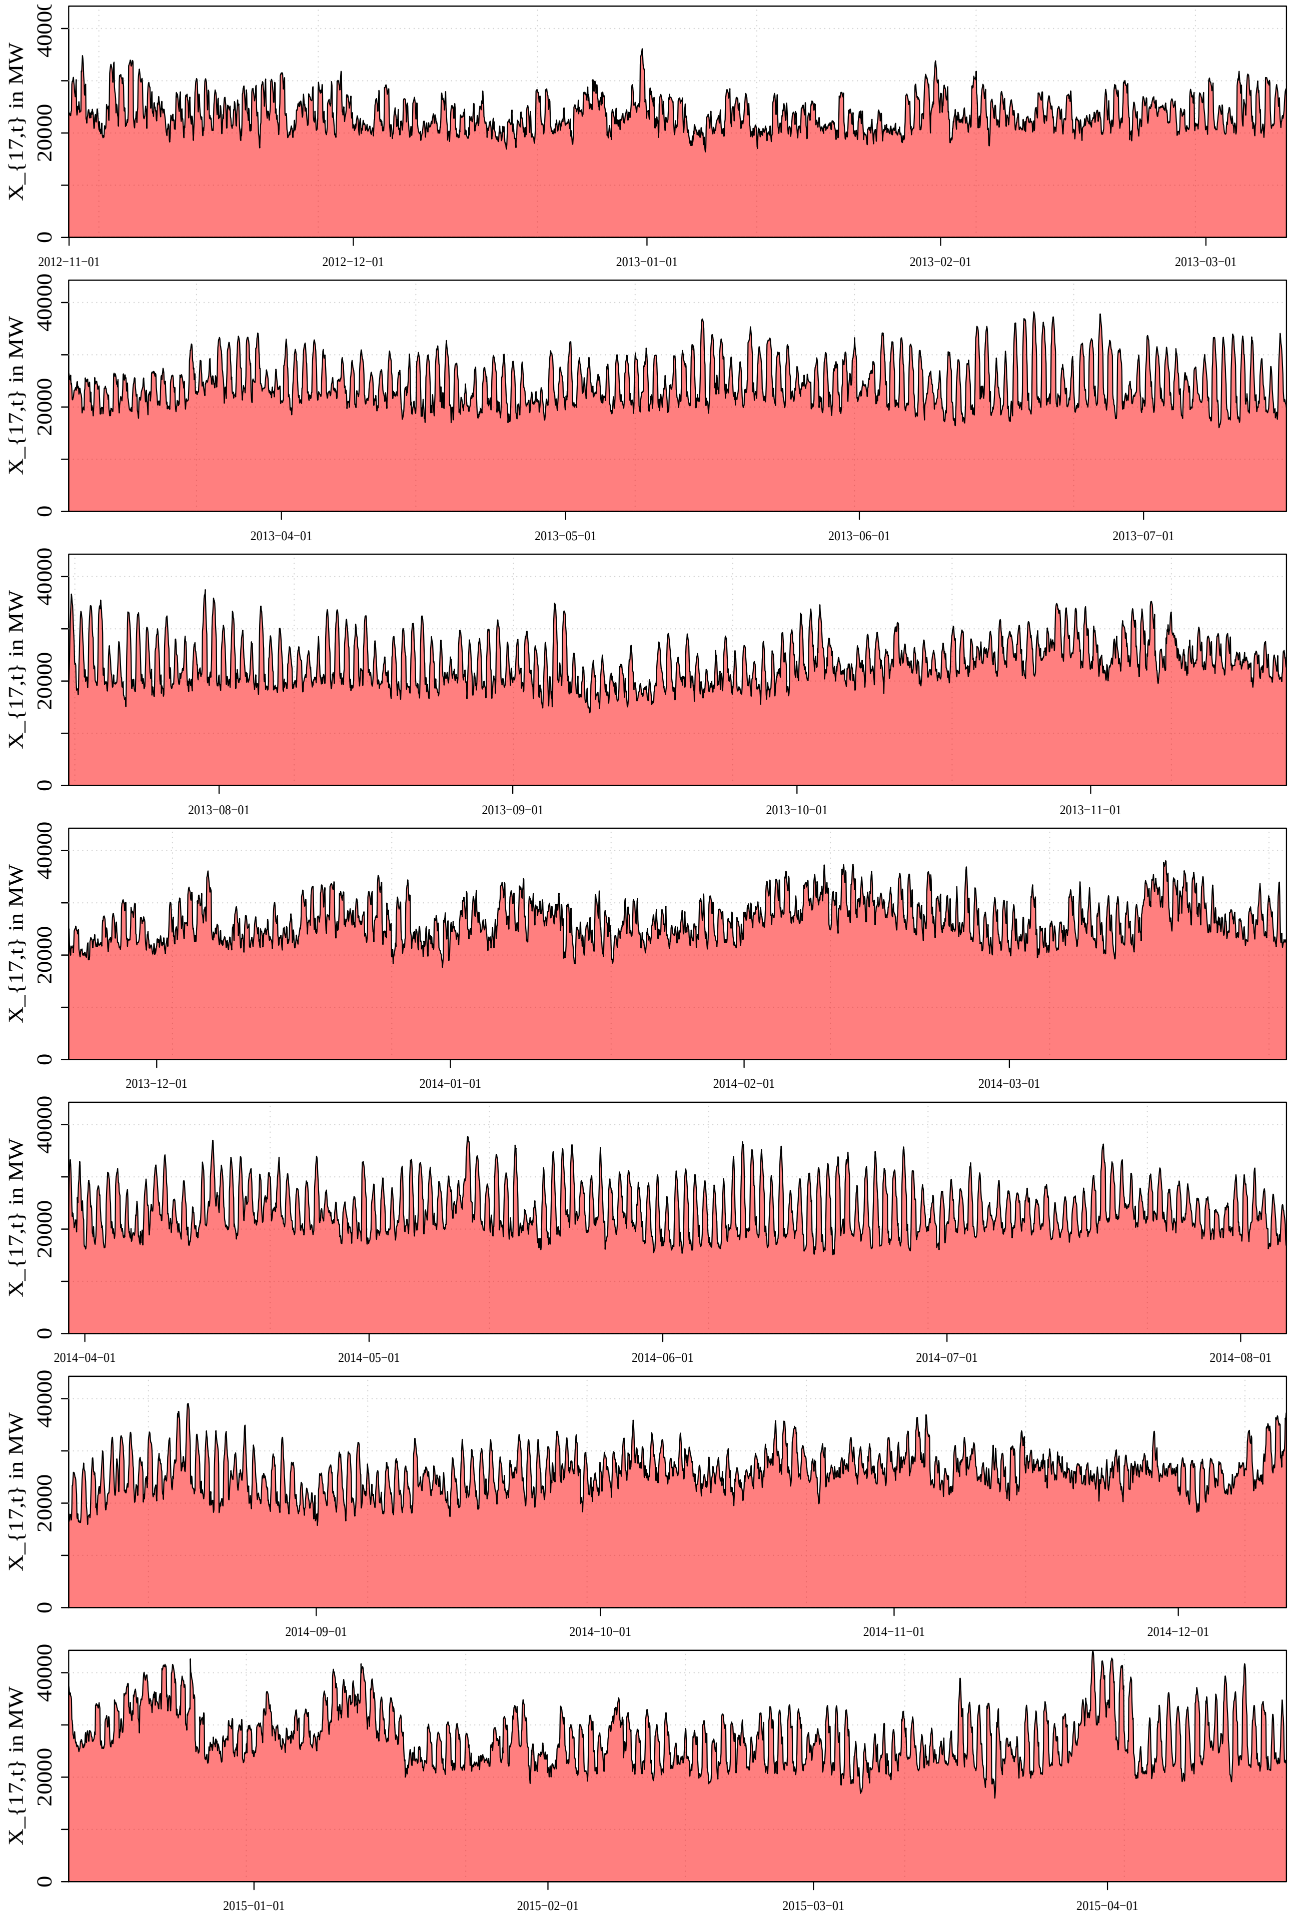


Figure 17: Time series plot of $X_{17,t} = X_{D,t}^{(3000)}$ with demand/purchase bids on exactly 3000

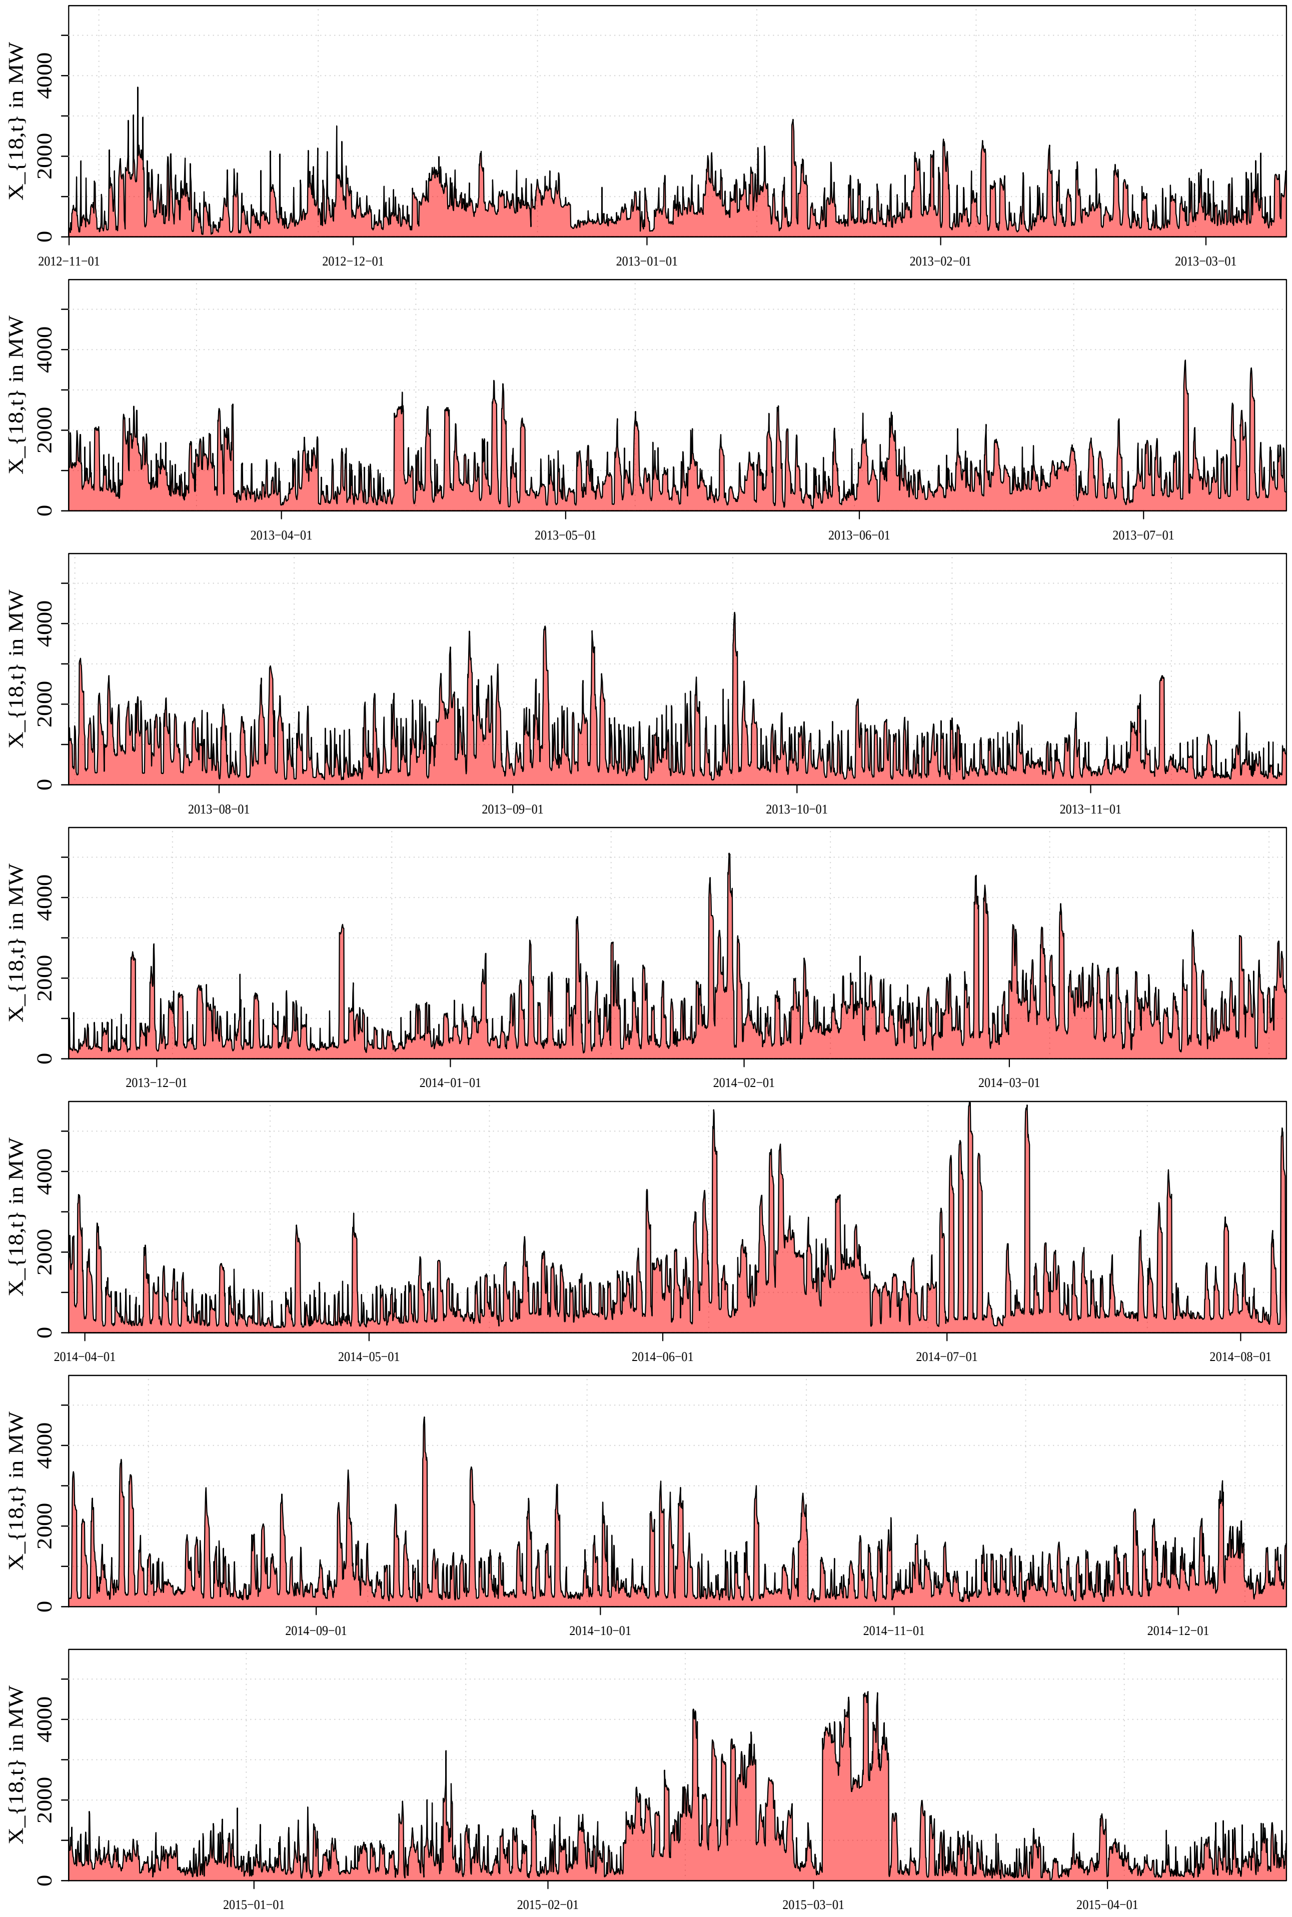


Figure 18: Time series plot of $X_{18,t} = X_{D,t}^{(499.9)}$ with demand/purchase bids on $[499.9, 2999.9]$

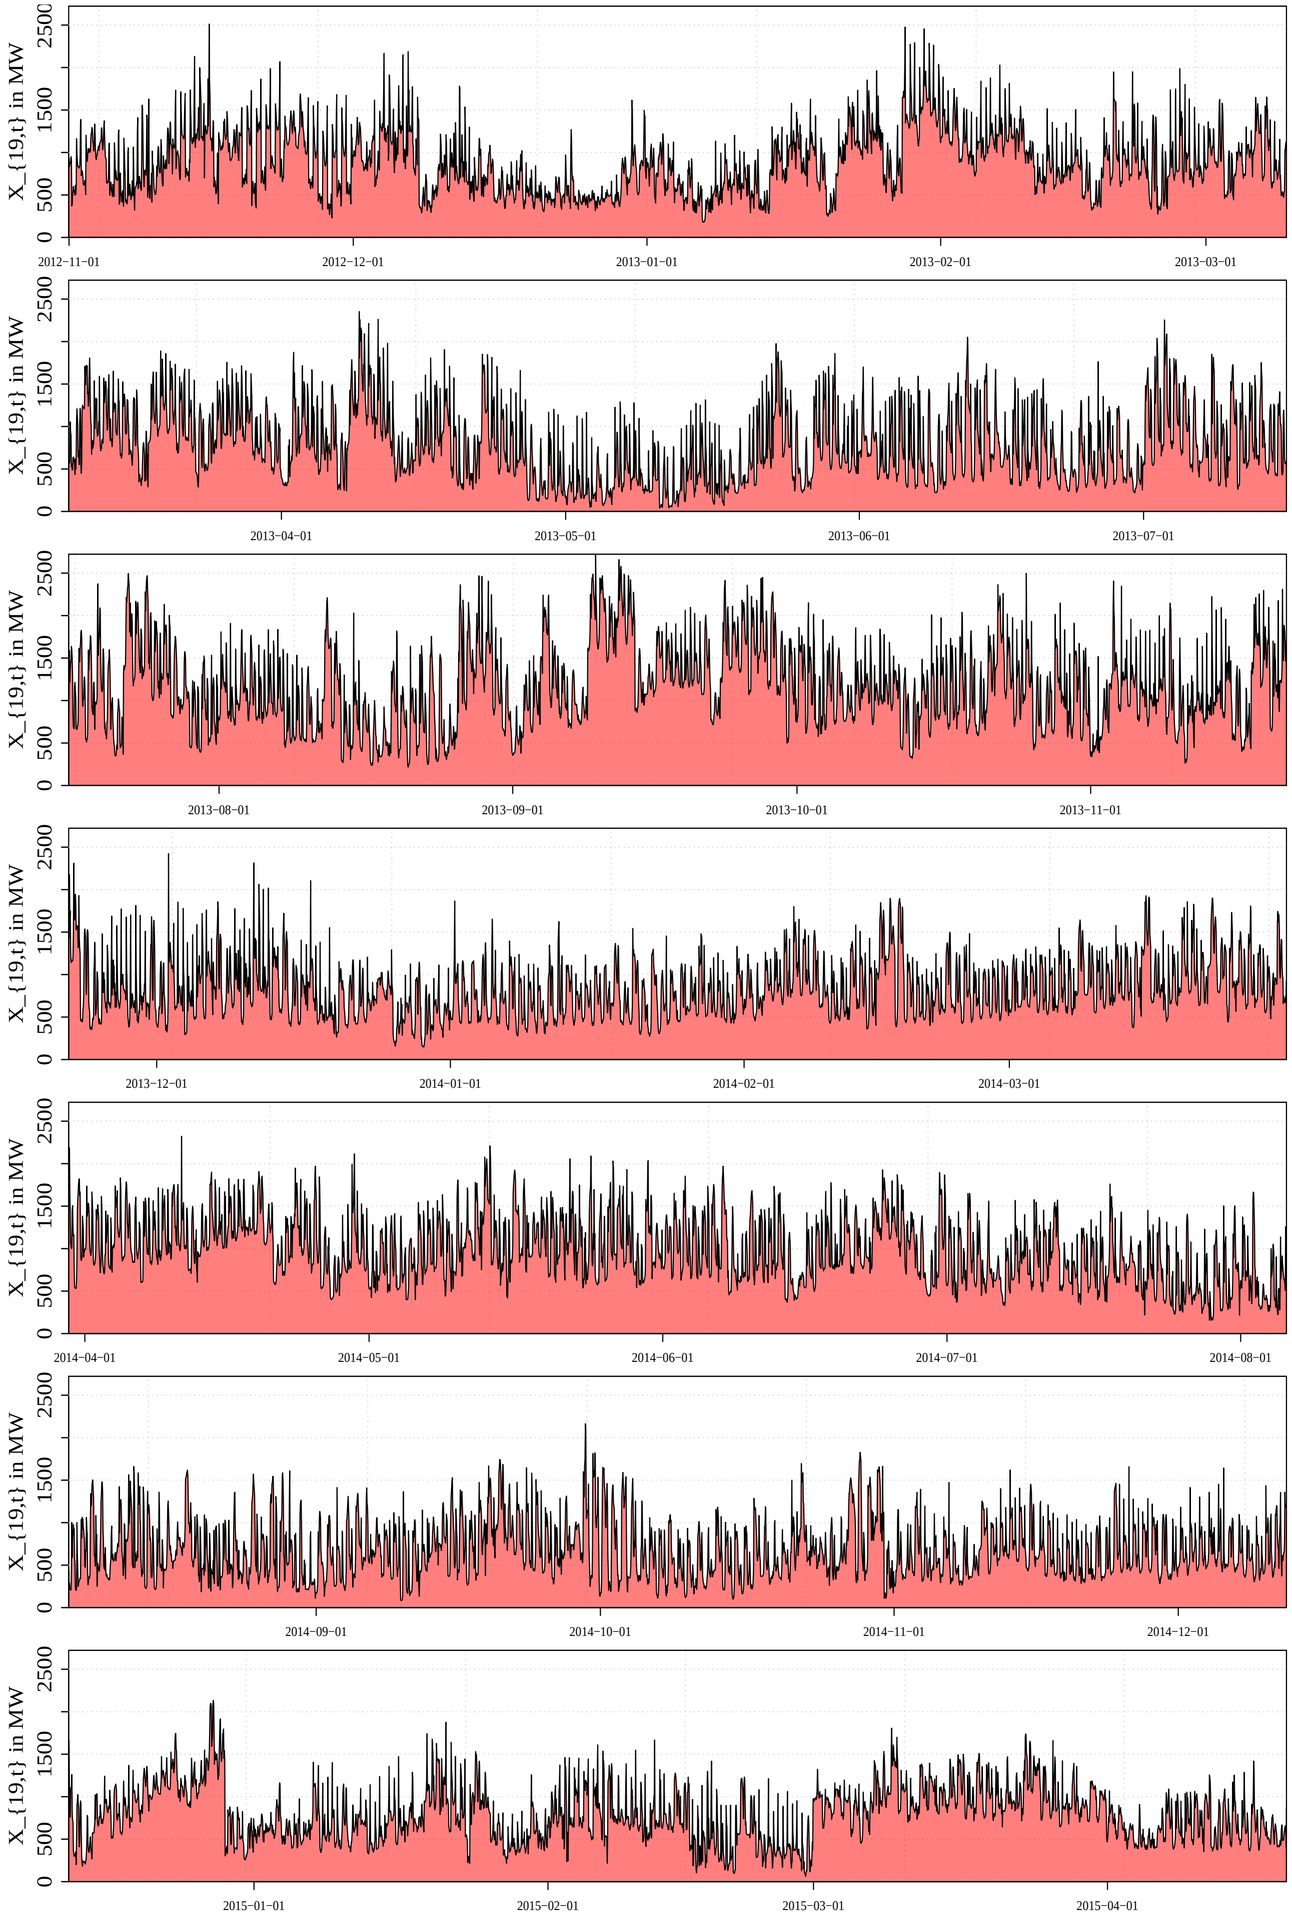


Figure 19: Time series plot of $X_{19,t} = X_{D,t}^{(157.4)}$ with demand/purchase bids on $[157.4, 499.8]$

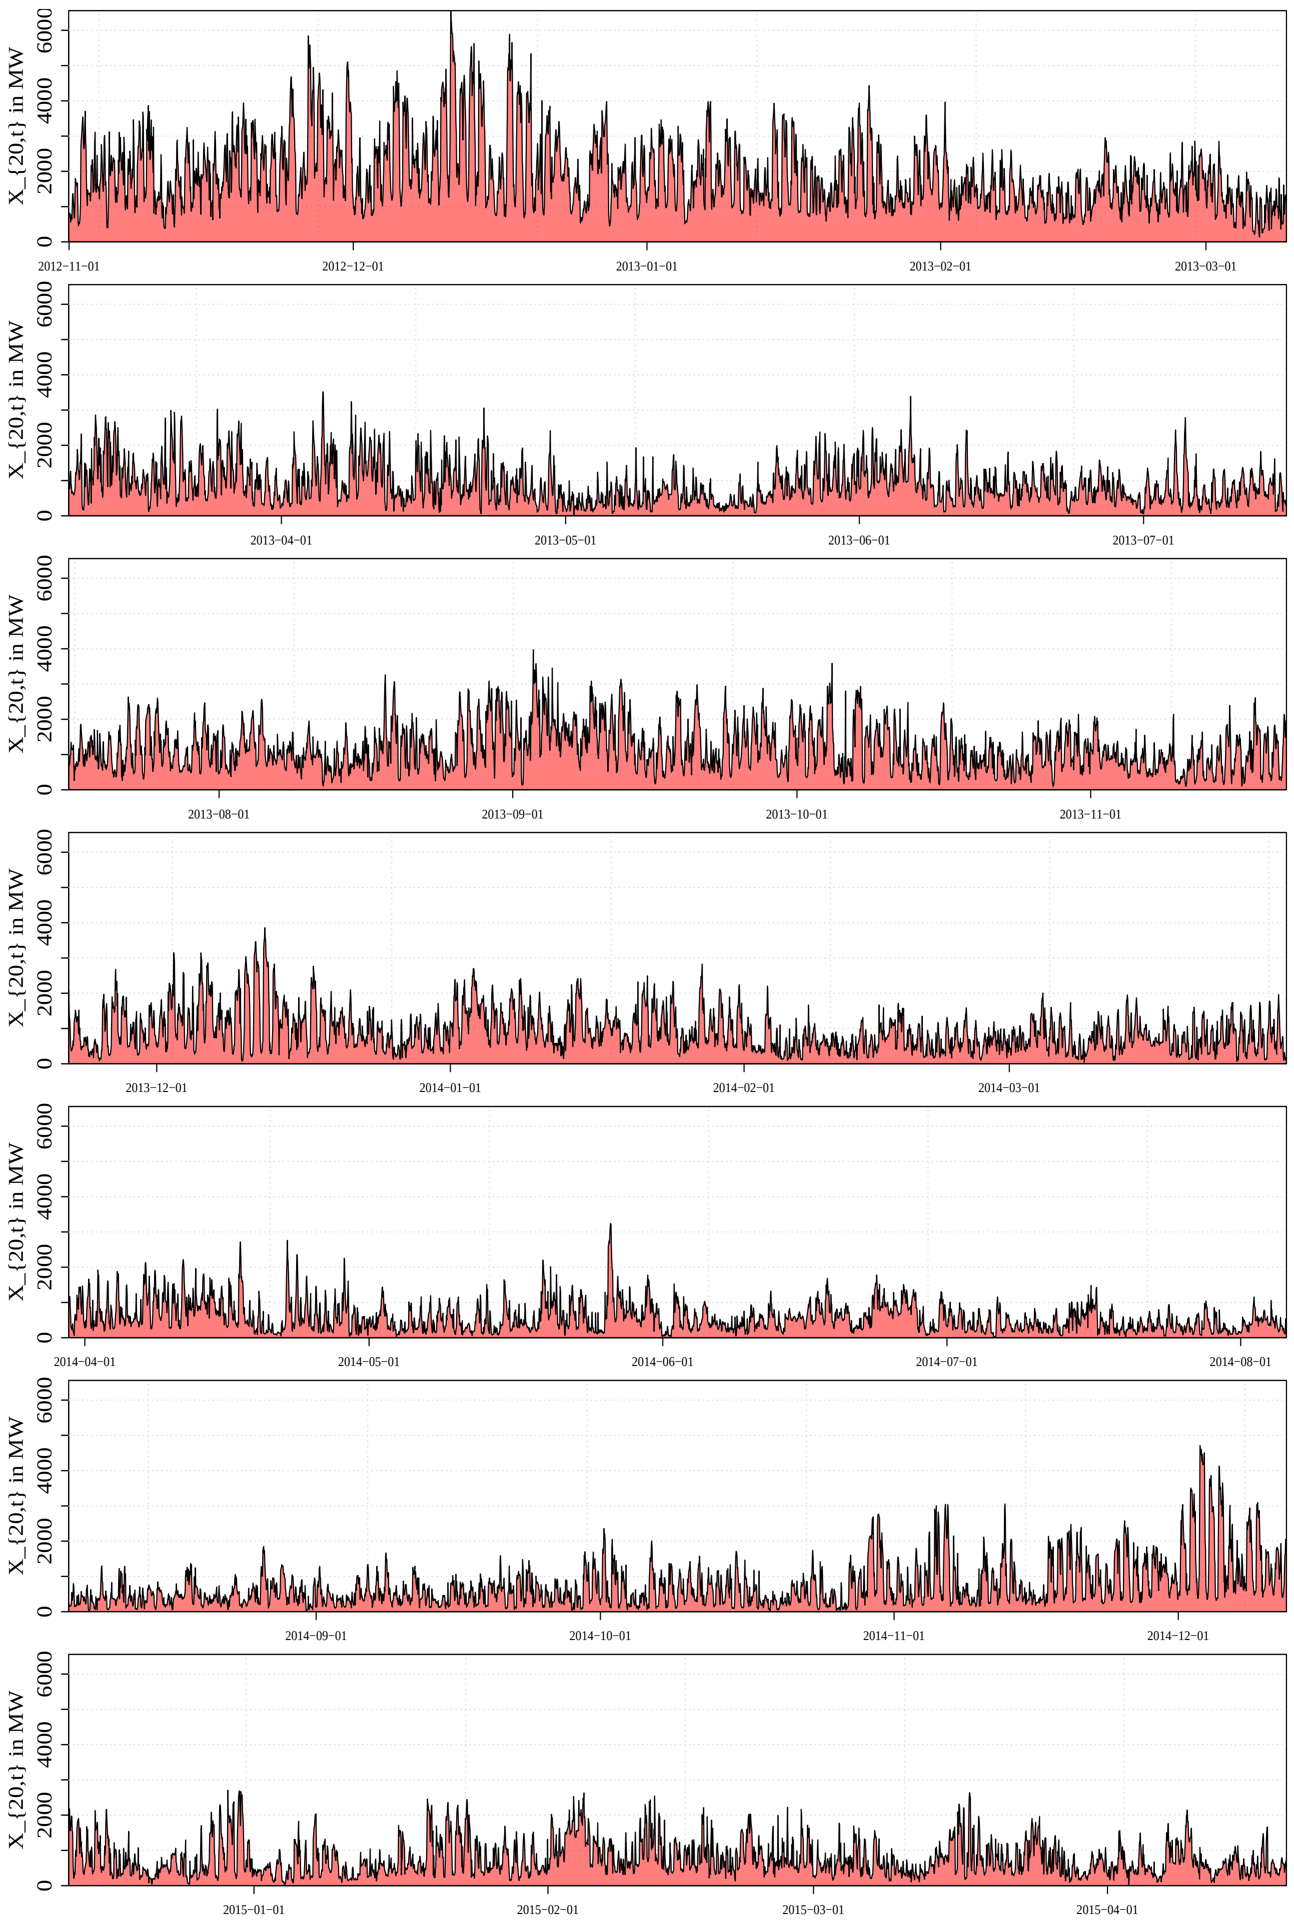


Figure 20: Time series plot of $X_{20,t} = X_{D,t}^{(52.6)}$ with demand/purchase bids on $[52.6, 157.3]$

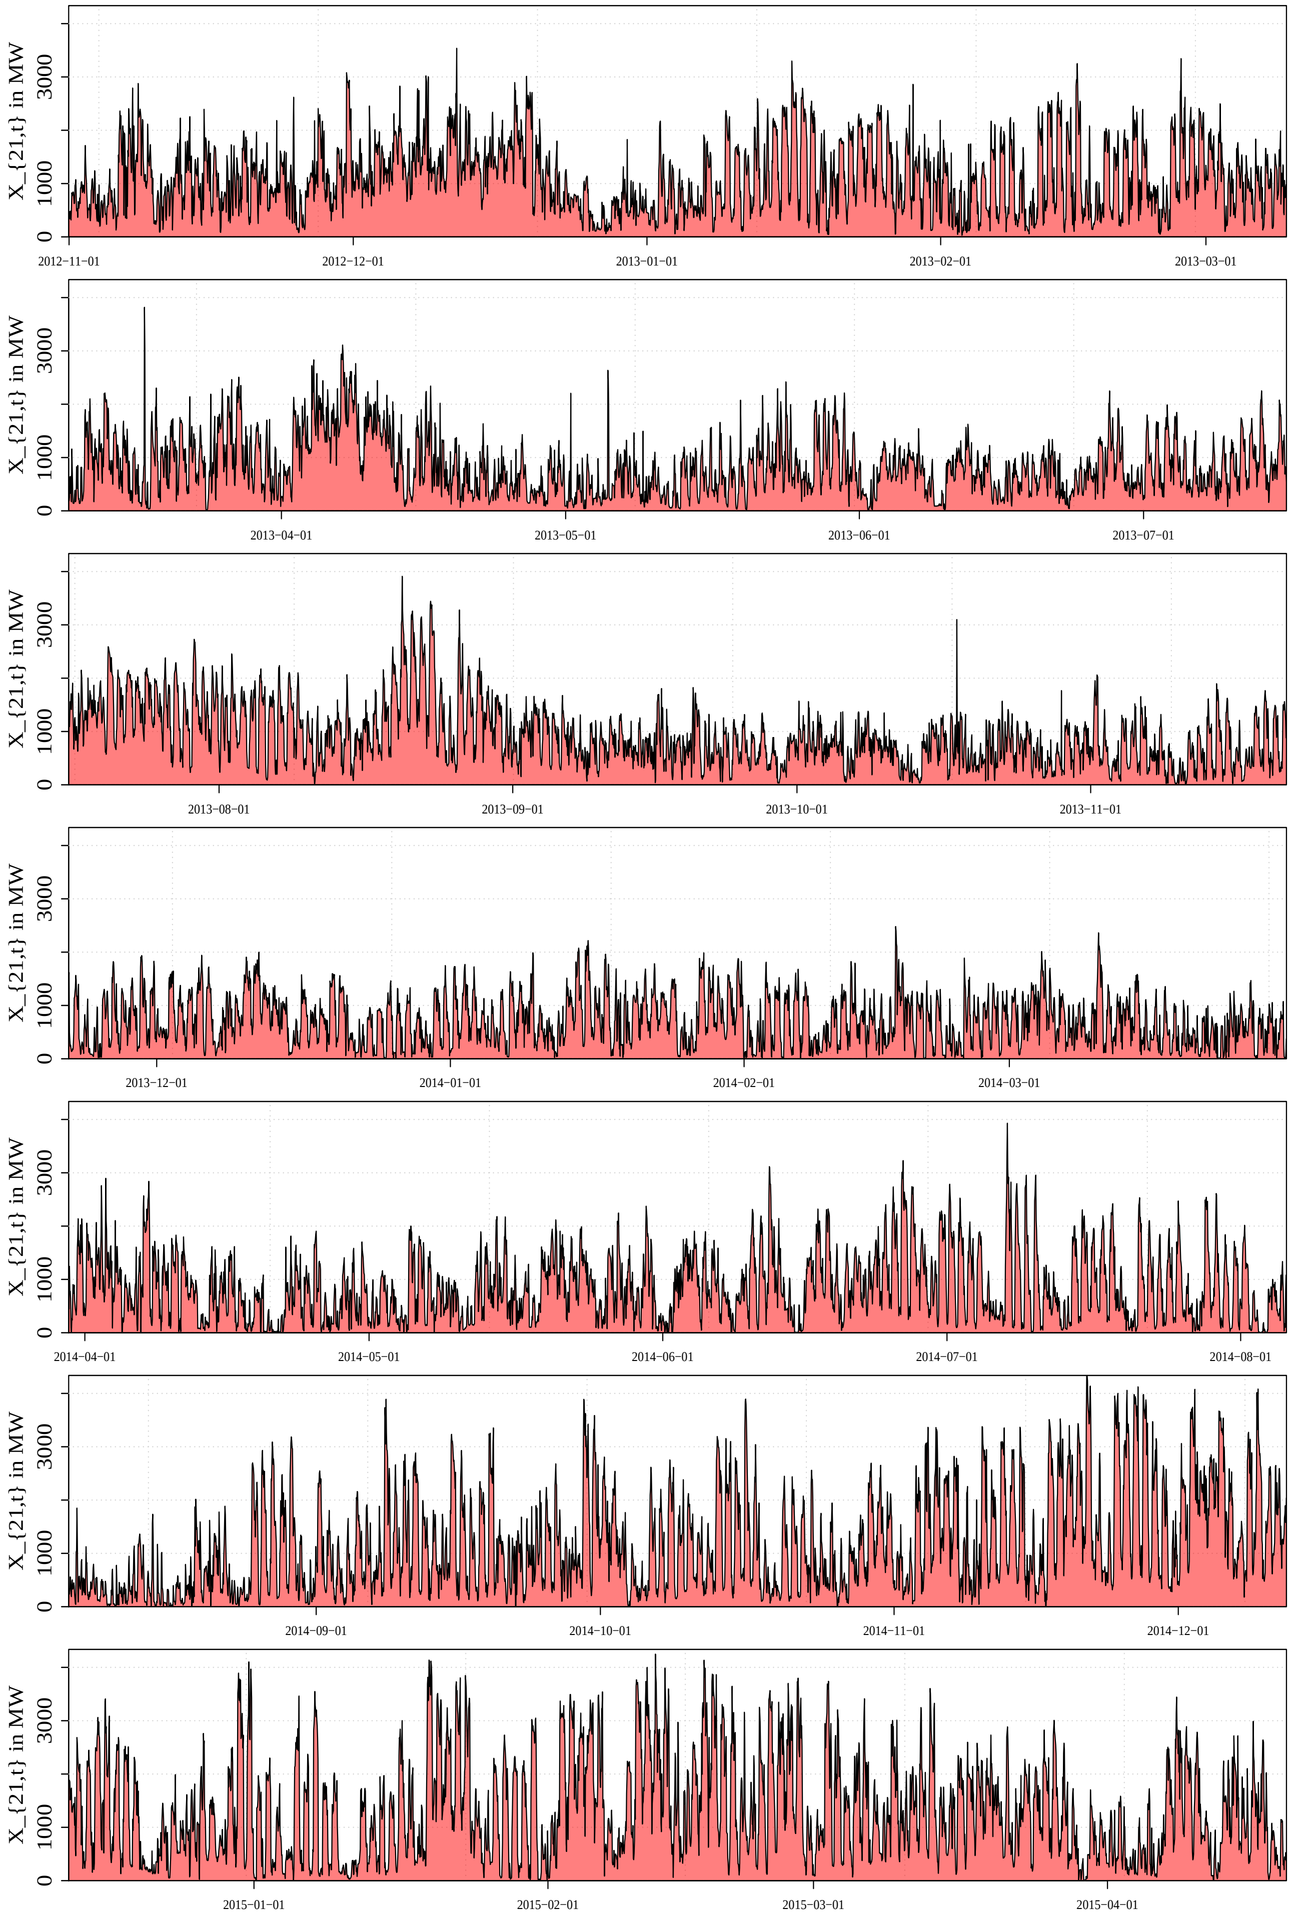


Figure 21: Time series plot of $X_{21,t} = X^{(37.3)}_{D,t}$ with demand/purchase bids on $[37.3, 52.5]$

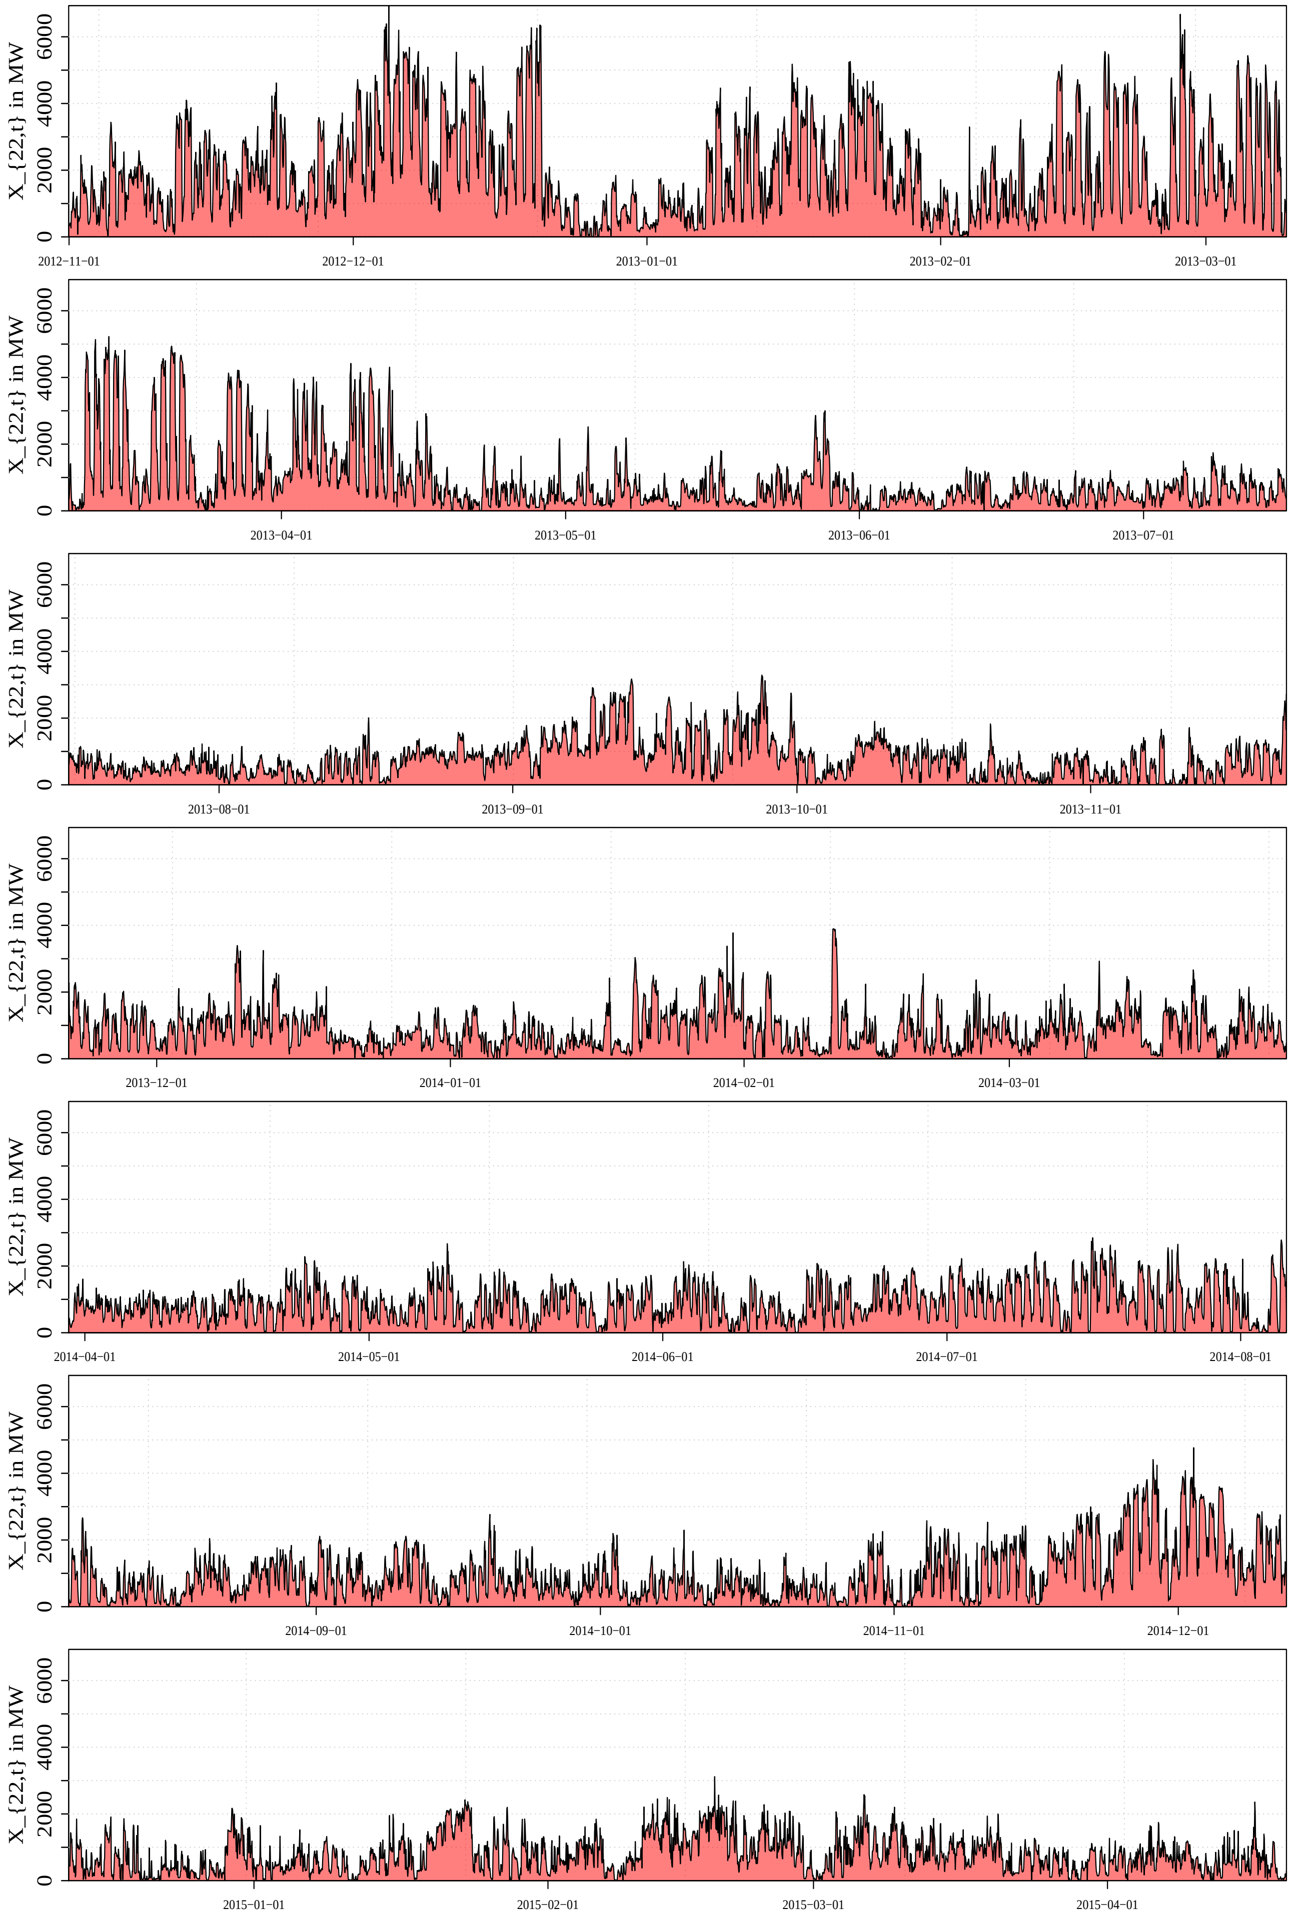


Figure 22: Time series plot of $X_{22,t} = X_{D,t}^{(30.9)}$ with demand/purchase bids on $[30.9, 37.2]$

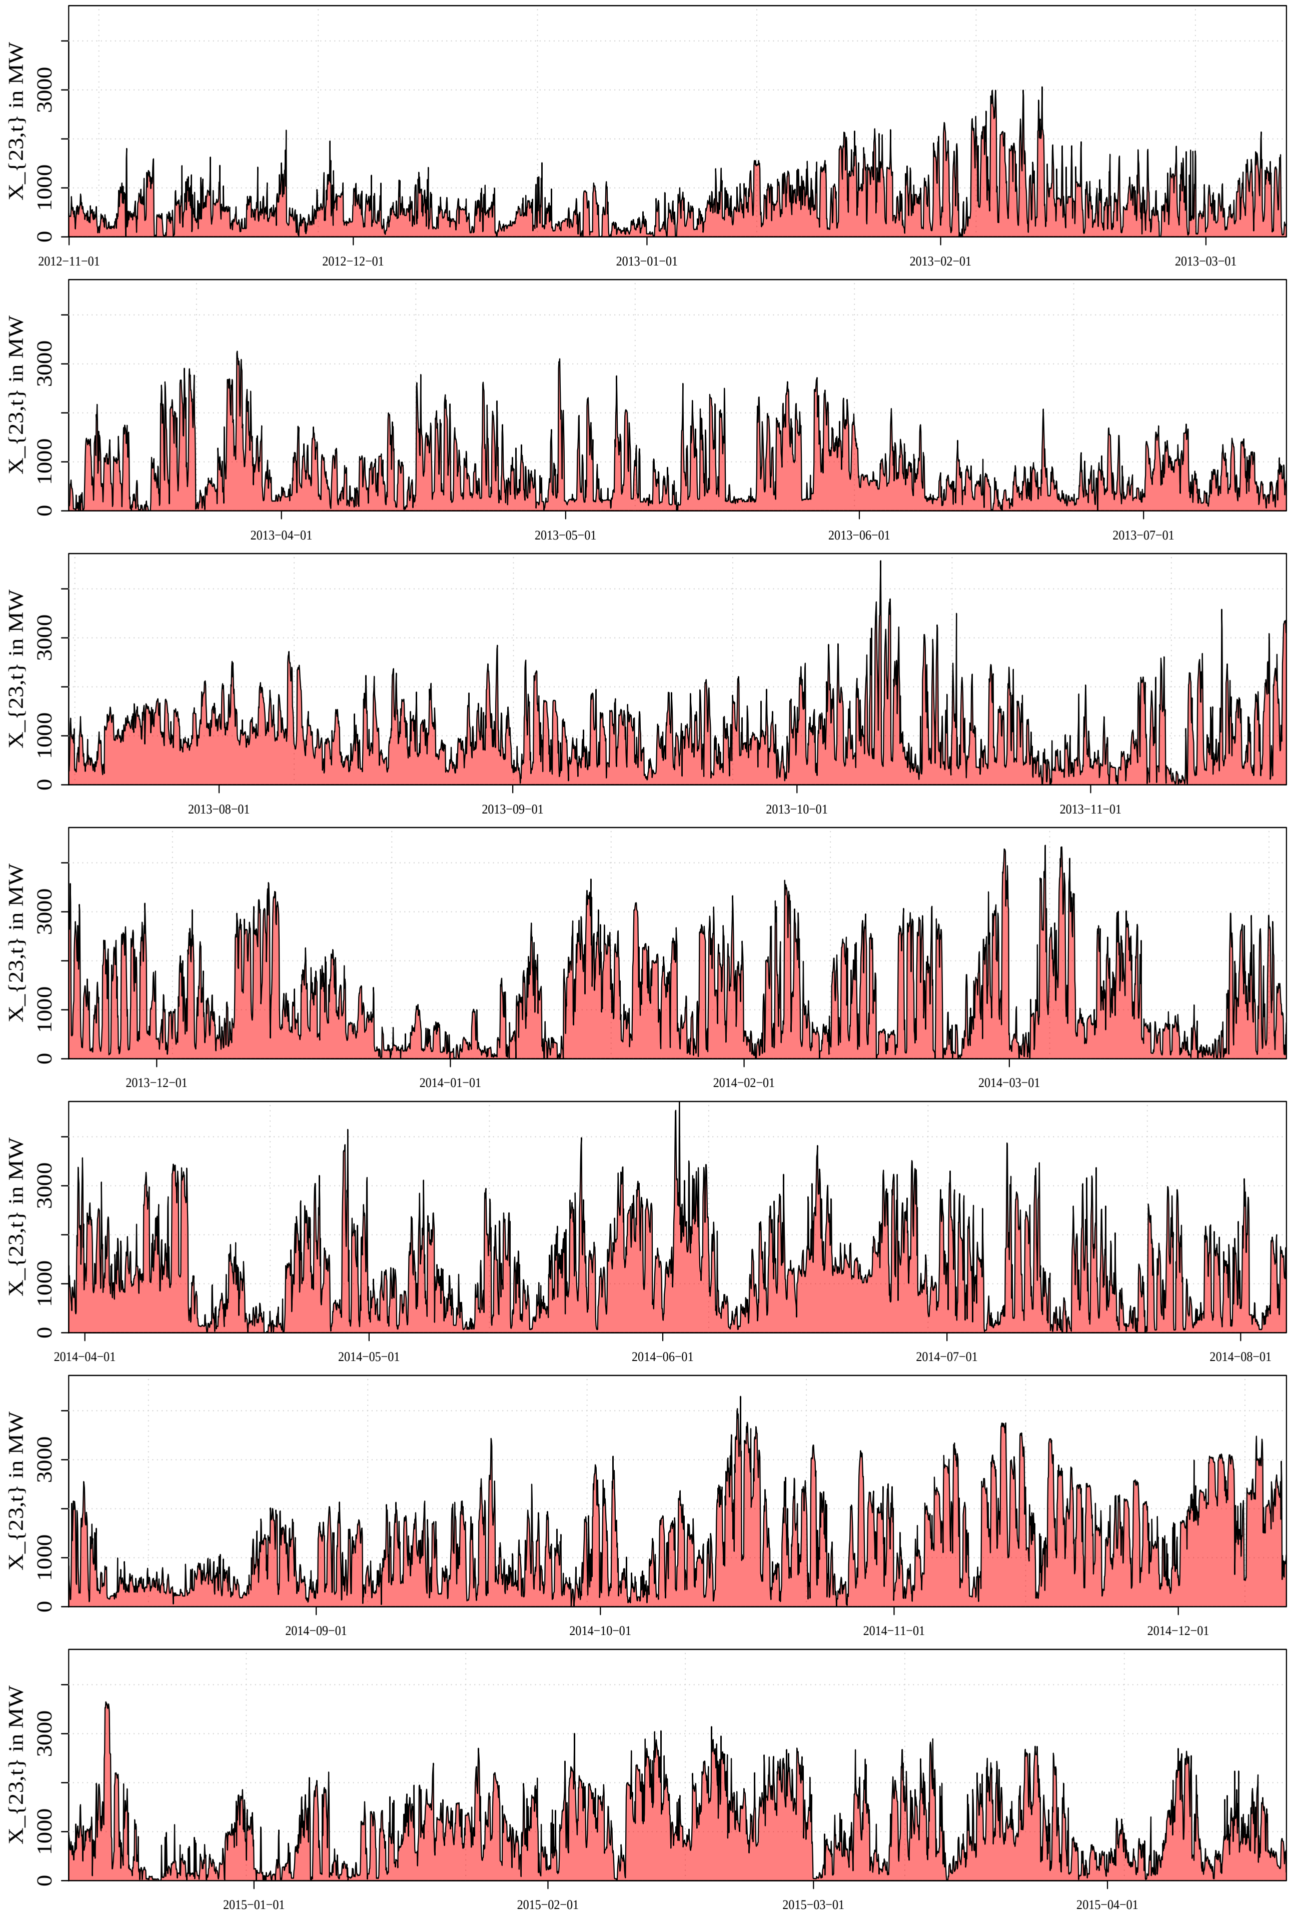


Figure 23: Time series plot of $X_{23,t} = X^{(28.0)}_{D,t}$ with demand/purchase bids on $[28.0, 30.8]$

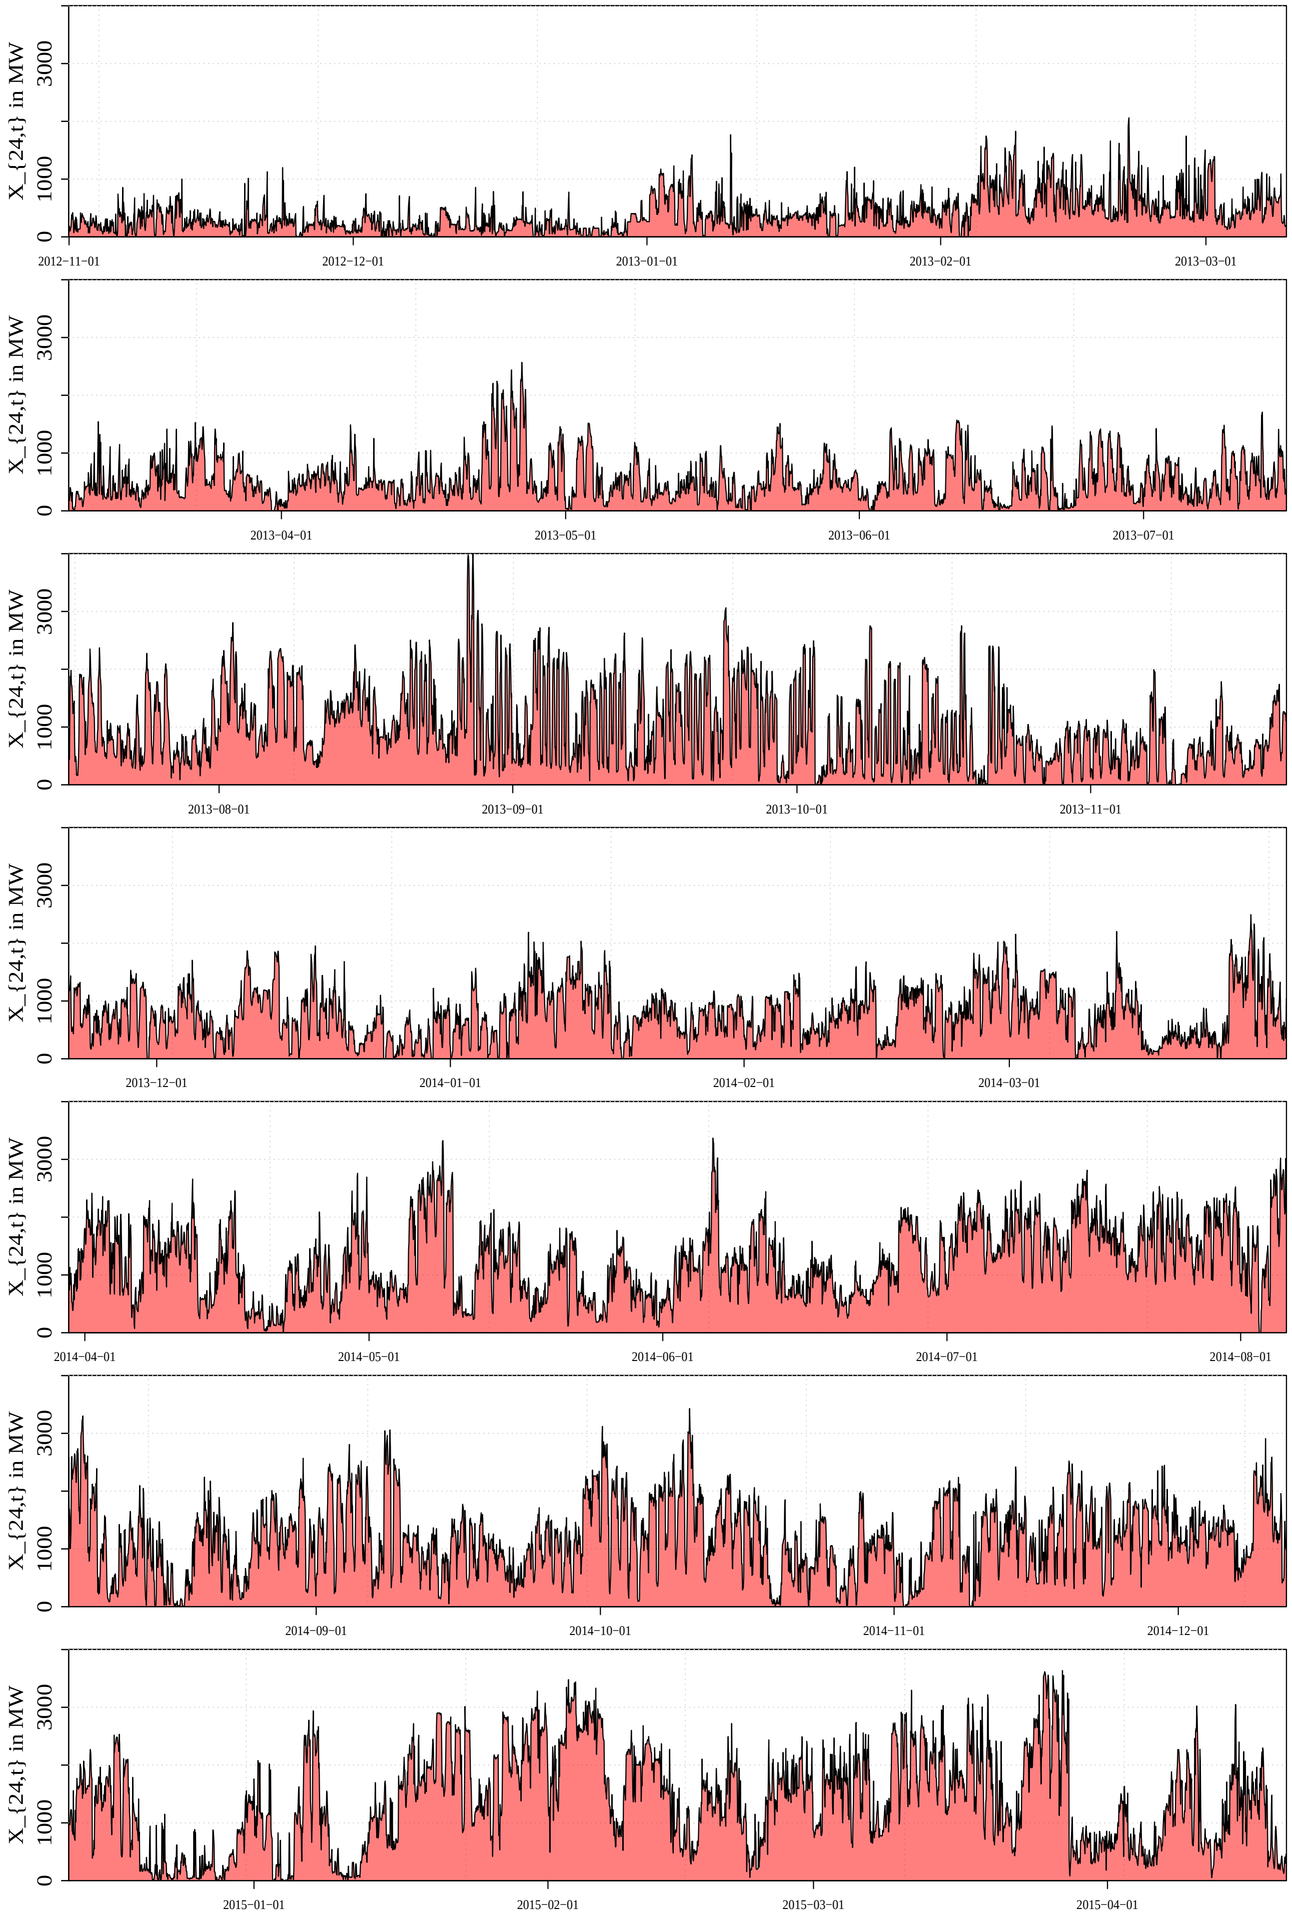


Figure 24: Time series plot of $X_{24,t} = X_{D,t}^{(24.5)}$ with demand/purchase bids on $[24.5, 27.9]$

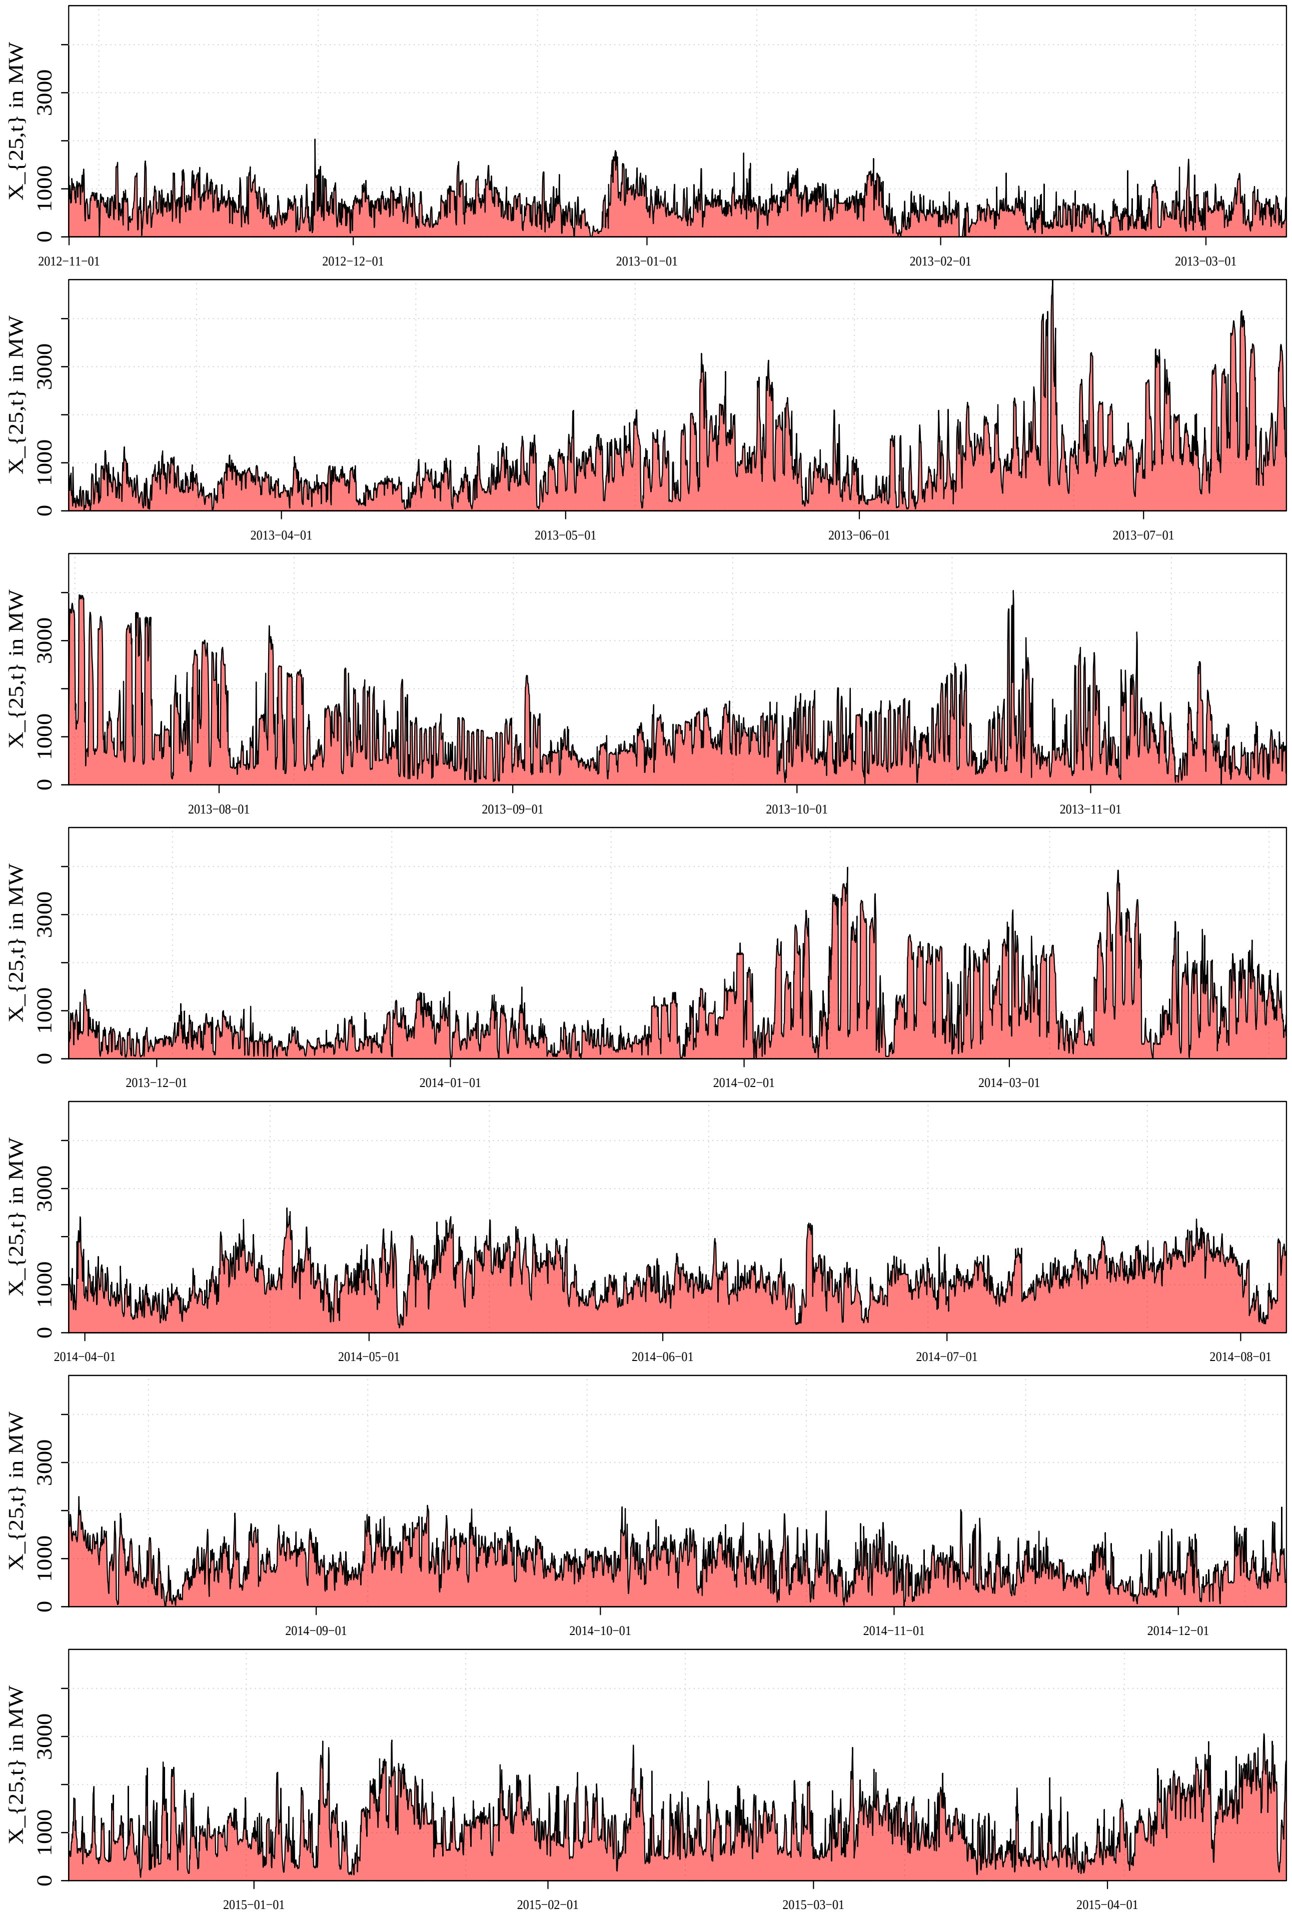


Figure 25: Time series plot of $X_{25,t} = X_{D,t}^{(17.8)}$ with demand/purchase bids on $[17.8, 24.4]$

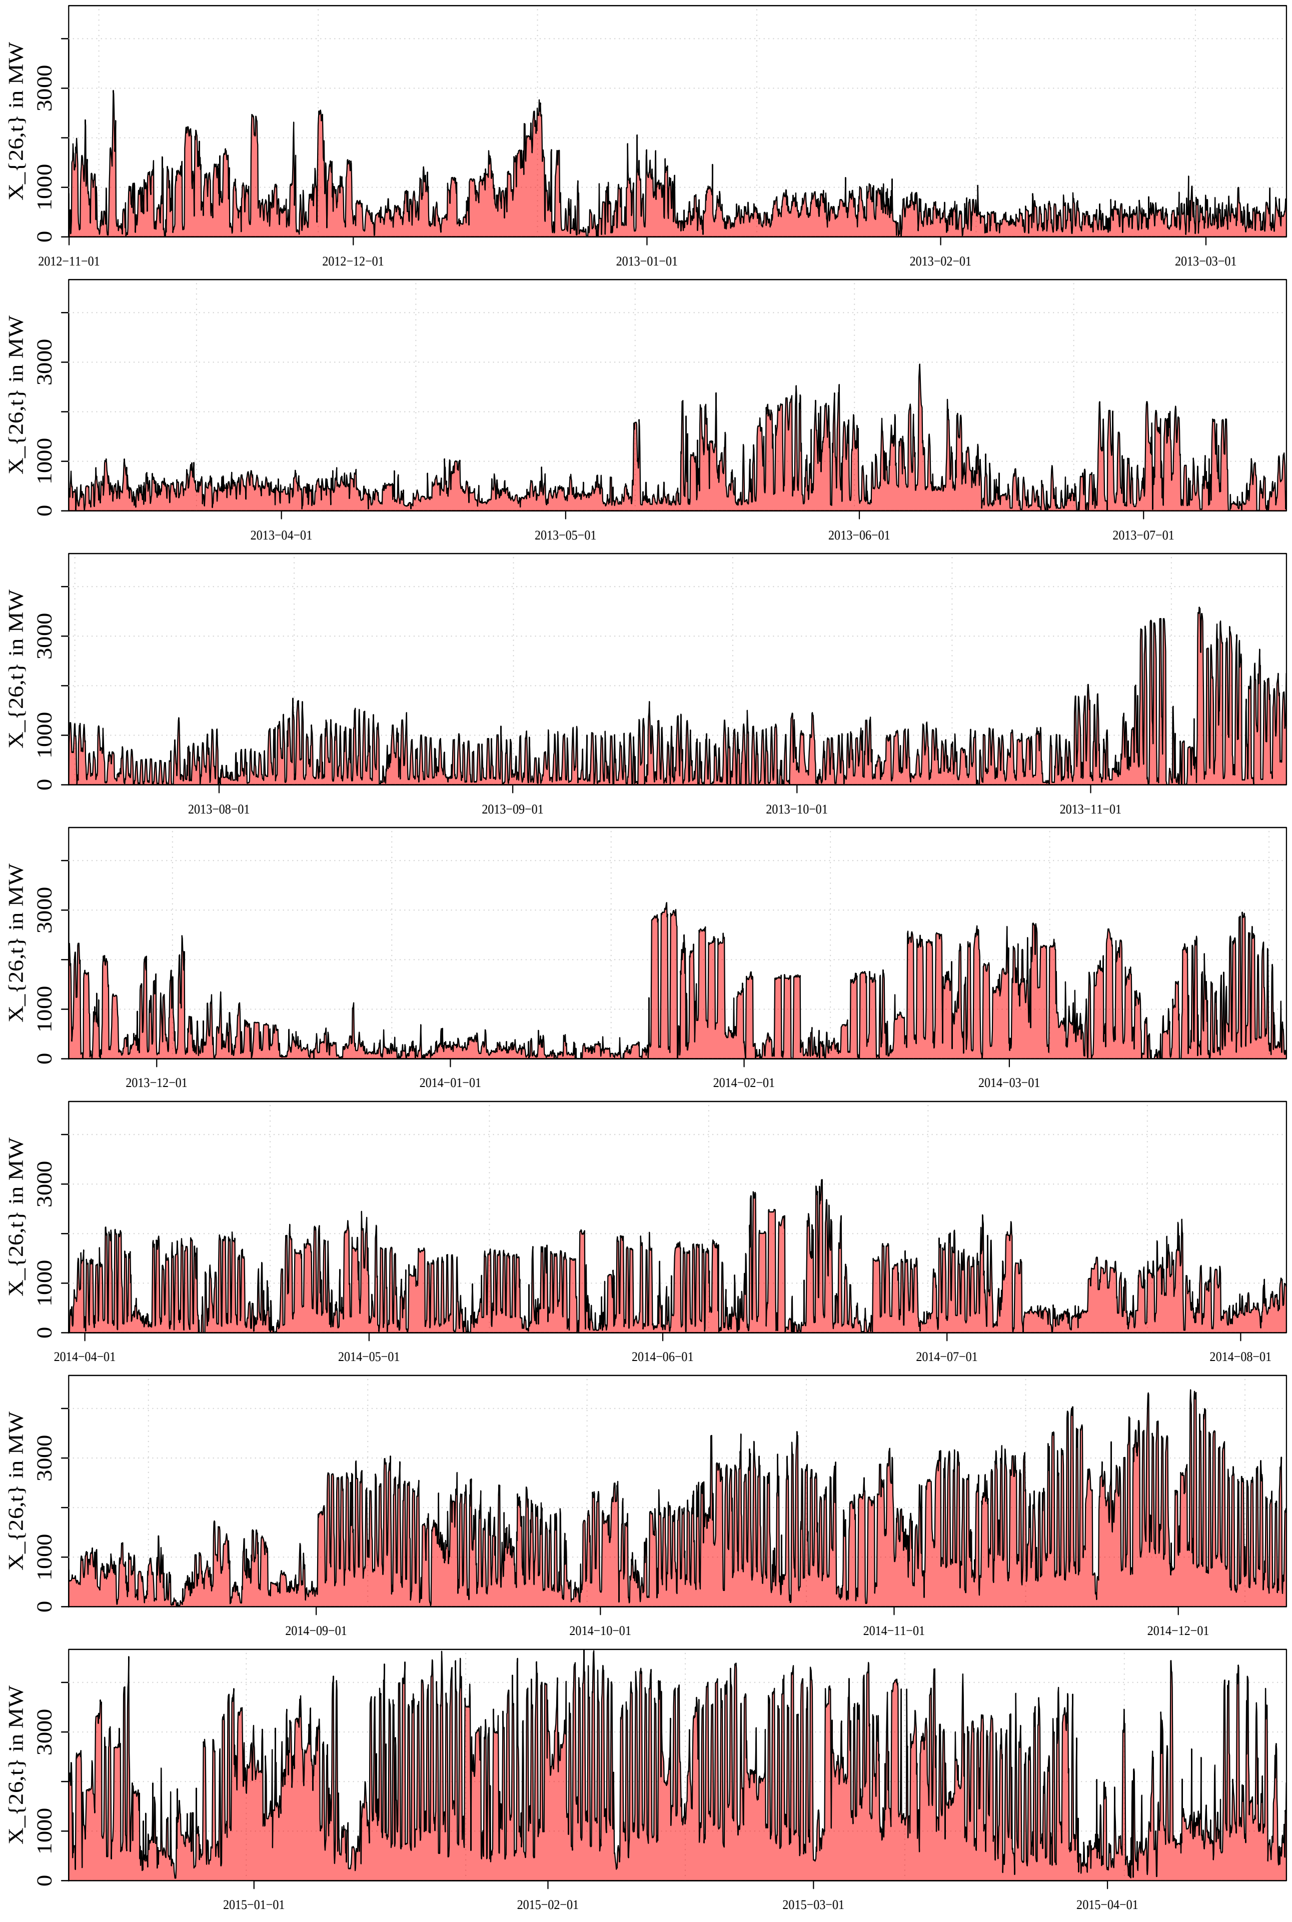


Figure 26: Time series plot of $X_{26,t} = X_{D,t}^{(13.8)}$ with demand/purchase bids on $[13.8, 17.7]$

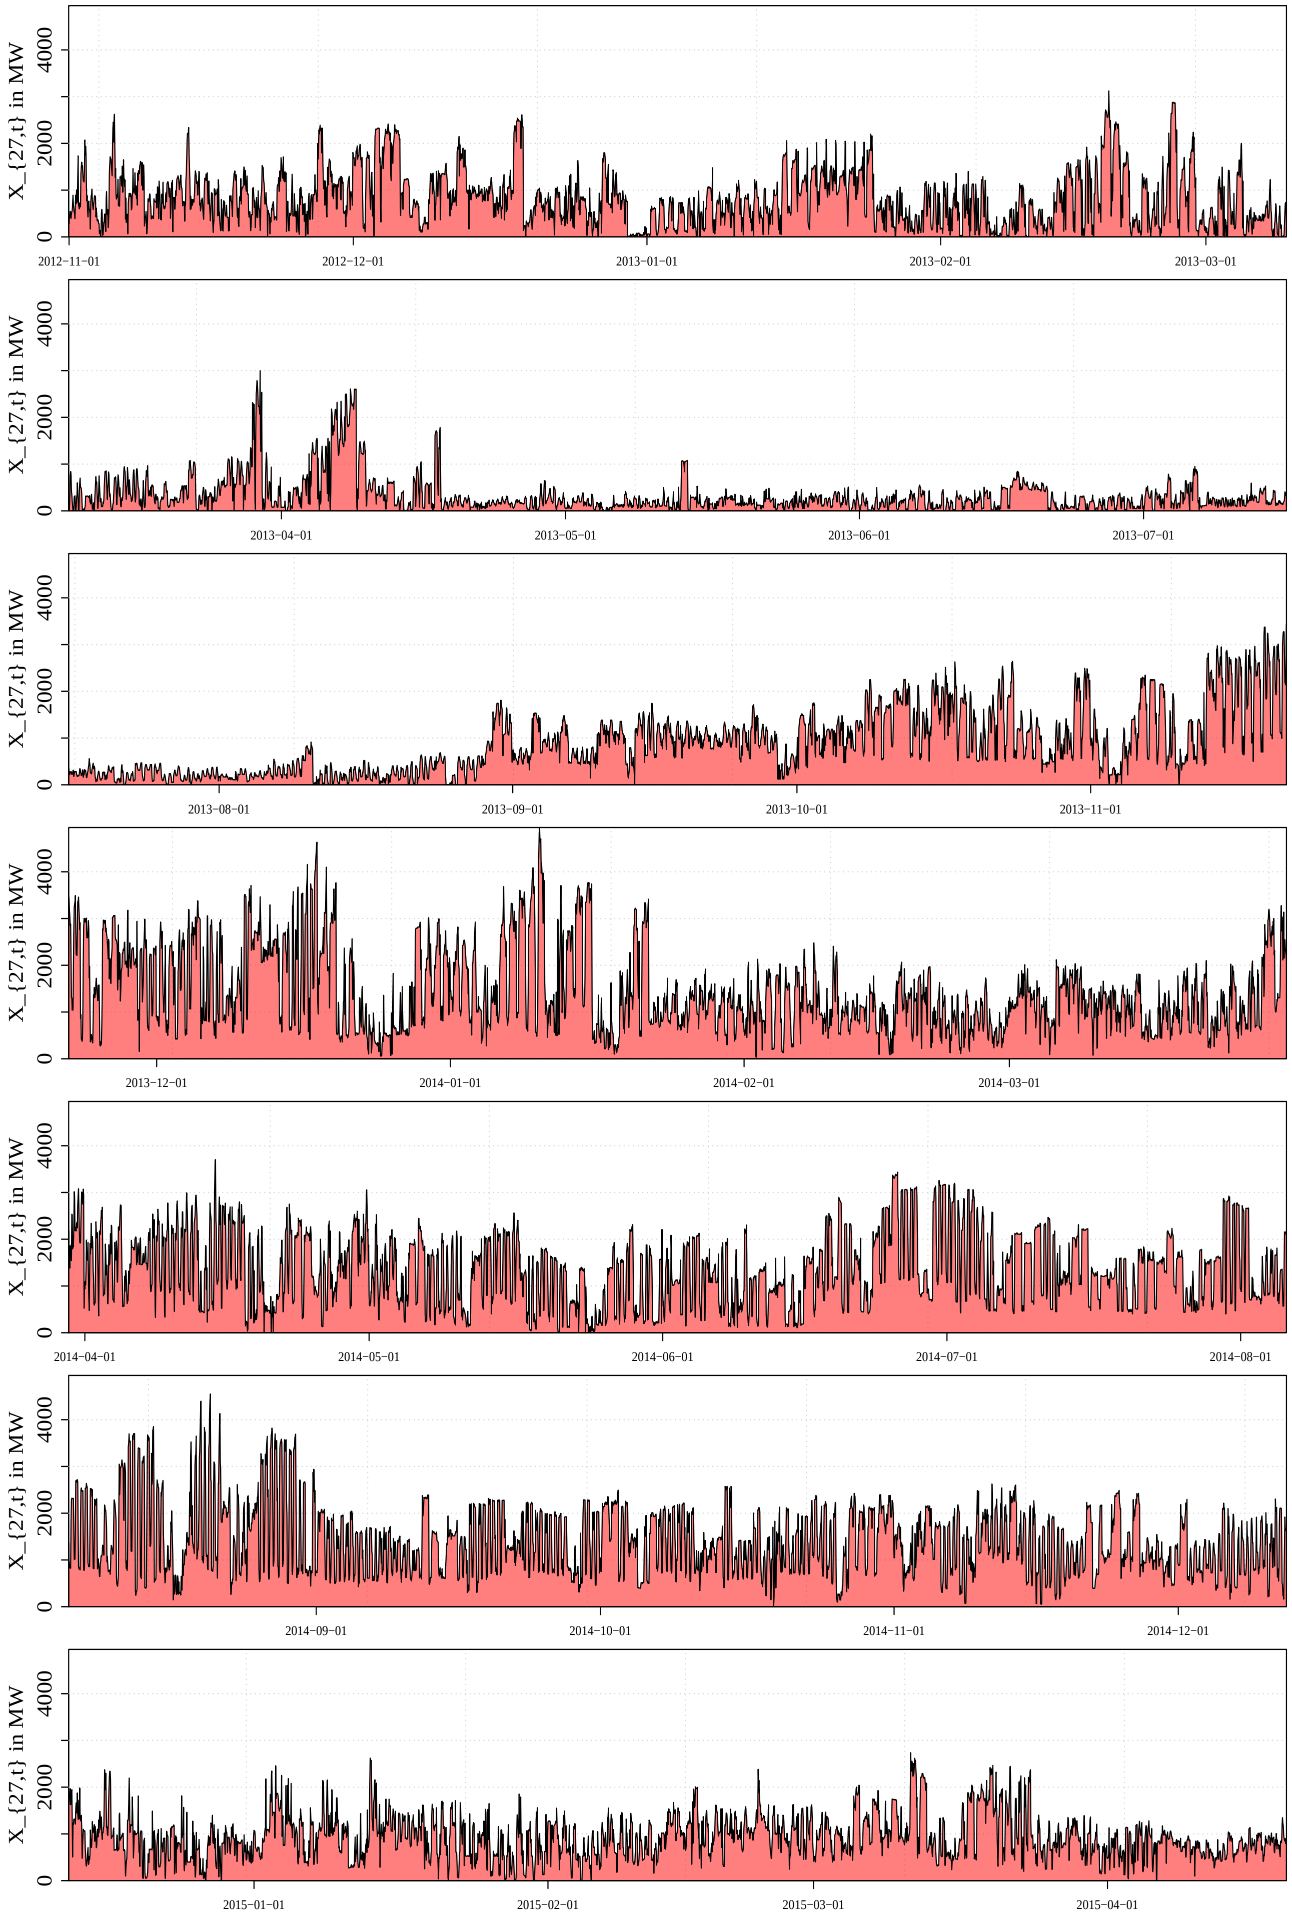


Figure 27: Time series plot of $X_{27,t} = X_{D,t}^{(11.2)}$ with demand/purchase bids on $[11.2, 13.7]$

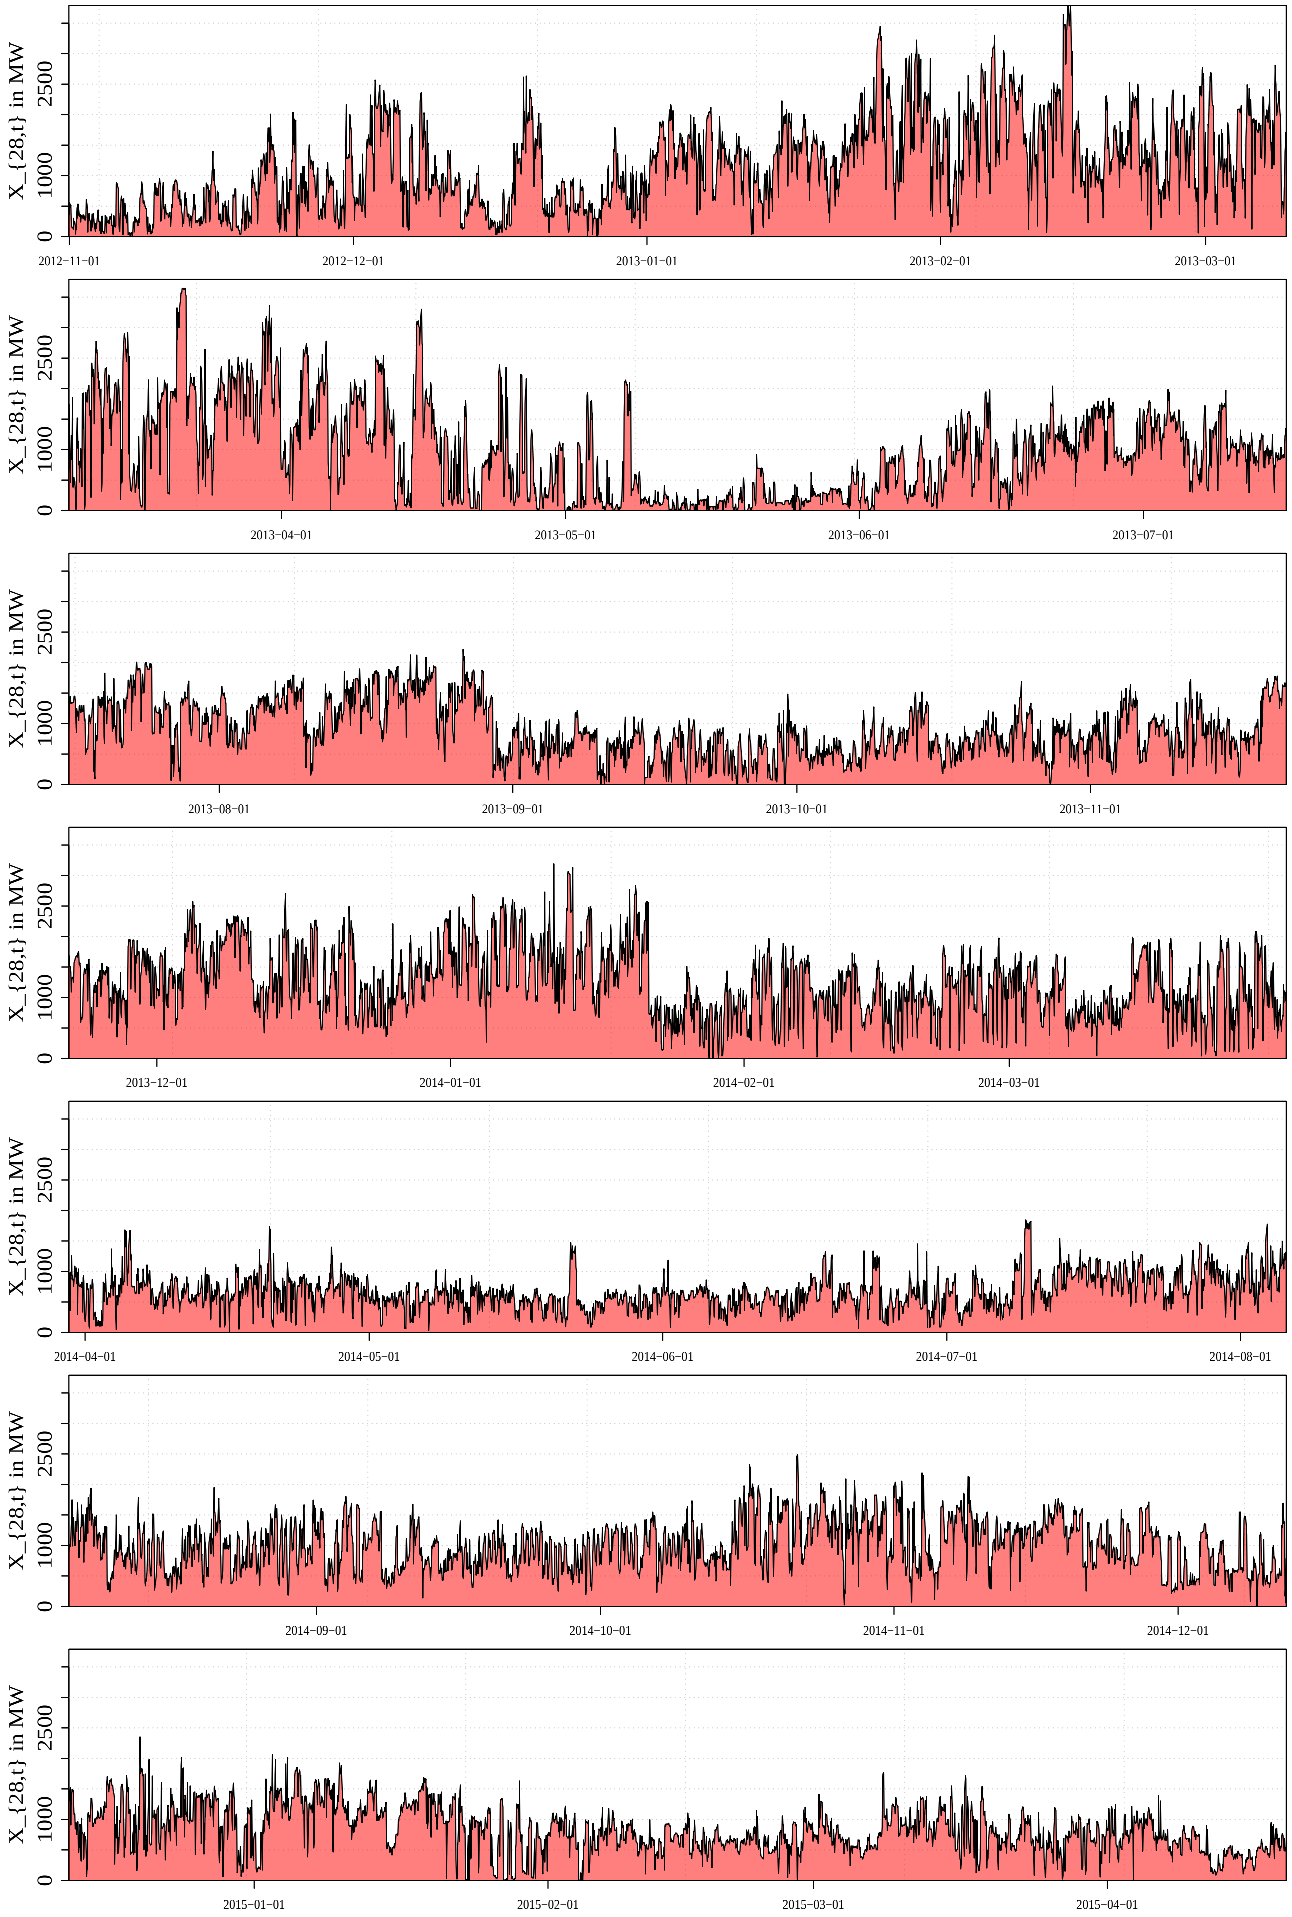


Figure 28: Time series plot of $X_{28,t} = X_{D,t}^{(8.4)}$ with demand/purchase bids on $[8.4, 11.1]$

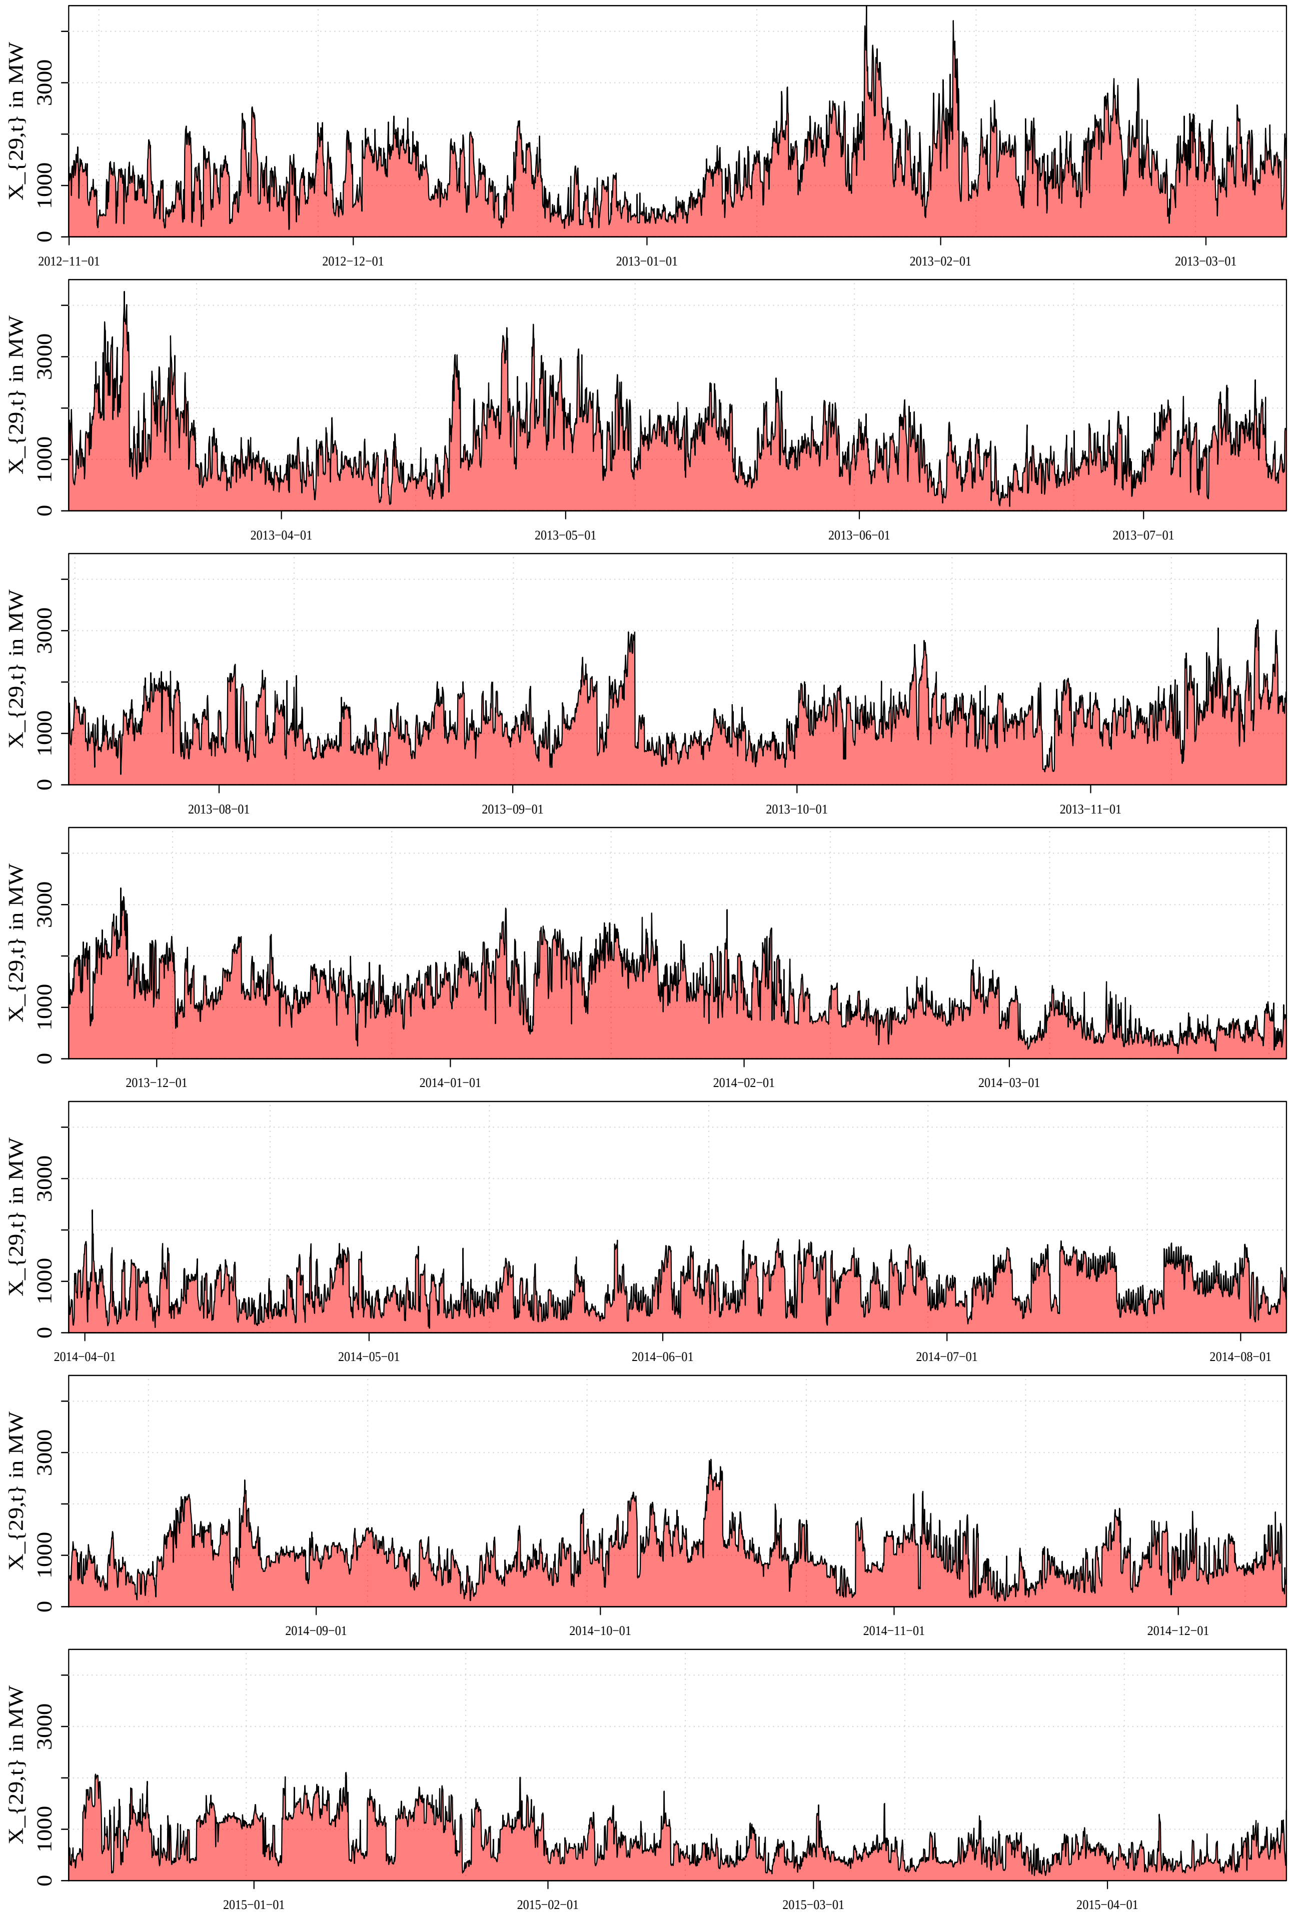


Figure 29: Time series plot of $X_{29,t} = X_{D,t}^{(0.0)}$ with demand/purchase bids on $[0.0, 8.3]$

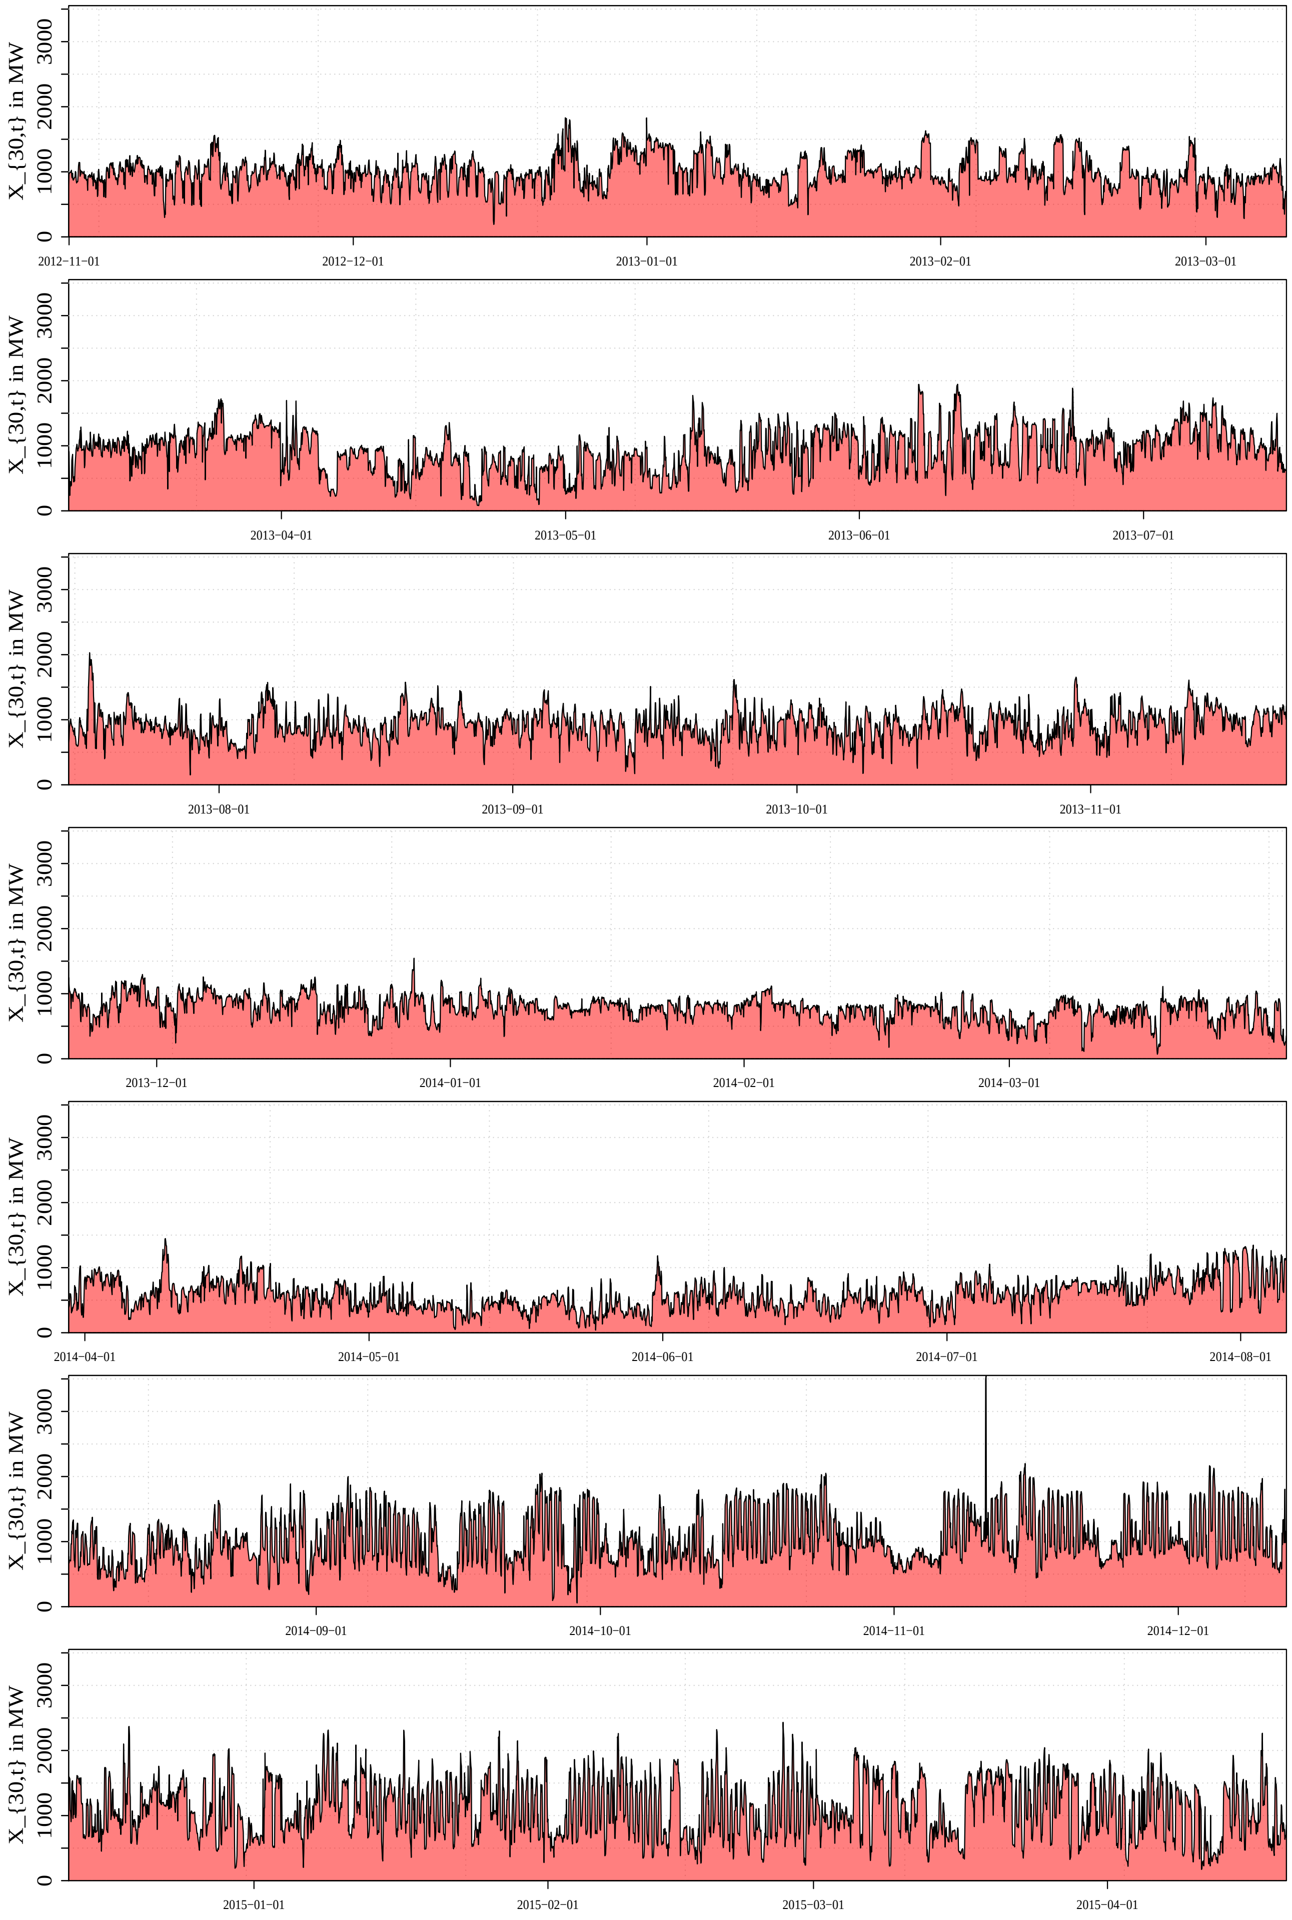


Figure 30: Time series plot of $X_{30,t} = X_{D,t}^{(-10.7)}$ with demand/purchase bids on $[-10.7, -0.1]$

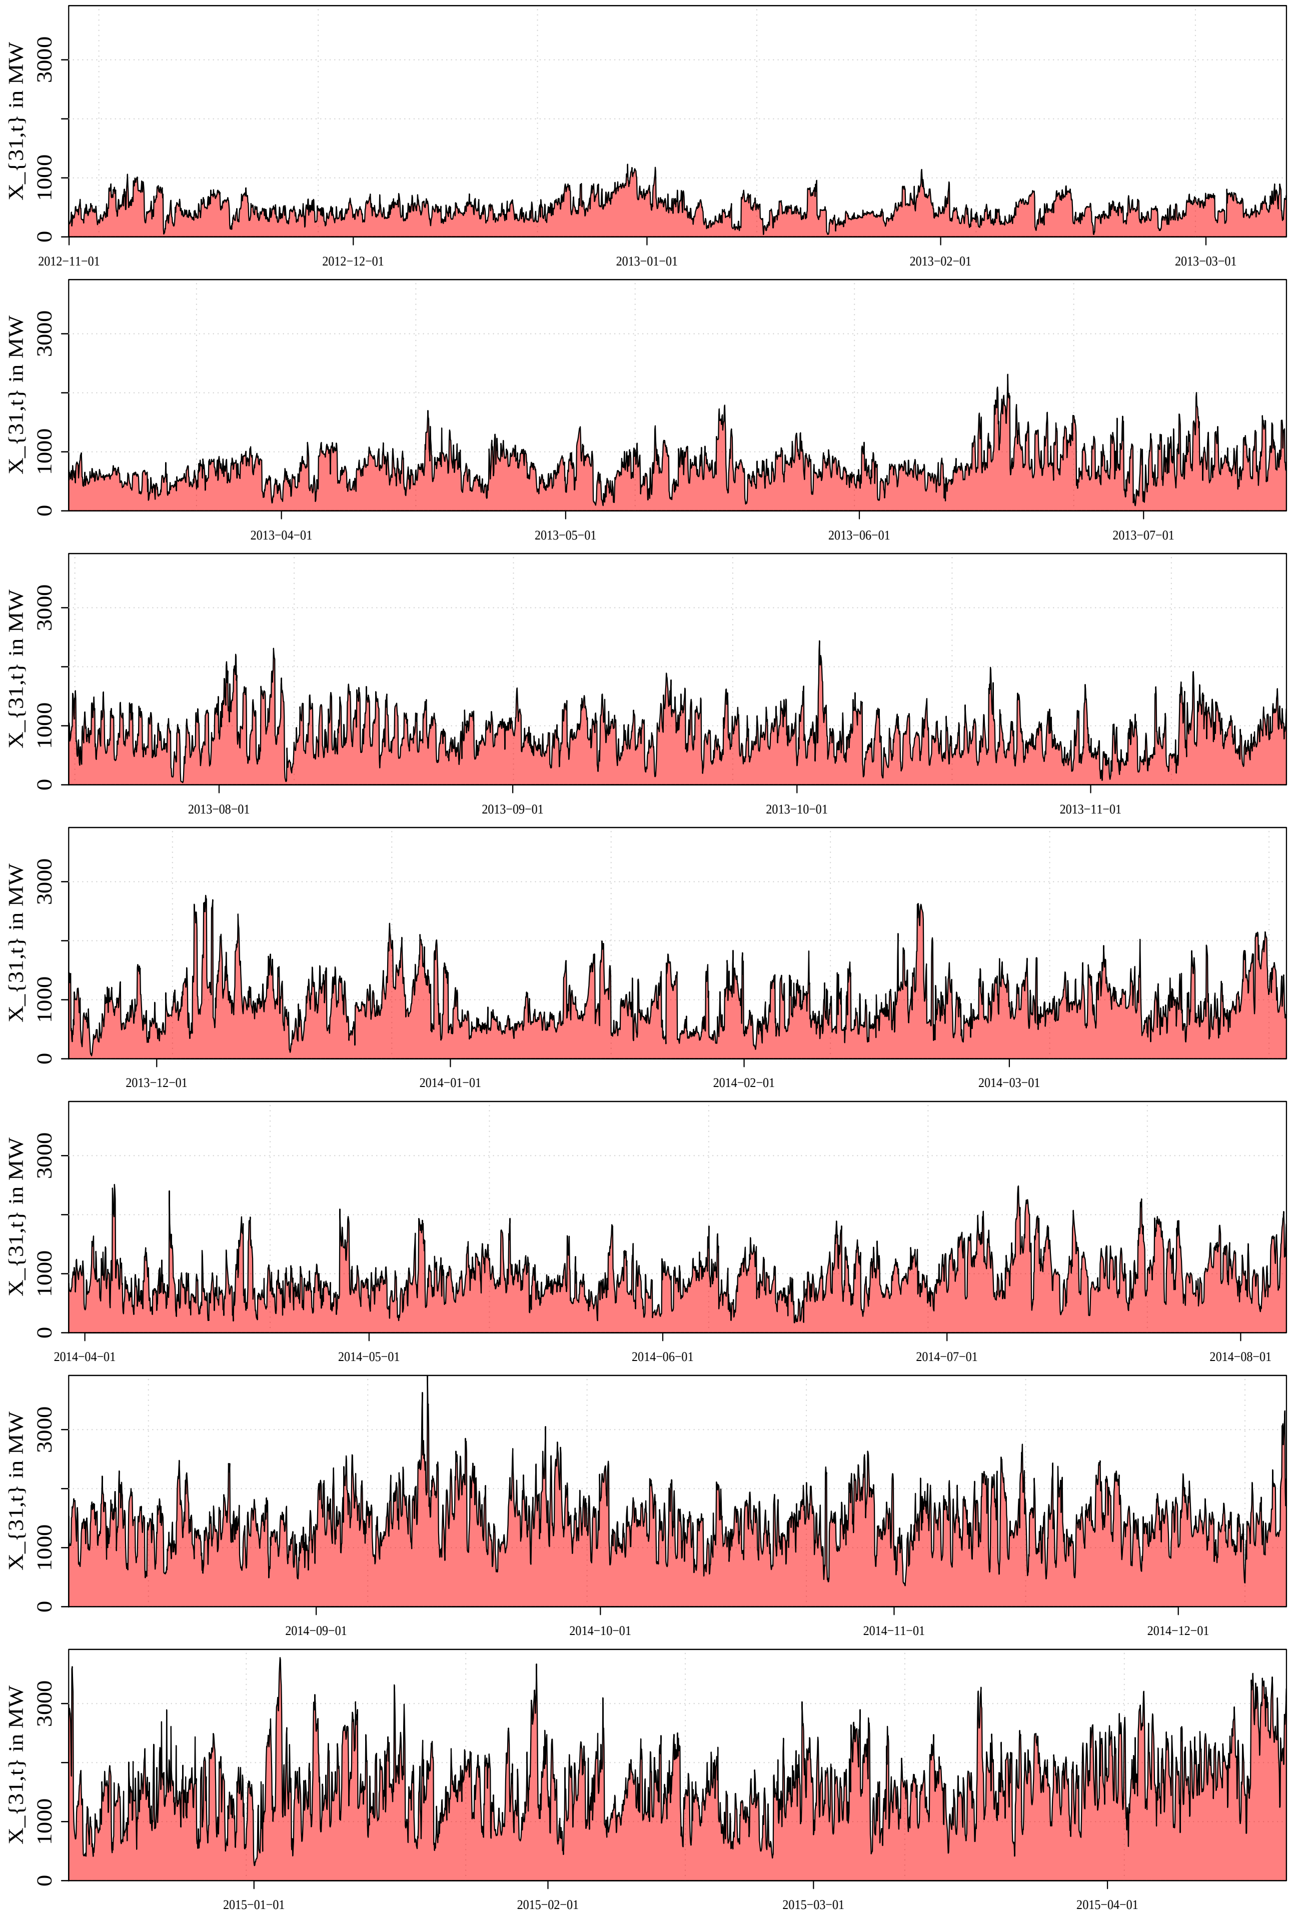


Figure 31: Time series plot of $X_{31,t} = X_{D,t}^{(-200.0)}$ with demand/purchase bids on $[-200.0, -10.8]$

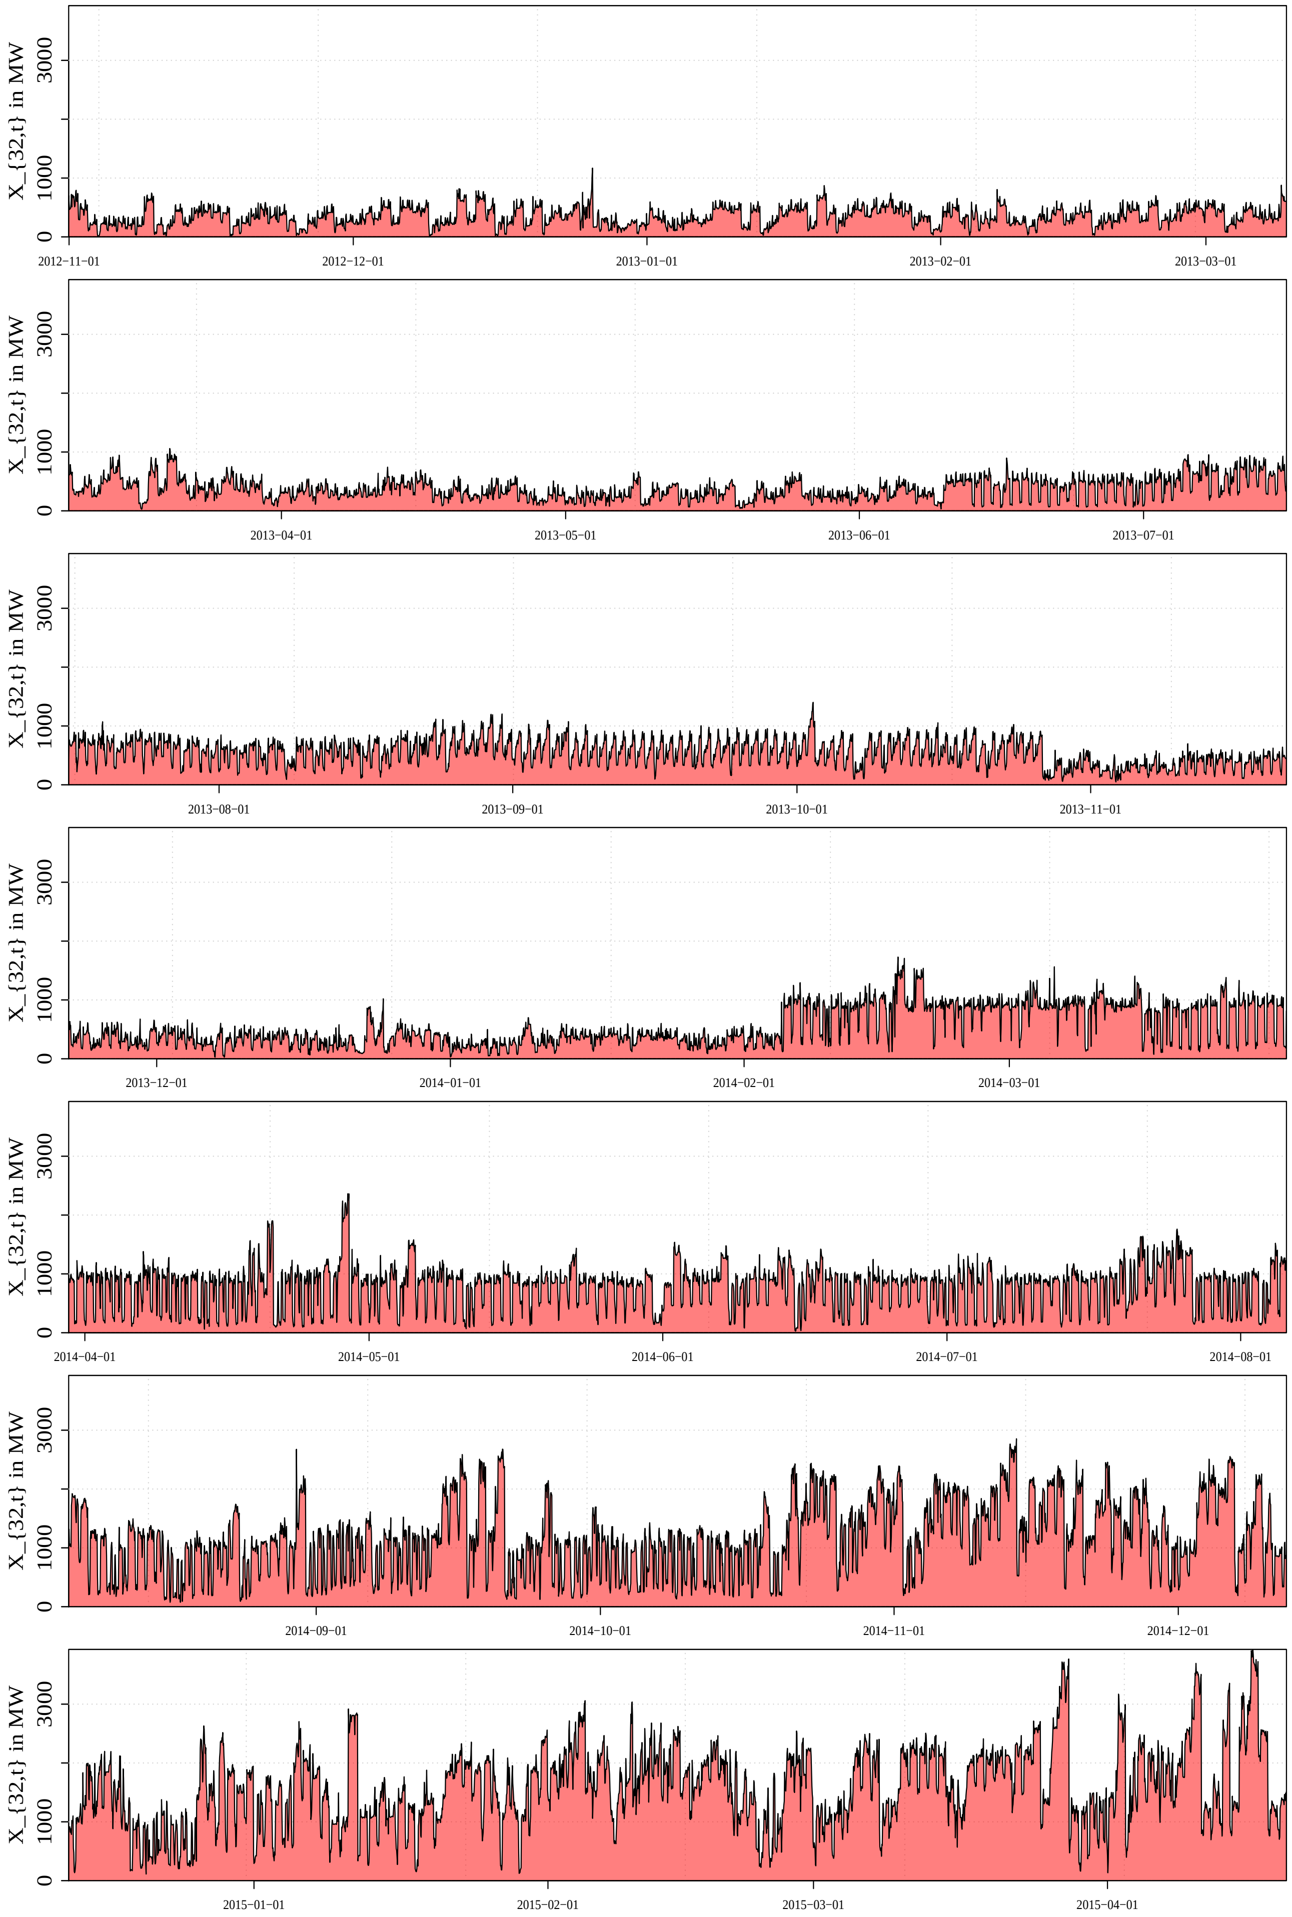


Figure 32: Time series plot of $X_{32,t} = X_{D,t}^{(-500.0)}$ with demand/purchase bids on $[-500.0, -200.1]$

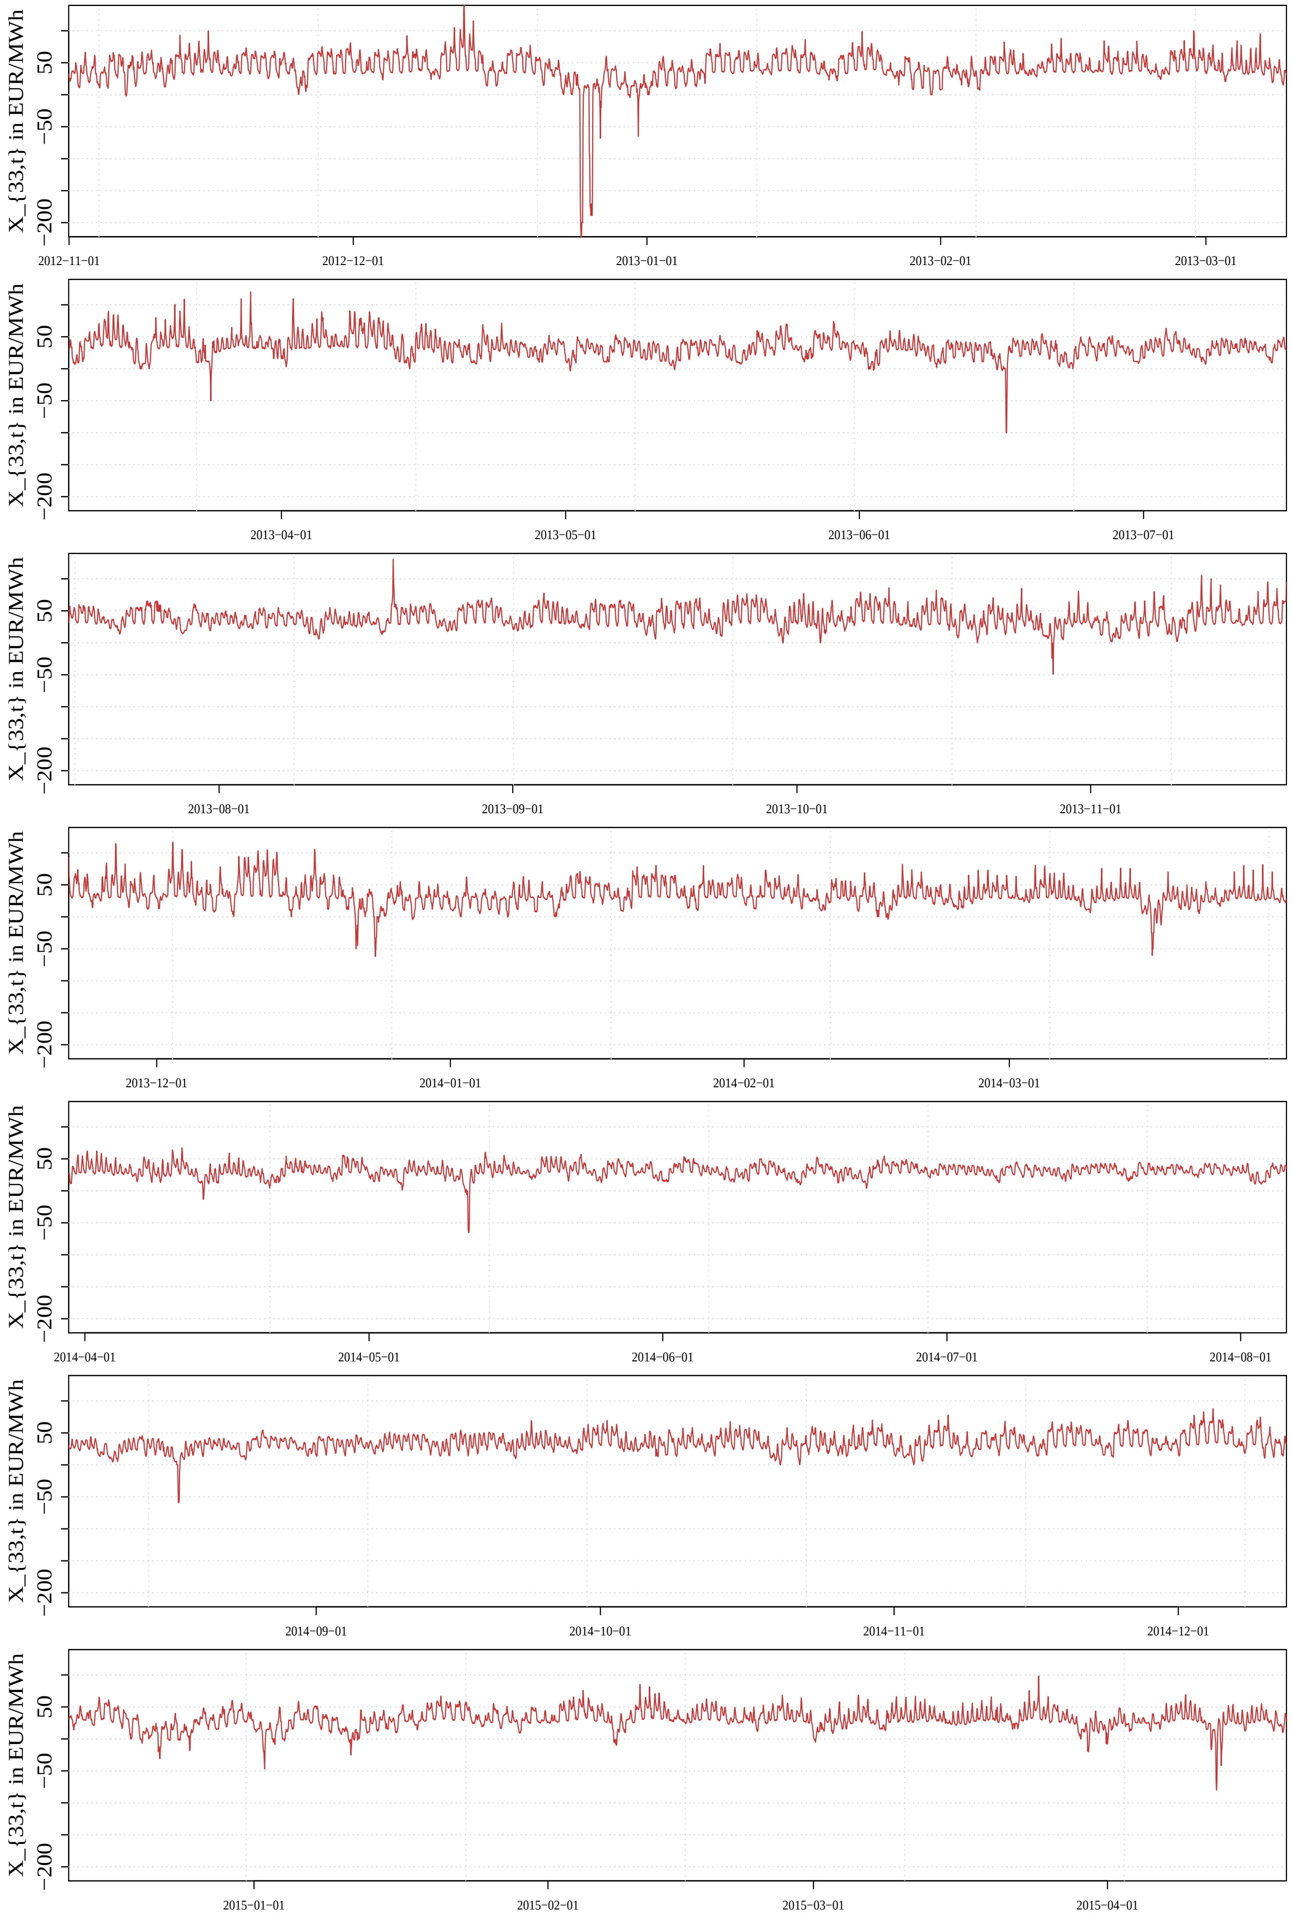


Figure 33: Time series plot of $X_{33,t} = X_{\text{price},t}$ (market clearing price in EUR/MWh)

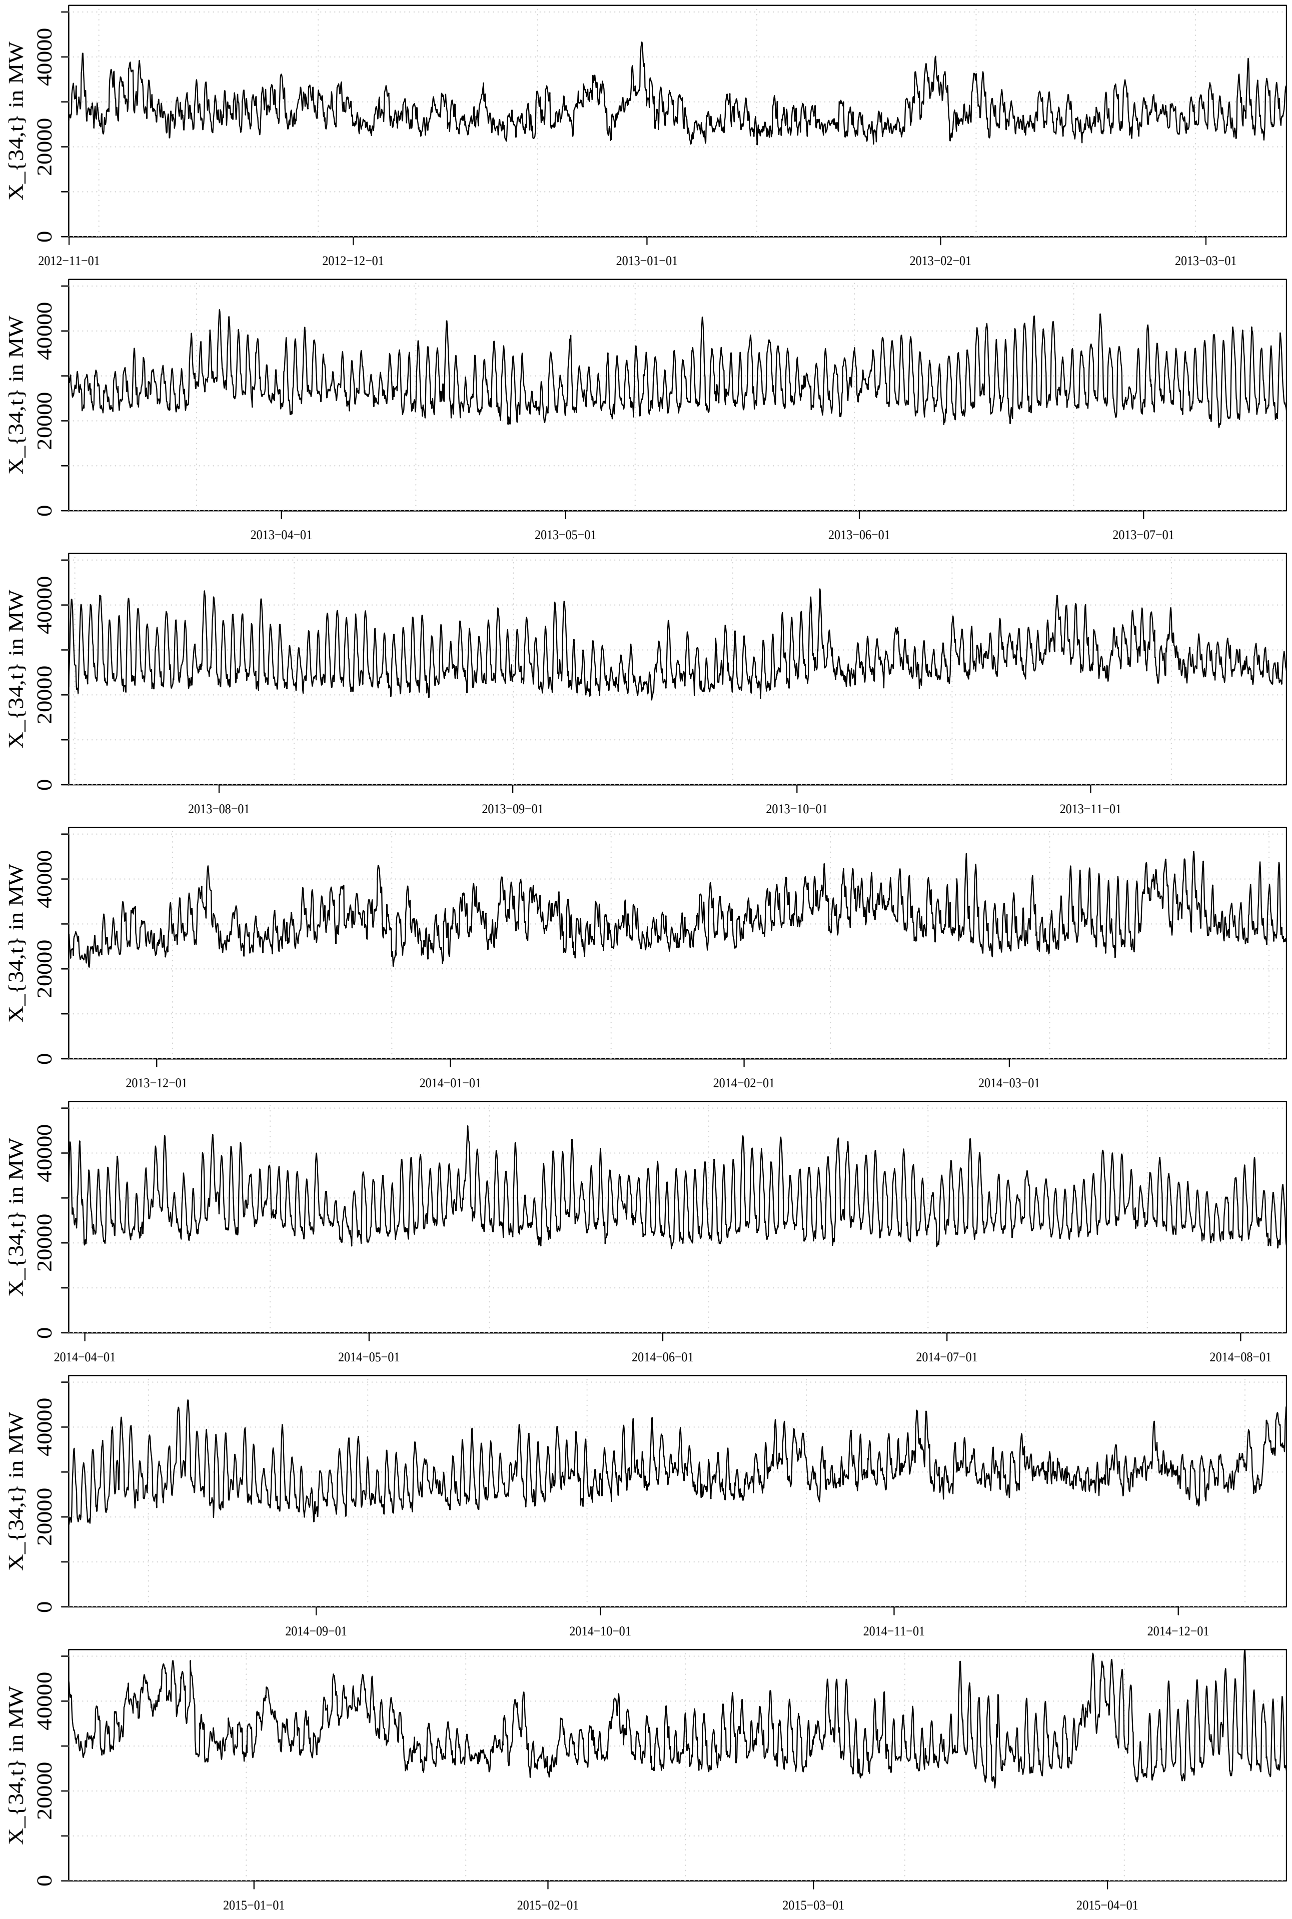


Figure 34: Time series plot of $X_{34,t} = X_{\text{volume},t}$ (market clearing volume)

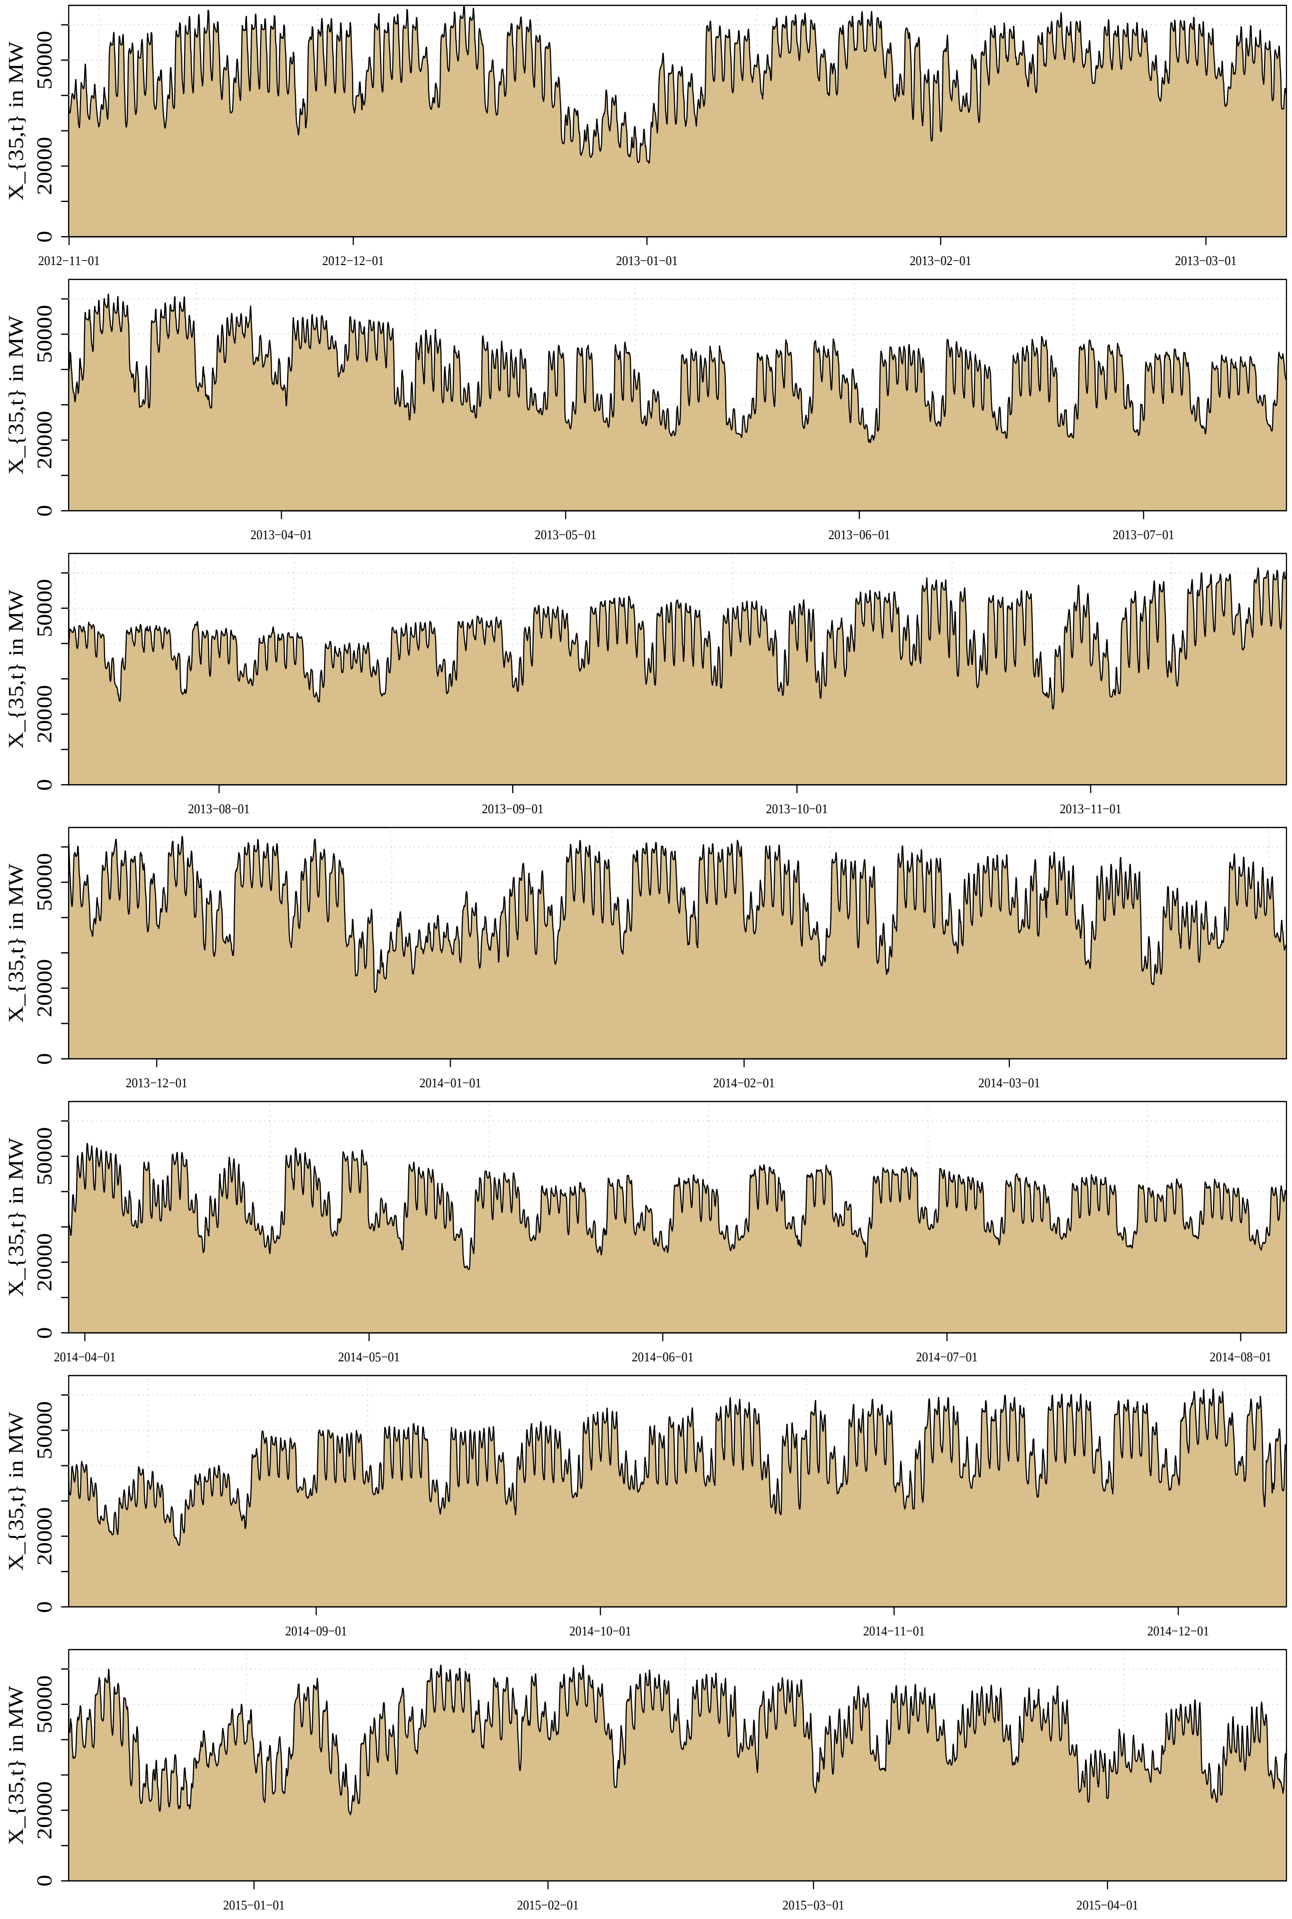


Figure 35: Time series plot of $X_{35,t} = X_{\text{generation},t}$ (planned generation, conv. $\geq$ 100MWh)

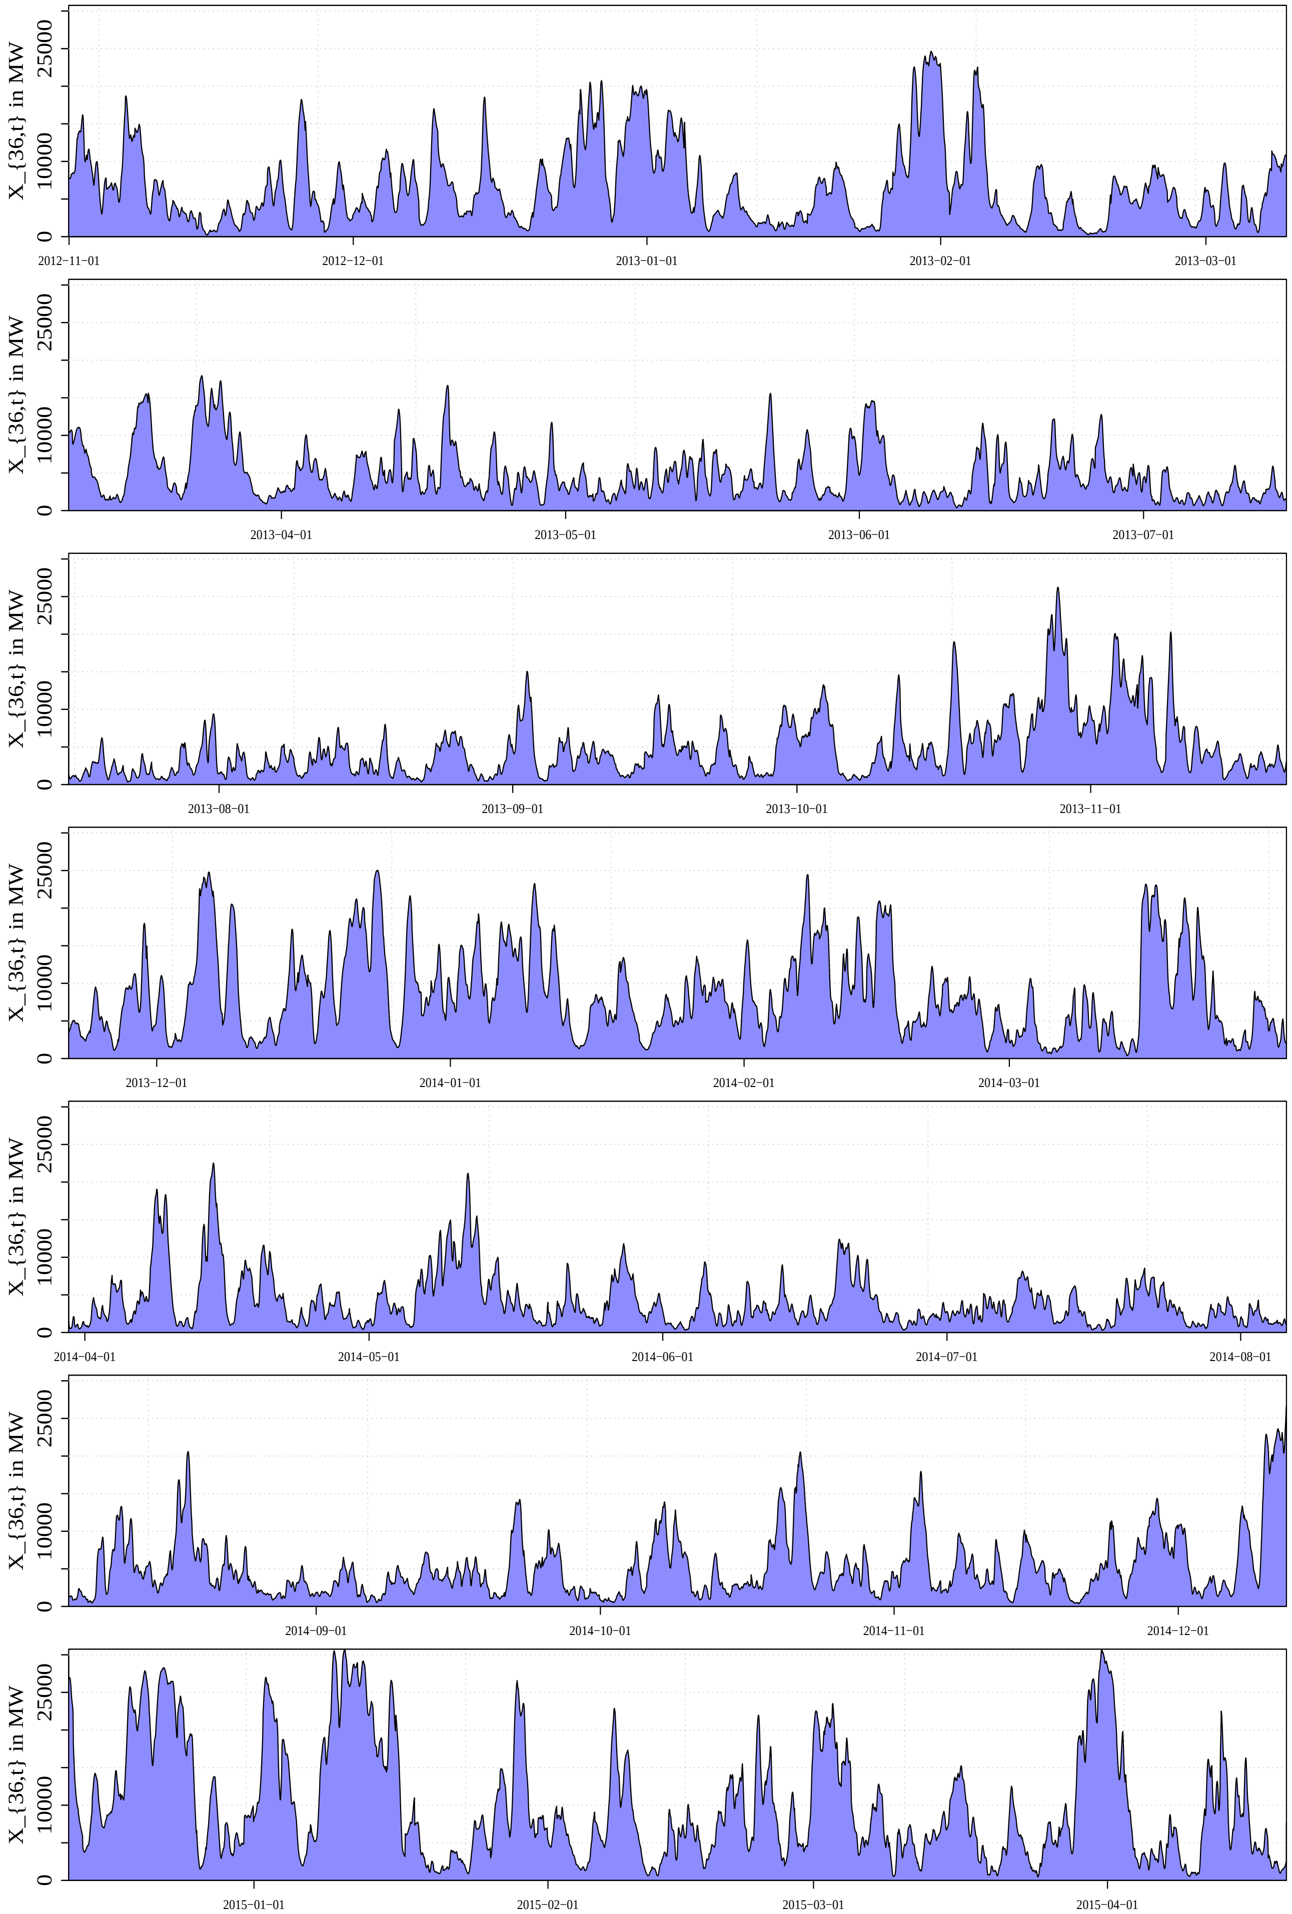


Figure 36: Time series plot of $X_{36,t} = X_{\text{wind},t}$ (planned wind generation)

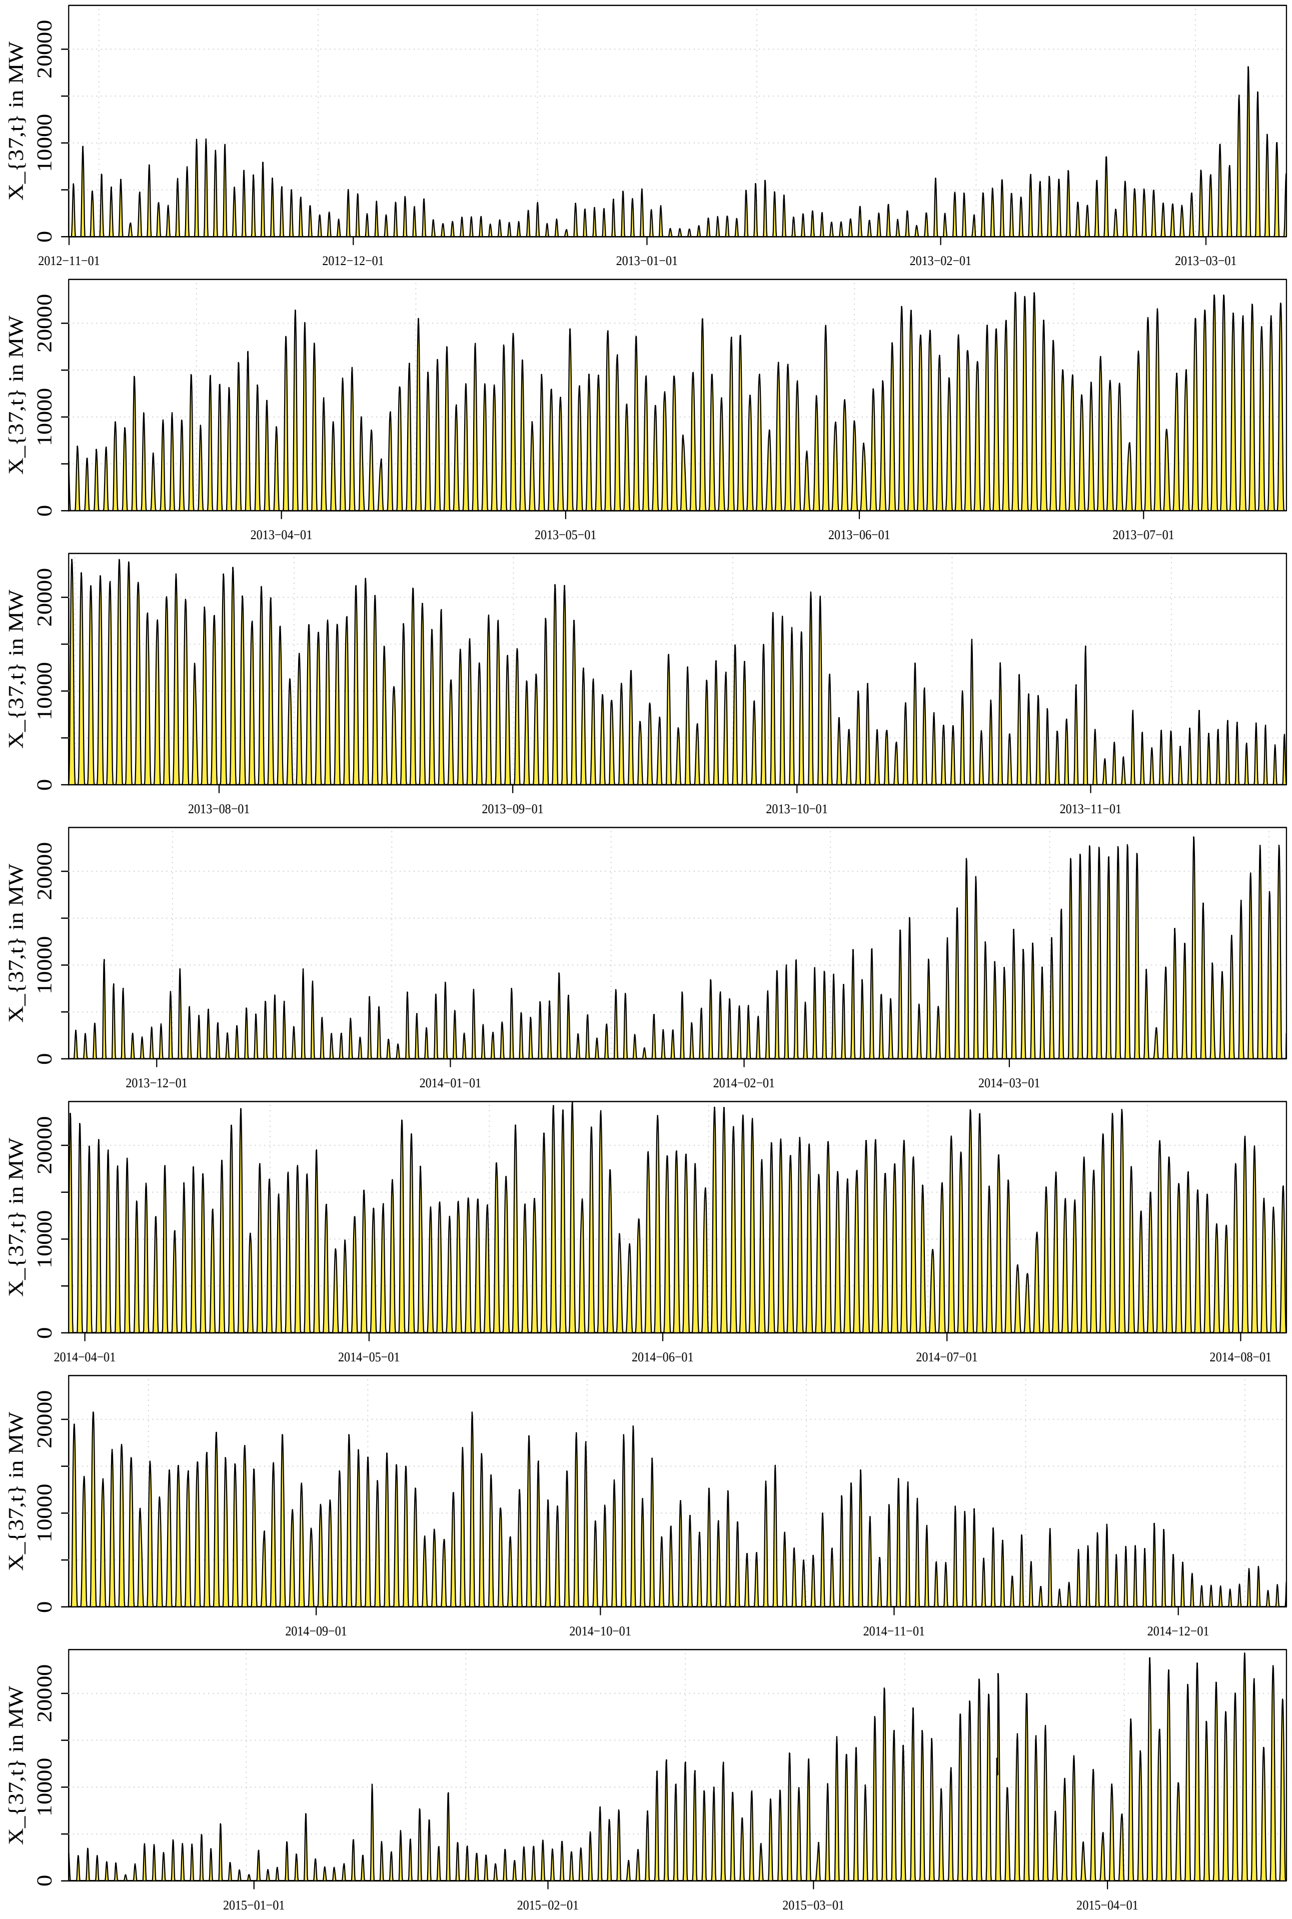


Figure 37: Time series plot of $X_{37,t} = X_{\text{solar},t}$ (planned solar generation)
